# Supplementary material for: Poincare function for moduli of differential-geometric structures
Source: arXiv:1802.01322 source file (2018-02-05)
Supplement: Supplementary file 1 [file 3-forms_orthogonal_stabilizers.pdf]

```

> with(DifferentialGeometry) : with(Tensor) : with(Tools) : Preferences("ShowFramePrompt",
  'false') :
> DGsetup([seq(x||i, i=1..9)], M9) :
> O3 := evalDG(dx1 &w dx2 &w dx3 + dx3 &w dx4 &w dx5 + dx5 &w dx6 &w dx7 + dx7
  &w dx8 &w dx9 + dx1 &w dx5 &w dx9)
O3 := (dx1 ∧ dx2) ∧ dx3 + (dx1 ∧ dx5) ∧ dx9 + (dx3 ∧ dx4) ∧ dx5
  + (dx5 ∧ dx6) ∧ dx7 + (dx7 ∧ dx8) ∧ dx9

```

(1)

```

> V := evalDG(add(add((a||i)||j·(x||j·D_x||i - x||i·D_x||j), j=i+1..9), i=1..9)):
> DGsimplify(subs(solve(DGinfo(LieDerivative(V, O3), "CoefficientSet"), V))
  0 D_x1

```

(2)

```

> n := 4 : DGsetup([seq(x||i, i=1..n)], M||n) :
O3 := evalDG(add(add(add(RandomTools[Generate](integer(range=0..9))·dx||i &w dx
  ||j &w dx||k, k=j+1..n), j=i+1..n), i=1..n));
V := evalDG(add(add((a||i)||j·(x||j·D_x||i - x||i·D_x||j), j=i+1..n), i=1..n)):
slv := solve(DGinfo(LieDerivative(V, O3), "CoefficientSet"), {seq(seq((a||i)||j, j=i+1
  ..n), i=1..n)});
tmp := 0 :for i to nops(slv) do if lhs(slv[i]) = rhs(slv[i]) then tmp := tmp + 1 :fi:od:
[nops(slv), binomial(n, 2), tmp];
DGsimplify(subs(slv, V)) :
O3 := ((6 dx1) ∧ dx2) ∧ dx3 + ((8 dx1) ∧ dx3) ∧ dx4 + ((9 dx2) ∧ dx3) ∧ dx4
slv := {a12 = a12, a13 = a13, a14 = -4/3 a12, a23 = a23, a24 = -3/2 a12, a34 = 4/3 a23
  - 3/2 a13}

```

[6, 6, 3] (3)

```

> n := 5 : DGsetup([seq(x||i, i=1..n)], M||n) :
O3 := evalDG(add(add(add(RandomTools[Generate](integer(range=0..9))·dx||i &w dx
  ||j &w dx||k, k=j+1..n), j=i+1..n), i=1..n));
V := evalDG(add(add((a||i)||j·(x||j·D_x||i - x||i·D_x||j), j=i+1..n), i=1..n)):
slv := solve(DGinfo(LieDerivative(V, O3), "CoefficientSet"), {seq(seq((a||i)||j, j=i+1
  ..n), i=1..n)});
tmp := 0 :for i to nops(slv) do if lhs(slv[i]) = rhs(slv[i]) then tmp := tmp + 1 :fi:od:
[nops(slv), binomial(n, 2), tmp];
DGsimplify(subs(slv, V)) :
O3 := ((9 dx1) ∧ dx2) ∧ dx3 + ((8 dx1) ∧ dx2) ∧ dx4 + ((6 dx1) ∧ dx2) ∧ dx5
  + ((7 dx1) ∧ dx3) ∧ dx5 + ((4 dx1) ∧ dx4) ∧ dx5 + ((7 dx2) ∧ dx3) ∧ dx4
  + ((7 dx2) ∧ dx3) ∧ dx5 + ((9 dx2) ∧ dx4) ∧ dx5 + ((6 dx3) ∧ dx4) ∧ dx5
slv := {a12 = a12, a13 = 847/4010 a12 - 10293/4010 a23, a14 = -4641/4010 a12 + 13979/4010 a23, a15
  = -445/802 a23 - 639/802 a12, a23 = a23, a24 = -195/802 a12 - 1111/802 a23, a25 =
  -610/401 a12 + 915/401 a23, a34 = -127/2005 a12 + 3198/2005 a23, a35 = 1182/2005 a12
  - 5783/2005 a23, a45 = 1333/4010 a12 + 7023/4010 a23}

```

[10, 10, 2] (4)

```

> n := 5 : DGsetup([seq(x||i, i=1..n)], M||n) :
O3 := evalDG(dx1 &w dx2 &w dx5 + dx3 &w dx4 &w dx5);
V := evalDG(add(add((a||i)||j·(x||j·D_x||i - x||i·D_x||j), j=i+1..n), i=1..n)):

```

```

slv := solve(DGinfo(LieDerivative(V, O3), "CoefficientSet"), {seq(seq((a || i) || j, j = i + 1 .. n), i = 1 .. n)});
tmp := 0 :for i to nops(slv) do if lhs(slv[i]) = rhs(slv[i]) then tmp := tmp + 1 :fi:od:
[nops(slv), binomial(n, 2), tmp];
DGsimplify(subs(slv, V)) :
O3 := (dx1 ^ dx2) ^ dx5 + (dx3 ^ dx4) ^ dx5
slv := {a12 = a12, a13 = a24, a14 = -a23, a15 = 0, a23 = a23, a24 = a24, a25 = 0, a34
= a34, a35 = 0, a45 = 0}
[10, 10, 4]

```

```

> n := 6 : DGsetup([seq(x || i, i = 1 .. n)], M || n) :
O3 := evalDG(add(add(add(RandomTools[Generate](integer(range = 0 .. 9)) · dx || i &w dx
|| j &w dx || k, k = j + 1 .. n), j = i + 1 .. n), i = 1 .. n));
V := evalDG(add(add((a || i) || j · (x || j · D_x || i - x || i · D_x || j), j = i + 1 .. n), i = 1 .. n));
slv := solve(DGinfo(LieDerivative(V, O3), "CoefficientSet"), {seq(seq((a || i) || j, j = i + 1 .. n), i = 1 .. n)});
tmp := 0 :for i to nops(slv) do if lhs(slv[i]) = rhs(slv[i]) then tmp := tmp + 1 :fi:od:
[nops(slv), binomial(n, 2), tmp];
DGsimplify(subs(slv, V))
O3 := ((3 dx1) ^ dx2) ^ dx3 + (dx1 ^ dx2) ^ dx4 + ((6 dx1) ^ dx2) ^ dx5
+ (dx1 ^ dx2) ^ dx6 + ((5 dx1) ^ dx3) ^ dx4 + ((2 dx1) ^ dx3) ^ dx6
+ ((3 dx1) ^ dx4) ^ dx5 + ((7 dx1) ^ dx4) ^ dx6 + ((3 dx1) ^ dx5) ^ dx6
+ ((3 dx2) ^ dx3) ^ dx4 + ((9 dx2) ^ dx3) ^ dx6 + ((7 dx2) ^ dx4) ^ dx5
+ ((9 dx2) ^ dx4) ^ dx6 + ((9 dx2) ^ dx5) ^ dx6 + ((9 dx3) ^ dx4) ^ dx5
+ ((2 dx3) ^ dx4) ^ dx6 + ((5 dx3) ^ dx5) ^ dx6 + (dx4 ^ dx5) ^ dx6
slv := {a12 = 0, a13 = 0, a14 = 0, a15 = 0, a16 = 0, a23 = 0, a24 = 0, a25 = 0, a26 = 0, a34
= 0, a35 = 0, a36 = 0, a45 = 0, a46 = 0, a56 = 0}
[15, 15, 0]
0 D_x1

```

```

> n := 7 : DGsetup([seq(x || i, i = 1 .. n)], M || n) :
O3 := evalDG(add(add(add(RandomTools[Generate](integer(range = 0 .. 9)) · dx || i &w dx
|| j &w dx || k, k = j + 1 .. n), j = i + 1 .. n), i = 1 .. n));
V := evalDG(add(add((a || i) || j · (x || j · D_x || i - x || i · D_x || j), j = i + 1 .. n), i = 1 .. n));
slv := solve(DGinfo(LieDerivative(V, O3), "CoefficientSet"), {seq(seq((a || i) || j, j = i + 1 .. n), i = 1 .. n)});
tmp := 0 :for i to nops(slv) do if lhs(slv[i]) = rhs(slv[i]) then tmp := tmp + 1 :fi:od:
[nops(slv), binomial(n, 2), tmp];
DGsimplify(subs(slv, V))
[21, 21, 0]
0 D_x1

```

```

> n := 8 : DGsetup([seq(x || i, i = 1 .. n)], M || n) :
O3 := evalDG(add(add(add(RandomTools[Generate](integer(range = 0 .. 9)) · dx || i &w dx
|| j &w dx || k, k = j + 1 .. n), j = i + 1 .. n), i = 1 .. n));
V := evalDG(add(add((a || i) || j · (x || j · D_x || i - x || i · D_x || j), j = i + 1 .. n), i = 1 .. n));
slv := solve(DGinfo(LieDerivative(V, O3), "CoefficientSet"), {seq(seq((a || i) || j, j = i + 1 .. n), i = 1 .. n)});
tmp := 0 :for i to nops(slv) do if lhs(slv[i]) = rhs(slv[i]) then tmp := tmp + 1 :fi:od:
[nops(slv), binomial(n, 2), tmp];
DGsimplify(subs(slv, V))
[28, 28, 0]
0 D_x1

```

```

> n := 9 : DGsetup( [seq(x||i, i = 1 ..n) ], M||n) :
O3 := evalDG(add(add(add(RandomTools[Generate](integer(range=0..9))·dx||i &w dx
||j &w dx||k, k=j+1 ..n), j=i+1 ..n), i=1 ..n)) :
V := evalDG(add(add((a||i)||j·(x||j·D_x||i - x||i·D_x||j), j=i+1 ..n), i=1 ..n)):
slv := solve(DGinfo(LieDerivative(V, O3), "CoefficientSet"), {seq(seq((a||i)||j, j=i+1
..n), i=1 ..n)}):
tmp := 0 :for i to nops(slv) do if lhs(slv[i]) = rhs(slv[i]) then tmp := tmp + 1 :fi:od:
[nops(slv), binomial(n, 2), tmp];
DGsimplify(subs(slv, V))

```

[36, 36, 0]  
0 D\_x1

(9)
