# Supplementary material for: Poincare function for moduli of differential-geometric structures
Source: arXiv:1802.01322 source file (2018-02-05)
Supplement: Supplementary file 2 [file ACS-inv-count.pdf]

This worksheet contains count of differential invariants of almost complex structures with respect to the diffeomorphism pseudogroup. The computation took several weeks on a computer with 2.40 GHz and 64 RAM

```
> with(DifferentialGeometry) : with(Tensor) : with(JetCalculus) : with(Tools) :  
with(PDEtools) : with(LinearAlgebra) : Preferences("ShowFramePrompt",false) :
```

We begin with the 4D case (this is a special case, and the number of invariants shall be computed by brute force in lower dimensions, before stabilization comes)

```
> DGsetup([x1, y1, x2, y2], [a11, a12, a21, a22, b11, b12, b21, b22], J3, 3) :  
> J := evalDG((a11 D_x1 + b11 D_y1 + a12 D_x2 + b12 D_y2) &t dx1 + (a11z D_x1  
+ b11z D_y1 + a12z D_x2 + b12z D_y2) &t dy1 + (a21 D_x1 + b21 D_y1 + a22 D_x2  
+ b22 D_y2) &t dx2 + (a21z D_x1 + b21z D_y1 + a22z D_x2 + b22z D_y2) &t dy2)  
J := (a11 D_x1) dx1 + (a11z D_x1) dy1 + (a21 D_x1) dx2 + (a21z D_x1) dy2  
+ (b11 D_y1) dx1 + (b11z D_y1) dy1 + (b21 D_y1) dx2 + (b21z D_y1) dy2  
+ (a12 D_x2) dx1 + (a12z D_x2) dy1 + (a22 D_x2) dx2 + (a22z D_x2) dy2  
+ (b12 D_y2) dx1 + (b12z D_y2) dy1 + (b22 D_y2) dx2 + (b22z D_y2) dy2
```

```
> sls := solve(DGinfo(evalDG(ContractIndices(J, J, [[2, 1]])) + (D_x1 &t dx1 + D_y1 &t dy1  
+ D_x2 &t dx2 + D_y2 &t dy2)), "CoefficientSet"), {a11z, a12z, a21z, a22z, b11z,  
b12z, b21z, b22z}) :  
> J := evalDG(subs({a11 = a11[], a12 = a12[], a21 = a21[], a22 = a22[], b11 = b11[], b12  
= b12[], b21 = b21[], b22 = b22[]}, subs(sls, J))) : ContractIndices(J, J, [[2, 1]])  
- (D_x1 dx1) - (D_y1 dy1) - (D_x2 dx2) - (D_y2 dy2)
```

```
> var := x1, y1, x2, y2 : phi1 := f1(var) : phi2 := f2(var) : psi1 := h1(var) : psi2 := h2(var) :  
declare(phi1) : declare(phi2) : declare(psi1) : declare(psi2) :
```

```
> DX := [D_x1, D_x2] : DY := [D_y1, D_y2] :  
DA := [[D_a11[], D_a12[]], [D_a21[], D_a22[]]] : DB := [[D_b11[], D_b12[]],  
[D_b21[], D_b22[]]] :
```

```
> X := evalDG(phi1 D_x1 + psi1 D_y1 + phi2 D_x2 + psi2 D_y2 + add(add(A[i][j] DA[i][j], j = 1  
..2), i = 1 ..2) + add(add(B[i][j] DB[i][j], j = 1 ..2), i = 1 ..2)) :
```

```
> slAB := solve(DGinfo(ContractIndices(LieDerivative(X, J), D_x1, [[2, 1]]),  
"CoefficientSet") union DGinfo(ContractIndices(LieDerivative(X, J), D_x2, [[2, 1]]),  
"CoefficientSet"), {A11, A12, A21, A22, B11, B12, B21, B22}) :
```

```
> X := evalDG(subs(slAB, X)) :
```

```
> X0 := ToJet(X, {phi1, phi2, psi1, psi2}, notation = jetnumbers) :  
X1 := ToJet(Prolong(X, 1), {phi1, phi2, psi1, psi2}, notation = jetnumbers) :  
X2 := ToJet(Prolong(X, 2), {phi1, phi2, psi1, psi2}, notation = jetnumbers) :  
X3 := ToJet(Prolong(X, 3), {phi1, phi2, psi1, psi2}, notation = jetnumbers) :
```

```
> pt0 := {x1, y1, x2, y2, seq(seq((a[i][j])[], j = 1 ..2), i = 1 ..2), seq(seq((b[i][j])[], j = 1  
..2), i = 1 ..2)} :  
ptp1 := {seq(seq(seq((a[i][j])_k, j = 1 ..2), i = 1 ..2), k = 1 ..4), seq(seq(seq((b[i][j])_k, j = 1  
..2), i = 1 ..2), k = 1 ..4)} : ptp1 := pt0 union ptp1 :  
ptp2 := {seq(seq(seq(seq((a[i][j])_k, j = 1 ..2), i = 1 ..2), l = k ..4), k = 1 ..4),  
seq(seq(seq(seq((b[i][j])_k, j = 1 ..2), i = 1 ..2), l = k ..4), k = 1 ..4)} : ptp2 := ptp1  
union ptp2 :
```

```
> rnd := rand(0 ..9) :
```

```
> Pt0 := {x1 = 0, y1 = 0, x2 = 0, y2 = 0, a11[] = 0, a12[] = 0, a21[] = 0, a22[] = 0, b11[] = 1,  
b12[] = 0, b21[] = 0, b22[] = 1} :
```

**for**  $s$  **to** 2 **do**  $(Ptp \parallel s) := \{seq((ptp \parallel s)[t] = rnd(), t = 1 \dots nops(ptp \parallel s))\} : (Pt \parallel s) := (Pt \parallel (s - 1)) \text{ union } (Ptp \parallel s) : \text{od}$

$\triangleright$   $gp0 := \{fl_{[]}, hl_{[]}, f2_{[]}, h2_{[]}\} :$   
 $gpp1 := \{seq(seq((f \parallel k)_{i,j}, i = 1 \dots 4), k = 1 \dots 2), seq(seq((h \parallel k)_{i,j}, i = 1 \dots 4), k = 1 \dots 2)\} : gp1$   
 $:= gp0 \text{ union } gpp1 :$   
 $gpp2 := \{seq(seq(seq((f \parallel k)_{i,j}, j = i \dots 4), i = 1 \dots 4), k = 1 \dots 2), seq(seq(seq((h \parallel k)_{i,j}, j = i \dots 4), i = 1 \dots 4), k = 1 \dots 2)\} : gp2 := gp1 \text{ union } gpp2 :$   
 $gpp3 := \{seq(seq(seq(seq((f \parallel k)_{i,j,l}, l = j \dots 4), j = i \dots 4), i = 1 \dots 4), k = 1 \dots 2), seq(seq(seq(seq((h \parallel k)_{i,j,l}, l = j \dots 4), j = i \dots 4), i = 1 \dots 4), k = 1 \dots 2)\} : gp3 := gp2 \text{ union } gpp3 :$

$\triangleright$   $subs(Pt0, X0)$   
 $fl_{[]} D_{x1} + hl_{[]} D_{y1} + f2_{[]} D_{x2} + h2_{[]} D_{y2} + (fl_2 + hl_1) D_{a11} + (f2_2 + h2_1) D_{a12} + (fl_4 + hl_3) D_{a21} + (f2_4 + h2_3) D_{a22} - (fl_1 - hl_2) D_{b11} - ((f2_1 - h2_2) D_{b12}) - ((fl_3 - hl_4) D_{b21}) - ((f2_3 - h2_4) D_{b22})$  (3)

$\triangleright$   $sl0 := solve(DGinfo(subs(Pt0, X0), "CoefficientSet"), gp1) ;$   
 $fv0 := \{ \} : \text{for } i \text{ to } nops(sl0) \text{ do if } lhs(sl0[i]) = rhs(sl0[i]) \text{ then } fv0 := fv0 \text{ union } \{lhs(sl0[i])\} : \text{fi:od} : fv0 ; n0 := nops(\%) : [n0, n0]$   
 $sl0 := \{fl_{[]} = 0, fl_1 = hl_2, fl_2 = -hl_1, fl_3 = hl_4, fl_4 = -hl_3, f2_{[]} = 0, f2_1 = h2_2, f2_2 = -h2_1, f2_3 = h2_4, f2_4 = -h2_3, hl_{[]} = 0, hl_1 = hl_1, hl_2 = hl_2, hl_3 = hl_3, hl_4 = hl_4, h2_{[]} = 0, h2_1 = h2_1, h2_2 = h2_2, h2_3 = h2_3, h2_4 = h2_4\}$   
 $\{hl_1, hl_2, hl_3, hl_4, h2_1, h2_2, h2_3, h2_4\}$   
 $[8, 8]$  (4)

$\triangleright$   $nops(gp1), nops(pt0), nops(pt0) - nops(gp1) + n0$   
 $20, 12, 0$  (5)

$\triangleright$   $sl1 := solve(DGinfo(subs(Pt1, X1), "CoefficientSet"), gp2) :$   
 $fv1 := \{ \} : \text{for } i \text{ to } nops(sl1) \text{ do if } lhs(sl1[i]) = rhs(sl1[i]) \text{ then } fv1 := fv1 \text{ union } \{lhs(sl1[i])\} : \text{fi:od} : fv1 ; n1 := nops(\%) : [n1, n1 - n0]$   
 $\{fl_{1,2}, fl_{1,3}, fl_{2,3}, fl_{3,4}, f2_{3,2}, f2_{1,2}, f2_{1,3}, f2_{1,4}, f2_{3,4}, hl_{1,2}, hl_{1,3}, hl_{1,4}, h2_{1,2}, h2_{3,2}, h2_{3,4}\}$   
 $[16, 8]$  (6)

$\triangleright$   $nops(gp2), nops(pt1), nops(pt1) - nops(gp2) + n1$   
 $60, 44, 0$  (7)

$\triangleright$   $sl2 := solve(DGinfo(subs(Pt2, X2), "CoefficientSet"), gp3) :$   
 $fv2 := \{ \} : \text{for } i \text{ to } nops(sl2) \text{ do if } lhs(sl2[i]) = rhs(sl2[i]) \text{ then } fv2 := fv2 \text{ union } \{lhs(sl2[i])\} : \text{fi:od} : fv2 ; n2 := nops(\%) : [n2, n2 - n1]$   
 $\{fl_{1,2,2}, fl_{3,4,4}, f2_{1,2}, f2_{1,4}, f2_{1,2,2}, f2_{3,4,4}, hl_{1,2,2}, hl_{1,2,3}, hl_{1,2,4}, hl_{1,3,4}, hl_{2,3,4}, h2_{3,4,4}, h2_{1,2,2}, h2_{1,2,3}, h2_{1,2,4}, h2_{1,3,4}, h2_{2,3,4}, h2_{3,4,4}\}$   
 $[18, 2]$  (8)

$\triangleright$   $nops(gp3), nops(pt2), nops(pt2) - nops(gp3) + n2$   
 $140, 124, 2$  (9)

$\triangleright$   $ptp3 := \{seq(seq(seq(seq(seq((a \parallel i \parallel j)_{k,l,m}, j = 1 \dots 2), i = 1 \dots 2), m = l \dots 4), l = k \dots 4), k = 1 \dots 4), seq(seq(seq(seq(seq((b \parallel i \parallel j)_{k,l,m}, j = 1 \dots 2), i = 1 \dots 2), m = l \dots 4), l = k \dots 4), k = 1 \dots 4)\} : pt3 := pt2 \text{ union } ptp3 :$   
 $Ptp3 := \{seq(ptp3[t] = rnd(), t = 1 \dots nops(ptp3))\} : Pt3 := Pt2 \text{ union } Ptp3 :$   
 $gpp4 := \{seq(seq(seq(seq(seq((f \parallel k)_{i,j,l,m}, m = l \dots 4), l = j \dots 4), j = i \dots 4), i = 1 \dots 4), k = 1 \dots 2$

$\}, seq(seq(seq(seq(seq((h \parallel k)_{i,j,l,m}, m=l..4), l=j..4), j=i..4), i=1..4), k=1..2) \}$   
 $: gp4 := gp3 \text{ union } gpp4 :$

>  $sl3 := solve(DGinfo(subs(Pt3, X3), "CoefficientSet"), gp4) :$   
 $fv3 := \{ \} : \text{for } i \text{ to } nops(sl3) \text{ do if } lhs(sl3[i]) = rhs(sl3[i]) \text{ then } fv3 := fv3$   
 $\text{union } \{lhs(sl3[i]) \} : \text{fi:od: } fv3; n3 := nops(\%) : [n3, n3 - n2]$   
 $\{f1_{1,1,2,2}, f1_{1,2,2,3}, f1_{1,2,2,4}, f1_{1,2,3,4}, f1_{1,3,4,4}, f1_{2,3,4,4}, f1_{3,3,4,4}, f2_{1,1,2,2}, f2_{1,2,2,3},$   
 $f2_{1,2,2,4}, f2_{1,2,3,4}, f2_{1,3,4,4}, f2_{2,3,4,4}, f2_{3,3,4,4}, h1_{1,1,2,2}, h1_{1,2,3,4}, h1_{3,3,4,4}, h2_{1,2,2,3},$   
 $h2_{1,3,4,4}, h2_{1,1,2,2}, h2_{1,2,3,4}, h2_{3,3,4,4} \}$   
 $[22, 4] \quad (10)$

>  $nops(gp4), nops(pt3), nops(pt3) - nops(gp4) + n3$   
 $280, 284, 26 \quad (11)$

>  $X4 := ToJet(Prolong(X, 4), \{\phi1, \phi2, \psi1, \psi2\}, notation = jetnumbers) :$   
>  $ptp4 := \{seq(seq(seq(seq(seq(seq((a \parallel i \parallel j)_{k,l,m,n}, j=1..2), i=1..2), n=m..4), m=l..4), l=k..4), k=1..4), seq(seq(seq(seq(seq(seq((b \parallel i \parallel j)_{k,l,m,n}, j=1..2), i=1..2), n=m..4), m=l..4), l=k..4), k=1..4) \} : pt4 := pt3 \text{ union } ptp4 :$   
 $Ptp4 := \{seq(ptp4[t] = rnd( ), t = 1..nops(ptp4)) \} : Pt4 := Pt3 \text{ union } Ptp4 :$   
 $gpp5 := \{seq(seq(seq(seq(seq(seq((f \parallel k)_{i,j,l,m,n}, n=m..4), m=l..4), l=j..4), j=i..4), i=1..4), k=1..2), seq(seq(seq(seq(seq(seq((h \parallel k)_{i,j,l,m,n}, n=m..4), m=l..4), l=j..4), j=i..4), i=1..4), k=1..2) \} : gp5 := gp4 \text{ union } gpp5 :$   
>  $sl4 := solve(DGinfo(subs(sl3, subs(sl2, subs(sl1, subs(sl0, subs(Pt4, X4))))), "CoefficientSet") :$   
 $fv4 := \{ \} : \text{for } i \text{ to } nops(sl4) \text{ do if } lhs(sl4[i]) = rhs(sl4[i]) \text{ then } fv4 := fv4$   
 $\text{union } \{lhs(sl4[i]) \} : \text{fi:od: } fv4; n4 := nops(\%) : [n4, n4 - n3]$   
 $\{f1_{1,1,2,2}, f1_{1,1,2,3}, f1_{1,2,3,4}, f1_{2,3,3,4}, f1_{3,3,3,4}, f2_{1,2,2,3}, f2_{1,2,2,4}, f2_{1,1,1,2,2},$   
 $f2_{1,1,1,2,3}, f2_{1,1,1,2,4}, f2_{1,1,2,2,2}, f2_{1,1,2,3,4}, f2_{1,2,3,4,4}, f2_{2,3,3,3,4}, f2_{2,3,3,4,4},$   
 $f2_{3,3,3,4,4}, f2_{3,3,4,4,4}, h1_{1,1,2,2,2}, h1_{1,1,2,3,4}, h1_{1,2,2,2,4}, h1_{1,2,2,3,4}, h1_{1,2,3,4,4},$   
 $h1_{1,3,3,3,4}, h1_{3,3,3,4,4}, h2_{1,1,2,3,4}, h2_{1,2,3,4,4} \}$   
 $[26, 4] \quad (12)$

>  $nops(gp5), nops(pt4), nops(pt4) - nops(gp5) + n4$   
 $504, 564, 86 \quad (13)$

>  $X5 := ToJet(Prolong(X, 5), \{\phi1, \phi2, \psi1, \psi2\}, notation = jetnumbers) :$   
>  $ptp5 := \{seq(seq(seq(seq(seq(seq(seq((a \parallel i \parallel j)_{k,l,m,n,o}, j=1..2), i=1..2), o=n..4), n=m..4), m=l..4), l=k..4), k=1..4), seq(seq(seq(seq(seq(seq(seq((b \parallel i \parallel j)_{k,l,m,n,o}, j=1..2), i=1..2), o=n..4), n=m..4), m=l..4), l=k..4), k=1..4) \} : pt5 := pt4 \text{ union } ptp5 :$   
 $Ptp5 := \{seq(ptp5[t] = rnd( ), t = 1..nops(ptp5)) \} : Pt5 := Pt4 \text{ union } Ptp5 :$   
 $gpp6 := \{seq(seq(seq(seq(seq(seq(seq((f \parallel k)_{i,j,l,m,n,o}, o=n..4), n=m..4), m=l..4), l=j..4), j=i..4), i=1..4), k=1..2), seq(seq(seq(seq(seq(seq(seq((h \parallel k)_{i,j,l,m,n,o}, o=n..4), n=m..4), m=l..4), l=j..4), j=i..4), i=1..4), k=1..2) \} : gp6 := gp5$   
 $\text{union } gpp6 :$   
>  $sl5 := solve(DGinfo(subs(sl4, subs(sl3, subs(sl2, subs(sl1, subs(sl0, subs(Pt5, X5))))), "CoefficientSet") :$   
 $fv5 := \{ \} : \text{for } i \text{ to } nops(sl5) \text{ do if } lhs(sl5[i]) = rhs(sl5[i]) \text{ then } fv5 := fv5$   
 $\text{union } \{lhs(sl5[i]) \} : \text{fi:od: } fv5; n5 := nops(\%) : [n5, n5 - n4]$   
 $\{f1_{1,2,3,4,4}, f1_{1,1,1,2,2,2}, f1_{1,1,1,2,3,4}, f1_{1,1,2,2,3,4}, f1_{1,2,2,3,4,4}, f1_{1,2,3,3,4,4}, f1_{1,2,3,4,4,4},$

$$\begin{aligned} & f1_{1,3,3,3,4,4}, f1_{3,3,3,4,4}, f2_{1,1,1,2,2,2}, f2_{1,1,2,2,3,4}, f2_{1,1,2,3,4,4}, f2_{1,2,2,2,3,4}, \\ & f2_{1,2,2,3,4,4}, f2_{1,2,3,3,4,4}, f2_{1,2,3,4,4,4}, f2_{2,3,3,3,4,4}, f2_{2,3,3,3,4,4}, f2_{3,3,3,4,4,4}, \\ & h1_{1,2,3,4,4}, h1_{1,1,1,2,2,2}, h1_{1,1,2,2,2,3}, h1_{1,1,2,2,2,4}, h1_{1,2,2,3,4,4}, h1_{1,3,4,4,4,4}, \\ & h1_{3,3,3,4,4,4}, h2_{1,1,1,2,2,3}, h2_{1,1,1,2,2,2}, h2_{1,2,2,2,2,3}, h2_{3,3,3,4,4,4} \} \end{aligned}$$

$$[30, 4] \quad (14)$$

$$> nops(gp6), nops(pt5), nops(pt5) - nops(gp6) + n5 \\ 840, 1012, 202 \quad (15)$$

$$> length(X5) \\ 7799975748 \quad (16)$$

$$> length(X4) \\ 704799042 \quad (17)$$

$$> length(X3) \\ 48657882 \quad (18)$$

$$> length(X2) \\ 2925095 \quad (19)$$

$$> length(X1) \\ 131938 \quad (20)$$

Now let us consider the 6D case (this is the second special case; starting from dimension  $2n=8$  the number of invariants is determined without computer calculations)

$$\begin{aligned} & > DGsetup([x1, y1, x2, y2, x3, y3], [a11, a12, a13, a21, a22, a23, a31, a32, a33, b11, b12, \\ & \quad b13, b21, b22, b23, b31, b32, b33], J3, 3) : \\ & > J := evalDG((a11 D_x1 + b11 D_y1 + a12 D_x2 + b12 D_y2 + a13 D_x3 + b13 D_y3) \\ & \quad \& dx1 + (a11z D_x1 + b11z D_y1 + a12z D_x2 + b12z D_y2 + a13z D_x3 \\ & \quad + b13z D_y3) \& dy1 + (a21 D_x1 + b21 D_y1 + a22 D_x2 + b22 D_y2 + a23 D_x3 \\ & \quad + b23 D_y3) \& dx2 + (a21z D_x1 + b21z D_y1 + a22z D_x2 + b22z D_y2 + a23z D_x3 \\ & \quad + b23z D_y3) \& dy2 + (a31 D_x1 + b31 D_y1 + a32 D_x2 + b32 D_y2 + a33 D_x3 \\ & \quad + b33 D_y3) \& dx3 + (a31z D_x1 + b31z D_y1 + a32z D_x2 + b32z D_y2 + a33z D_x3 \\ & \quad + b33z D_y3) \& dy3) : \\ & > sls := solve(DGinfo(evalDG(ContractIndices(J, J, [[2, 1]])) + (D_x1 \& dx1 + D_y1 \& dy1 \\ & \quad + D_x2 \& dx2 + D_y2 \& dy2 + D_x3 \& dx3 + D_y3 \& dy3)), "CoefficientSet"), \\ & \quad \{a11z, a12z, a13z, a21z, a22z, a23z, a31z, a32z, a33z, b11z, b12z, b13z, b21z, b22z, b23z, \\ & \quad b31z, b32z, b33z\}) : \\ & > J := evalDG(subs(\{a11 = a11_{[]}, a12 = a12_{[]}, a13 = a13_{[]}, a21 = a21_{[]}, a22 = a22_{[]}, a23 \\ & \quad = a23_{[]}, a31 = a31_{[]}, a32 = a32_{[]}, a33 = a33_{[]}, b11 = b11_{[]}, b12 = b12_{[]}, b13 = b13_{[]}, \\ & \quad b21 = b21_{[]}, b22 = b22_{[]}, b23 = b23_{[]}, b31 = b31_{[]}, b32 = b32_{[]}, b33 = b33_{[]}\}, subs(sls, \\ & \quad J))) : ContractIndices(J, J, [[2, 1]]) \\ & \quad - (D_x1 dx1) - (D_y1 dy1) - (D_x2 dx2) - (D_y2 dy2) - (D_x3 dx3) - (D_y3 dy3) \quad (21) \end{aligned}$$

$$\begin{aligned} & > var := x1, y1, x2, y2, x3, y3 : \varphi1 := f1(var) : \varphi2 := f2(var) : \varphi3 := f3(var) : \psi1 \\ & \quad := h1(var) : \psi2 := h2(var) : \psi3 := h3(var) : declare(\varphi1) : declare(\varphi2) : \\ & \quad declare(\varphi3) : declare(\psi1) : declare(\psi2) : declare(\psi3) : \\ & > DX := [D_x1, D_x2, D_x3] : DY := [D_y1, D_y2, D_y3] : \\ & \quad DA := [[D_a11_{[]}, D_a12_{[]}, D_a13_{[]}], [D_a21_{[]}, D_a22_{[]}, D_a23_{[]}], [D_a31_{[]}, D_a32_{[]}, \\ & \quad D_a33_{[]}]] : DB := [[D_b11_{[]}, D_b12_{[]}, D_b13_{[]}], [D_b21_{[]}, D_b22_{[]}, D_b23_{[]}], \\ & \quad [D_b31_{[]}, D_b32_{[]}, D_b33_{[]}]] : \\ & > X := evalDG(\varphi1 D_x1 + \psi1 D_y1 + \varphi2 D_x2 + \psi2 D_y2 + \varphi3 D_x3 + \psi3 D_y3 \\ & \quad + add(add(A || i || j \cdot DA[i, j], j = 1 .. 3), i = 1 .. 3) + add(add(B || i || j \cdot DB[i, j], j = 1 .. 3), i \\ & \quad = 1 .. 3)) : \end{aligned}$$

```

> slAB := solve(DGinfo(ContractIndices(LieDerivative(X, J), D_x1, [[2, 1]]),
  "CoefficientSet") union DGinfo(ContractIndices(LieDerivative(X, J), D_x2, [[2, 1]]),
  "CoefficientSet") union DGinfo(ContractIndices(LieDerivative(X, J), D_x3, [[2, 1]]),
  "CoefficientSet"), {A11, A12, A13, A21, A22, A23, A31, A32, A33, B11, B12, B13, B21,
  B22, B23, B31, B32, B33}) :
> X := evalDG(subs(slAB, X)) :
> X0 := ToJet(X, {φ1, φ2, φ3, ψ1, ψ2, ψ3}, notation = jetnumbers) :
X1 := ToJet(Prolong(X, 1), {φ1, φ2, φ3, ψ1, ψ2, ψ3}, notation = jetnumbers) :
X2 := ToJet(Prolong(X, 2), {φ1, φ2, φ3, ψ1, ψ2, ψ3}, notation = jetnumbers) :
X3 := ToJet(Prolong(X, 3), {φ1, φ2, φ3, ψ1, ψ2, ψ3}, notation = jetnumbers) :
> pt0 := {x1, y1, x2, y2, x3, y3, seq(seq((a || i || j)_[j], j = 1 ..3), i = 1 ..3), seq(seq((b || i || j)_[j], j
  = 1 ..3), i = 1 ..3)} :
ptp1 := {seq(seq(seq((a || i || j)_[j], j = 1 ..3), i = 1 ..3), k = 1 ..6), seq(seq(seq((b || i || j)_[j], j = 1
  ..3), i = 1 ..3), k = 1 ..6)} : ptp1 := pt0 union ptp1 :
ptp2 := {seq(seq(seq(seq((a || i || j)_[j], j = 1 ..3), i = 1 ..3), l = k ..6), k = 1 ..6),
  seq(seq(seq(seq((b || i || j)_[j], j = 1 ..3), i = 1 ..3), l = k ..6), k = 1 ..6)} : ptp2 := ptp1
union ptp2 :
> rnd := rand(0 ..9) :
> Pt0 := {x1 = 0, y1 = 0, x2 = 0, y2 = 0, x3 = 0, y3 = 0, a11_[ ] = 0, a12_[ ] = 0, a13_[ ] = 0, a21_[ ]
  = 0, a22_[ ] = 0, a23_[ ] = 0, a31_[ ] = 0, a32_[ ] = 0, a33_[ ] = 0, b11_[ ] = 1, b12_[ ] = 0, b13_[ ] = 0,
  b21_[ ] = 0, b22_[ ] = 1, b23_[ ] = 0, b31_[ ] = 0, b32_[ ] = 0, b33_[ ] = 1} :
for s to 3 do (Ptp || s) := {seq((ptp || s)[t] = rnd(), t = 1 ..nops(ptp || s))} : (Pt || s) := (Pt || (s
  - 1)) union (Ptp || s) : od :
> gp0 := {f1_[ ], h1_[ ], f2_[ ], h2_[ ], f3_[ ], h3_[ ]} :
gpp1 := {seq(seq((f || k)_[j], j = 1 ..6), k = 1 ..3), seq(seq((h || k)_[j], j = 1 ..6), k = 1 ..3)} : gp1
  := gp0 union gpp1 :
gpp2 := {seq(seq(seq((f || k)_[j], j = i ..6), i = 1 ..6), k = 1 ..3), seq(seq(seq((h || k)_[j], j = i
  ..6), i = 1 ..6), k = 1 ..3)} : gp2 := gp1 union gpp2 :
gpp3 := {seq(seq(seq(seq((f || k)_[j], j = l ..6), l = j ..6), j = i ..6), i = 1 ..6), k = 1 ..3), seq(seq(seq
  (seq((h || k)_[j], j = l ..6), l = j ..6), j = i ..6), i = 1 ..6), k = 1 ..3)} : gp3 := gp2 union gpp3 :
> subs(Pt0, X0)
fl[ ] D_x1 + hl[ ] D_y1 + f2[ ] D_x2 + h2[ ] D_y2 + f3[ ] D_x3 + h3[ ] D_y3 + (fl2
  + hl1) D_a11[ ] + (f22 + h21) D_a12[ ] + (f32 + h31) D_a13[ ] + (fl4
  + hl3) D_a21[ ] + (f24 + h23) D_a22[ ] + (f34 + h33) D_a23[ ] + (fl6
  + hl5) D_a31[ ] + (f26 + h25) D_a32[ ] + (f36 + h35) D_a33[ ] - ((fl1
  - hl2) D_b11[ ]) - ((f21 - h22) D_b12[ ]) - ((f31 - h32) D_b13[ ]) - ((fl3
  - hl4) D_b21[ ]) - ((f23 - h24) D_b22[ ]) - ((f33 - h34) D_b23[ ]) - ((fl5
  - hl6) D_b31[ ]) - ((f25 - h26) D_b32[ ]) - ((f35 - h36) D_b33[ ])
(22)
> sl0 := solve(DGinfo(subs(Pt0, X0), "CoefficientSet"), gp1);
fv0 := {} for i to nops(sl0) do if lhs(sl0[i]) = rhs(sl0[i]) then fv0 := fv0
  union {lhs(sl0[i])} fi : od : fv0; n0 := nops(%) : [n0, n0]
sl0 := {f1_[ ] = 0, f11 = h12, f12 = -h11, f13 = h14, f14 = -h13, f15 = h16, f16 = -h15, f2_[ ] = 0, f21
  = h22, f22 = -h21, f23 = h24, f24 = -h23, f25 = h26, f26 = -h25, f3_[ ] = 0, f31 = h32, f32 =
  -h31, f33 = h34, f34 = -h33, f35 = h36, f36 = -h35, h1_[ ] = 0, h11 = h11, h12 = h12, h13 = h13,

```

$$\begin{aligned}
& h1_4 = h1_4, h1_5 = h1_5, h1_6 = h1_6, h2_{[]} = 0, h2_1 = h2_1, h2_2 = h2_2, h2_3 = h2_3, h2_4 = h2_4, h2_5 \\
& = h2_5, h2_6 = h2_6, h3_{[]} = 0, h3_1 = h3_1, h3_2 = h3_2, h3_3 = h3_3, h3_4 = h3_4, h3_5 = h3_5, h3_6 = h3_6 \} \\
& \{ h1_1, h1_2, h1_3, h1_4, h1_5, h1_6, h2_1, h2_2, h2_3, h2_4, h2_5, h2_6, h3_1, h3_2, h3_3, h3_4, h3_5, h3_6 \} \\
& [18, 18]
\end{aligned} \tag{23}$$

$$\begin{aligned}
& > nops(gp1), nops(pt0), nops(pt0) - nops(gp1) + n0 \\
& 42, 24, 0
\end{aligned} \tag{24}$$

$$\begin{aligned}
& > sl1 := solve(DGinfo(subs(Pt1, X1), "CoefficientSet"), gp2) : \\
& fv1 := \{ \} : \text{for } i \text{ to } nops(sl1) \text{ do if } lhs(sl1[i]) = rhs(sl1[i]) \text{ then } fv1 := fv1 \\
& \quad \text{union } \{ lhs(sl1[i]) \} : \text{fi:od: } fv1; n1 := nops(\%) : [n1, n1 - n0] \\
& \{ f1_{1,2}, f1_{3,4}, f1_{5,6}, f2_{1,2}, f2_{2,3}, f2_{3,4}, f2_{5,6}, f3_{1,2}, f3_{1,5}, f3_{2,5}, f3_{3,4}, f3_{3,5}, f3_{5,6}, h1_1, h1_3, h1_{1,2}, \\
& \quad h1_{2,3}, h1_{2,4}, h1_{2,5}, h1_{2,6}, h1_{3,4}, h1_{4,5}, h1_{4,6}, h1_{5,6}, h2_{1,2}, h2_{1,5}, h2_{1,6}, h2_{2,3}, h2_{3,4}, \\
& \quad h2_{4,5}, h2_{4,6}, h2_{5,6}, h3_{1,2}, h3_{1,4}, h3_{2,4}, h3_{3,4}, h3_{3,5}, h3_{5,6} \} \\
& [38, 20]
\end{aligned} \tag{25}$$

$$\begin{aligned}
& > nops(gp2), nops(pt1), nops(pt1) - nops(gp2) + n1 \\
& 168, 132, 2
\end{aligned} \tag{26}$$

$$\begin{aligned}
& > sl2 := solve(DGinfo(subs(Pt2, X2), "CoefficientSet"), gp3) : \\
& fv2 := \{ \} : \text{for } i \text{ to } nops(sl2) \text{ do if } lhs(sl2[i]) = rhs(sl2[i]) \text{ then } fv2 := fv2 \\
& \quad \text{union } \{ lhs(sl2[i]) \} : \text{fi:od: } fv2; n2 := nops(\%) : [n2, n2 - n1] \\
& \{ f1_{1,2}, f1_{1,2,4}, f1_{2,3}, f1_{2,5}, f1_{3,4}, f1_{3,5}, f1_{5,6}, f2_{1,2}, f2_{1,2,3}, f2_{1,2,5}, f2_{2,3}, f2_{2,3,4}, f2_{2,3,5}, f2_{3,4}, f2_{3,5}, f2_{5,6}, f3_{1,2}, f3_{1,2,5}, f3_{1,3}, f3_{1,3,4}, f3_{1,3,5}, f3_{1,4}, f3_{1,4,5}, f3_{1,5}, f3_{2,3}, f3_{2,3,4}, f3_{2,3,5}, f3_{3,4}, f3_{3,4,5}, f3_{5,6}, h1_{1,2}, h1_{1,2,4}, h1_{1,2,5}, h1_{1,2,6}, h1_{2,3}, h1_{2,3,4}, h1_{2,3,6}, h1_{2,4}, h1_{2,4,6}, h1_{2,5}, h1_{3,4}, h1_{3,4,5}, h1_{3,4,6}, h1_{3,5}, h1_{3,5,6}, h2_{1,2}, h2_{1,2,3}, h2_{1,2,5}, h2_{1,5}, h2_{2,3}, h2_{2,3,4}, h2_{2,3,5}, h2_{2,4}, h2_{2,4,5}, h2_{2,5}, h2_{3,4}, h2_{3,4,5}, h2_{3,5}, h2_{3,5,6}, h3_{1,2}, h3_{1,2,3}, h3_{1,2,4}, h3_{1,2,5}, h3_{1,5}, h3_{3,4}, h3_{3,4,4}, h3_{3,4,5}, h3_{3,5}, h3_{3,5,6}, h3_{4,5}, h3_{5,6}, h3_{5,6,6} \} \\
& [60, 22]
\end{aligned} \tag{27}$$

$$\begin{aligned}
& > nops(gp3), nops(pt2), nops(pt2) - nops(gp3) + n2 \\
& 504, 510, 66
\end{aligned} \tag{28}$$

$$\begin{aligned}
& > ptp3 := \{ seq(seq(seq(seq(seq((a || i || j)_{k,l,m}, j = 1..3), i = 1..3), m = l..6), l = k..6), k = 1 \\
& \quad ..6), seq(seq(seq(seq(seq((b || i || j)_{k,l,m}, j = 1..3), i = 1..3), m = l..6), l = k..6), k = 1 \\
& \quad ..6) \} : pt3 := pt2 \text{ union } ptp3 : \\
& Ptp3 := \{ seq(ptp3[t] = rnd( ), t = 1..nops(ptp3) \} : Pt3 := Pt2 \text{ union } Ptp3 : \\
& gpp4 := \{ seq(seq(seq(seq(seq((f || k)_{i,j,l,m}, m = l..6), l = j..6), j = i..6), i = 1..6), k = 1..3 \\
& \quad ), seq(seq(seq(seq(seq((h || k)_{i,j,l,m}, m = l..6), l = j..6), j = i..6), i = 1..6), k = 1..3) \} \\
& : gp4 := gp3 \text{ union } gpp4 :
\end{aligned}$$

$$\begin{aligned}
& > sl3 := solve(DGinfo(subs(Pt3, X3), "CoefficientSet"), gp4) : \\
& fv3 := \{ \} : \text{for } i \text{ to } nops(sl3) \text{ do if } lhs(sl3[i]) = rhs(sl3[i]) \text{ then } fv3 := fv3 \\
& \quad \text{union } \{ lhs(sl3[i]) \} : \text{fi:od: } fv3; n3 := nops(\%) : [n3, n3 - n2] \\
& \{ f1_{1,1,2}, f1_{1,2,2}, f1_{1,2,2,3}, f1_{1,2,2,4}, f1_{1,2,2,5}, f1_{1,2,2,6}, f1_{1,2,3}, f1_{1,2,3,5}, f1_{1,2,5}, f1_{1,3,4}, f1_{1,3,4,6}, f1_{2,3,5}, f1_{2,4,5}, f1_{2,4,5,6}, f1_{3,3,4}, f1_{3,4,5}, f1_{5,5,6}, f2_{1,1,2}, f2_{1,2,2}, f2_{1,2,2,3}, f2_{1,2,2,4}, f2_{1,2,2,6}, f2_{1,2,3}, f2_{1,2,5}, f2_{1,3,4}, f2_{2,3,4}, f2_{3,3,4}, f2_{3,4,4}, f2_{3,4,4,5}, f2_{3,4,5}, f2_{4,5,6}, f2_{5,5,6}, f3_{1,1,2}, f3_{1,1,4}, f3_{1,2,3}, f3_{1,2,4}, f3_{1,2,5}, f3_{1,3,4}, f3_{2,3,3}, f3_{2,3,4}, f3_{2,3,4,5}, f3_{2,5,6}, f3_{3,3,4}, f3_{3,3,4,4}, f3_{3,3,4,5}, f3_{3,4,5}, f3_{3,5,6}, f3_{4,5,6}, f3_{5,5,6}, h1_{1,1,2}, h1_{1,2,2}, h1_{1,2,2,3}, h1_{1,2,2,4}, h1_{1,2,2,5}, h1_{1,2,2,6}, h1_{1,2,3}, h1_{1,2,3,5}, h1_{1,2,5}, h1_{1,3,4}, h1_{1,3,4,6}, h1_{1,3,6}, h1_{2,3}, h1_{2,3,4}, h1_{2,3,4,5}, h1_{2,3,4,6}, h1_{2,3,6}, h1_{2,4}, h1_{2,4,5}, h1_{2,4,6}, h1_{2,5}, h1_{2,5,6}, h1_{3,4}, h1_{3,4,5}, h1_{3,4,6}, h1_{3,5}, h1_{3,5,6}, h1_{4,5}, h1_{4,5,6}, h1_{5,6}, h1_{5,6,6} \}
\end{aligned}$$

$$\begin{aligned}
& h1_{1, 2, 3, 4}, h1_{1, 2, 4, 6}, h1_{1, 2, 5, 6}, h1_{1, 3, 4, 4}, h1_{1, 5, 6, 6}, h1_{2, 3, 4, 4}, h1_{2, 5, 6, 6}, h1_{3, 3, 4, 4}, \\
& h1_{3, 4, 4, 5}, h1_{3, 4, 4, 6}, h1_{3, 4, 5, 6}, h1_{3, 5, 6, 6}, h1_{4, 5, 6, 6}, h1_{5, 5, 6, 6}, h2_{1, 1, 2, 2}, h2_{1, 2, 2, 6}, \\
& h2_{1, 2, 3, 4}, h2_{1, 2, 3, 5}, h2_{1, 2, 3, 6}, h2_{1, 2, 5, 6}, h2_{1, 3, 4, 5}, h2_{1, 3, 4, 6}, h2_{1, 5, 6, 6}, h2_{2, 3, 5, 6}, \\
& h2_{2, 4, 5, 6}, h2_{2, 5, 6, 6}, h2_{3, 3, 4, 4}, h2_{3, 3, 4, 6}, h2_{3, 4, 5, 6}, h2_{4, 5, 6, 6}, h2_{5, 5, 6, 6}, h3_{1, 1, 2, 2}, \\
& h3_{1, 2, 2, 3}, h3_{1, 2, 2, 4}, h3_{1, 2, 2, 5}, h3_{1, 2, 2, 6}, h3_{1, 2, 3, 4}, h3_{1, 2, 5, 6}, h3_{1, 3, 5, 6}, h3_{1, 4, 5, 6}, \\
& h3_{2, 5, 6, 6}, h3_{3, 3, 4, 4}, h3_{3, 4, 4, 6}, h3_{3, 4, 5, 6}, h3_{5, 5, 6, 6} \} \\
& \qquad \qquad \qquad [90, 30] \tag{29}
\end{aligned}$$

$$\begin{aligned}
& \textcolor{red}{> } nops(gp4), nops(pt3), nops(pt3) - nops(gp4) + n3 \\
& \qquad \qquad \qquad 1260, 1518, 348 \tag{30}
\end{aligned}$$

$$\begin{aligned}
& \textcolor{red}{> } length(X3) \\
& \qquad \qquad \qquad 28650173028 \tag{31}
\end{aligned}$$
