# Supplementary material for: Poincare function for moduli of differential-geometric structures
Source: arXiv:1802.01322 source file (2018-02-05)
Supplement: Supplementary file 3 [file BK-2016-Poincare.pdf]

## 1. Second ord ODEs mod point

$$\begin{aligned}
 &> HR5 := 3 : HR := k \rightarrow \frac{k(k-1)}{2} - 4 : \\
 &> simplify\left( expand\left( HR5 \cdot z^5 + \sum_{k=6}^{\infty} HR(k) \cdot z^k \right) \right) \\
 &\quad - \frac{z^5 (3 z^3 - 7 z^2 + 2 z + 3)}{(z-1)^3}
 \end{aligned} \tag{1}$$

### 1a. Second ord ODEs cubic in p=y' (2D projective connections) mod point

$$\begin{aligned}
 &> HR := k \rightarrow 2(k-1) : \\
 &> simplify\left( expand\left( \sum_{k=4}^{\infty} HR(k) \cdot z^k \right) \right) \\
 &\quad - \frac{2 z^4 (2 z - 3)}{(z-1)^2}
 \end{aligned} \tag{2}$$

### 1b. Second ord ODEs of Lie type mod point

$$\begin{aligned}
 &> HR4 := 2 : HR := k \rightarrow (k-1) : \\
 &> simplify\left( expand\left( HR4 \cdot z^4 + \sum_{k=5}^{\infty} HR(k) \cdot z^k \right) \right) \\
 &\quad - \frac{z^4 (z^2 - 2)}{(z-1)^2}
 \end{aligned} \tag{3}$$

>

## 2. The space of germs of Riemannian metric is given by the following Hilbert polynomial

$$\begin{aligned}
 &> RF := k \rightarrow factor(expand(binomial(n+1, 2) \cdot binomial(n+k-1, k))) : \\
 &> seq(RF(k), k=0..5) \\
 &\quad \frac{1}{2} n(n+1), \frac{1}{2} n^2(n+1), \frac{1}{4} n^2(n+1)^2, \frac{1}{12} n^2(n+2)(n+1)^2, \frac{1}{48} n^2(n+2)(n \\
 &\quad + 3)(n+1)^2, \frac{1}{240} n^2(n+4)(n+3)(n+2)(n+1)^2
 \end{aligned} \tag{4}$$

Let us compute the Hilbert polynomial and the Poincare function of the space of moduli of Riemannian metrics

$$\begin{aligned}
 &> HR2 := factor\left( \frac{1}{2} n^2(n+1) \cdot \left( \frac{n+1}{2} - \frac{n+2}{3} \right) - \frac{n(n-1)}{2} \right) \\
 &\quad HR2 := \frac{1}{12} n(n-1)(-2+n)(n+3)
 \end{aligned} \tag{5}$$

$$\begin{aligned}
 &> HR := k \rightarrow factor\left( expand\left( \frac{n(n+1)}{2} \cdot binomial(n+k-1, k) - n \cdot binomial(n+k, k \right. \right. \\
 &\quad \left. \left. + 1) \right) \right) : \\
 &> factor(HR(0) + HR(1) + HR(2)) \\
 &\quad \frac{1}{12} n(n-1)(-2+n)(n+3)
 \end{aligned} \tag{6}$$

$$\begin{aligned}
 &> seq(HR(k), k=3..6) \\
 &\quad \frac{1}{24} n^2(n-1)(n+2)(n+1), \frac{1}{80} n^2(n-1)(n+3)(n+2)(n+1), \frac{1}{360} n^2(n \\
 &\quad - 1)(n+4)(n+3)(n+2)(n+1), \frac{1}{2016} n^2(n-1)(n+5)(n+4)(n+3)(n
 \end{aligned} \tag{7}$$

$$\begin{aligned} &> PR := \text{simplify}\left(\text{expand}\left(HR2 \cdot z^2 + \sum_{k=3}^{\infty} HR(k) \cdot z^k\right)\right) \\ PR &:= \frac{1}{2} \frac{(-z^3 n + (1-z)^{-n} z n + z^3 + (1-z)^{-n} z + z n - 2(1-z)^{-n} - z + 2) n}{z} \end{aligned} \quad (8)$$

$$\begin{aligned}
&> HR2 := 9 : HR := k \rightarrow \frac{1}{6} (k-1) (k^2 + 25k + 36) : \\
&> simplify \left( expand \left( HR2 \cdot z^2 + \sum_{k=3}^{\infty} HR(k) \cdot z^k \right) \right) \\
&\quad - \frac{z^2 (6z^4 - 24z^3 + 30z^2 - 4z - 9)}{(z-1)^4} \tag{15}
\end{aligned}$$

2c. The space of germs of Kahlerian metric is given by the following Hilbert polynomial

$$\begin{aligned}
&> KF := k \rightarrow factor(expand(binomial(2n+k+1, 2n-1) - 2 \cdot binomial(n+k+1, n-1))) : \\
&> seq(KF(k), k=0..6) \\
&n^2, n^2(n+1), \frac{1}{12} n^2(7n+11)(n+1), \frac{1}{12} n^2(3n+5)(n+2)(n+1), \frac{1}{360} n^2(n+1)(n+2)(31n^2+132n+137), \\
&\quad \frac{1}{120} n^2(3n+7)(n+3)(n+1)(n+2)^2, \\
&\quad \frac{1}{20160} n^2(n+3)(n+2)(n+1)(127n^3+1002n^2+2573n+2178) \tag{16}
\end{aligned}$$

Let us compute the Hilbert polynomial and the Poincare function of the space of moduli of Kahler metrics

$$\begin{aligned}
&> HK2 := factor \left( \frac{1}{12} n^2(7n+11)(n+1) - 2 \cdot \frac{n^2(n+1)(n+2)}{6} - n^2 \right) \\
&\quad HK2 := \frac{1}{4} n^2(n+3)(n-1) \tag{17}
\end{aligned}$$

$$\begin{aligned}
&> HK := k \rightarrow factor(expand(binomial(2n+k+1, 2n-1) - 2 \cdot binomial(n+k+1, n-1) - 2n \cdot binomial(n+k, n-1))) : \\
&> factor(HK(0) + HK(1) + HK(2)) \\
&\quad \frac{1}{4} n^2(n+3)(n-1) \tag{18}
\end{aligned}$$

$$\begin{aligned}
&> seq(HK(k), k=3..8) \\
&\frac{1}{6} n^2(n+2)(n+1)^2, \frac{1}{72} n^2(5n+13)(n+2)(n+1)^2, \frac{1}{180} n^2(4n+11)(n+3)(n+2)(n+1)^2, \\
&\quad \frac{1}{2880} n^2(17n+58)(n+2)(n+3)^2(n+1)^2, \\
&\quad \frac{1}{30240} n^2(n+4)(n+3)(n+2)(41n^2+269n+446)(n+1)^2, \frac{1}{604800} n^2(n+4)(n+3)(n+2)(167n^3+1868n^2+6947n+8658)(n+1)^2 \tag{19}
\end{aligned}$$

$$\begin{aligned}
&> seq(subs(n=1, KF(k)), k=0..8); seq(subs(n=1, HK(k)), k=3..8) \\
&\quad 1, 2, 3, 4, 5, 6, 7, 8, 9 \\
&\quad 2, 3, 4, 5, 6, 7 \tag{20}
\end{aligned}$$

$$\begin{aligned}
&> PK := simplify \left( expand \left( HK2 \cdot z^2 + \sum_{k=3}^{\infty} HK(k) \cdot z^k \right) \right) \\
&\quad PK := - \frac{z^4 n^2 - z^2 n^2 + 2(1-z)^{-n} z n - 2 z n + 2(1-z)^{-n} - (1-z)^{-2n} - 1}{z^2} \tag{21}
\end{aligned}$$

$$\begin{aligned}
&> factor(z^4 n^2 - z^2 n^2 - 2 z n - 1) \\
&\quad (n z^2 + n z + 1) (n z^2 - n z - 1) \tag{22}
\end{aligned}$$

$$\begin{aligned} &> \text{simplify}\left(-\frac{z^4 n^2 - z^2 n^2 + 2(1-z)^{-n} z n - 2 z n + 2(1-z)^{-n} - (1-z)^{-2n} - 1}{z^2}\right. \\ &\quad \left.- \left(\frac{1}{z^2 (1-z)^{2n}} - \frac{2(zn+1)}{z^2 (1-z)^n} + n^2(1-z^2) + \frac{2zn+1}{z^2}\right)\right) \\ &\quad 0 \end{aligned} \quad (23)$$

2d. The space of germs of hyper-Kahlerian metric is given by the following Hilbert polynomial

$$\begin{aligned} &> HF0 := 2n^2 + n : \\ &> HF := k \rightarrow \text{factor}\left(\text{expand}\left(2 \cdot \left(\sum_{i=0}^n \text{binomial}(2n+k-i, k) \cdot (n-i)\right) + \text{binomial}(2n+k\right.\right. \\ &\quad \left.\left.+ 1, k+2) - 2 \cdot \text{binomial}(n+k+1, k+2)\right)\right) : \\ &> \text{seq}(HF(k), k=1..8) \\ &\frac{4}{3} n (n+1) (2n+1), \frac{1}{2} (2n+3) (2n+1) (n+1) n, \frac{4}{15} n (2n+3) (2n+1) (n \\ &\quad + 2) (n+1), \frac{1}{18} (2n+5) (2n+3) (2n+1) (n+2) (n+1) n, \frac{2}{105} n (2n \\ &\quad + 5) (2n+3) (2n+1) (n+3) (n+2) (n+1), \frac{1}{360} (2n+7) (2n+5) (2n \\ &\quad + 3) (2n+1) (n+3) (n+2) (n+1) n, \frac{2}{2835} n (2n+7) (2n+5) (2n \\ &\quad + 3) (2n+1) (n+4) (n+3) (n+2) (n+1), \frac{1}{12600} (2n+9) (2n+7) (2n \\ &\quad + 5) (2n+3) (2n+1) (n+4) (n+3) (n+2) (n+1) n \end{aligned} \quad (24)$$

Let us compute the Hilbert polynomial and the Poincare function of the space of moduli of hyper-Kahler metrics

$$\begin{aligned} &> HK := k \rightarrow \text{factor}\left(\text{expand}\left(2 \cdot \left(\sum_{i=0}^n \text{binomial}(2n+k-i, k) \cdot (n-i)\right) - \text{binomial}(2n+k\right.\right. \\ &\quad \left.\left.+ 1, k+2) - 2 \cdot \text{binomial}(n+k+1, k+2)\right)\right) : \\ &> HK2 := \text{factor}(HK(0) + HK(1) + HK(2)) \\ &\quad HK2 := \frac{1}{6} n (2n+1) (n+3) (2n-1) \end{aligned} \quad (25)$$

$$\begin{aligned} &> \text{seq}(HK(k), k=3..7) \\ &\frac{2}{15} n (2n+3) (2n+1) (n+2) (n+1), \frac{1}{30} (2n+5) (2n+3) (2n+1) (n \\ &\quad + 2) (n+1) n, \frac{4}{315} n (2n+5) (2n+3) (2n+1) (n+3) (n+2) (n+1), \\ &\quad \frac{1}{504} (2n+7) (2n+5) (2n+3) (2n+1) (n+3) (n+2) (n+1) n, \\ &\quad \frac{1}{1890} n (2n+7) (2n+5) (2n+3) (2n+1) (n+4) (n+3) (n+2) (n+1) \end{aligned} \quad (26)$$

$$\begin{aligned} &> PH := \text{simplify}\left(\text{expand}\left(HK2 \cdot z^2 + \sum_{k=3}^{\infty} HK(k) \cdot z^k\right)\right) \end{aligned} \quad (27)$$

$$PH := -\frac{1}{(-1+z)z^2} (2z^5n^2 - 2z^4n^2 + nz^5 - 2n^2z^3 - nz^4 + 2z^2n^2 - nz^3 + 2z(1-z) \quad (27)$$

$$^{-2n}n - 3nz^2 + 3z(1-z)^{-2n} + 4zn - 3(1-z)^{-2n} - 3z + 3)$$

$$\begin{aligned} &> \text{simplify}\left(PH - \frac{2nz + 3z - 3}{z^2} \cdot \frac{1}{(1-z)^{2n+1}}\right) \\ &\quad - \frac{2n^2z^4 + nz^4 - 2n^2z^2 - nz^2 - 4nz - 3}{z^2} \end{aligned} \quad (28)$$

### 3. The space of germs of general connections (n>2)

$$> FG := k \rightarrow \text{factor}(\text{expand}(n^3 \cdot \text{binomial}(n+k-1, k))) :$$

$$> \text{seq}(FG(k), k=0..6)$$

$$\begin{aligned} &n^3, n^4, \frac{1}{2}n^4(n+1), \frac{1}{6}n^4(n+1)(n+2), \frac{1}{24}n^4(n+3)(n+2)(n+1), \frac{1}{120}n^4(n \\ &\quad + 4)(n+3)(n+2)(n+1), \frac{1}{720}n^4(n+5)(n+4)(n+3)(n+2)(n+1) \end{aligned} \quad (29)$$

Let us compute the Hilbert polynomial and the Poincare function of the space of moduli of general connections, n>2

$$\begin{aligned} &> HG0 := \text{factor}\left(n^3 - \frac{1}{2}n^2(n+1) - n^2\right) \\ &\quad HG0 := \frac{1}{2}n^2(n-3) \end{aligned} \quad (30)$$

$$> HG := k \rightarrow \text{factor}(\text{expand}(n^3 \cdot \text{binomial}(n+k-1, k) - n \cdot \text{binomial}(n+k+1, k+2))) :$$

$$> \text{seq}(HG(k), k=1..8)$$

$$\begin{aligned} &\frac{1}{6}n^2(5n+2)(n-1), \frac{1}{24}n^2(n-1)(11n+6)(n+1), \frac{1}{120}n^2(n-1)(19n \\ &\quad + 12)(n+2)(n+1), \frac{1}{720}n^2(29n+20)(n-1)(n+3)(n+2)(n+1), \\ &\quad \frac{1}{5040}n^2(n-1)(41n+30)(n+4)(n+3)(n+2)(n+1), \frac{1}{40320}n^2(n \\ &\quad - 1)(55n+42)(n+5)(n+4)(n+3)(n+2)(n+1), \frac{1}{362880}n^2(n \\ &\quad - 1)(71n+56)(n+6)(n+5)(n+4)(n+3)(n+2)(n+1), \frac{1}{3628800}n^2(n \\ &\quad - 1)(89n+72)(n+7)(n+6)(n+5)(n+4)(n+3)(n+2)(n+1) \end{aligned} \quad (31)$$

$$\begin{aligned} &> PH := \text{factor}\left(\text{expand}\left(HG0 + \sum_{k=1}^{\infty} HG(k) \cdot z^k\right)\right) \\ &\quad PH := \frac{4(n+1)(5n+2)((1-z)^n z^2 n - z^2 n^2 - (1-z)^n z n - (1-z)^n + 1)n}{(1-z)^n z^2 (5n+3 + \sqrt{5n^2+2n+1})(-5n-3 + \sqrt{5n^2+2n+1})} \end{aligned} \quad (32)$$

$$\begin{aligned} &> \text{factor}(\text{expand}((5n+3 + \sqrt{5n^2+2n+1})(-5n-3 + \sqrt{5n^2+2n+1}))) \\ &\quad - 4(n+1)(5n+2) \end{aligned} \quad (33)$$

$$\begin{aligned} &> PH := \frac{((1-z)^n(zn+1-z^2n) + z^2n^2 - 1)n}{(1-z)^n z^2} \\ &\quad PH := \frac{((-z+1)^n(-nz^2+nz+1) + n^2z^2 - 1)n}{(-z+1)^n z^2} \end{aligned} \quad (34)$$

For n=2

$$\begin{aligned} &> PH := factor \left( expand \left( 6z + \sum_{k=2}^{\infty} subs(n=2, HG(k)) \cdot z^k \right) \right) \\ &PH := -\frac{2z(z^2 - z - 3)}{(z-1)^2} \end{aligned} \quad (35)$$

$$\begin{aligned} &> simplify(expand(subs(n=2, HG(k)))) \\ &6k + 2 \end{aligned} \quad (36)$$

$$\begin{aligned} &> PH := simplify \left( \frac{2((1-z)^2(2z+1-z^2-z^3) + 4z^2-1)}{(1-z)^2 z^2} \right) \\ &PH := -\frac{2z(z^2 - z - 3)}{(z-1)^2} \end{aligned} \quad (37)$$

3a. Let us compute the Poincare function of the space of moduli of symmetric connections. First  $n > 2$ :

$$\begin{aligned} &> HG0 := simplify \left( \frac{n^2(n+1)}{2} - \frac{n^2(n+1)}{2} \right) \\ &HG0 := 0 \end{aligned} \quad (38)$$

$$\begin{aligned} &> HG1 := factor \left( \frac{n^3(n+1)}{2} - n^2 - \frac{n^2(n+1)(n+2)}{6} \right) \\ &HG1 := \frac{1}{3} n^2 (n-2) (n+2) \end{aligned} \quad (39)$$

$$\begin{aligned} &> HG := k \rightarrow factor \left( expand \left( \frac{n^2(n+1)}{2} \cdot \text{binomial}(n+k-1, k) - n \cdot \text{binomial}(n+k+1, k \right. \right. \\ &\quad \left. \left. + 2) \right) \right) : \\ &> PH := factor \left( expand \left( HG0 + HG1 \cdot z + \sum_{k=2}^{\infty} HG(k) \cdot z^k \right) \right) \\ &PH := -\frac{1}{2} \frac{(2(-z+1)^n z^3 n - n^2 z^2 - 2(-z+1)^n z n - n z^2 - 2(-z+1)^n + 2) n}{(-z+1)^n z^2} \end{aligned} \quad (40)$$

$$\begin{aligned} &> simplify \left( PH - \frac{n \cdot (n(n+1)z^2 - 2)}{2z^2} \cdot \frac{1}{(1-z)^n} - \frac{n(1+nz(1-z^2))}{z^2} \right) \\ &0 \end{aligned} \quad (41)$$

For  $n=2$

$$\begin{aligned} &> HG0 := simplify(6 \cdot 1 - 2 \cdot 3) \\ &HG0 := 0 \end{aligned} \quad (42)$$

$$\begin{aligned} &> HG1 := simplify(6 \cdot 2 - 2 \cdot 2 - 2 \cdot 4 + 1) \\ &HG1 := 1 \end{aligned} \quad (43)$$

$$\begin{aligned} &> HG2 := simplify(6 \cdot 3 - 2 \cdot 5 - 1) \\ &HG2 := 7 \end{aligned} \quad (44)$$

$$\begin{aligned} &> HG := k \rightarrow simplify(6 \cdot (k+1) - 2 \cdot (k+3)) \\ &HG := k \rightarrow simplify(4k) \end{aligned} \quad (45)$$

$$\begin{aligned} &> PH := simplify \left( HG1 \cdot z + HG2 \cdot z^2 + \sum_{k=3}^{\infty} HG(k) \cdot z^k \right) \\ &PH := -\frac{z(z^3 + z^2 - 5z - 1)}{(z-1)^2} \end{aligned} \quad (46)$$

$$\begin{aligned} &> \text{series}(PH, z=0, 7) \\ & \quad z + 7z^2 + 12z^3 + 16z^4 + 20z^5 + 24z^6 + O(z^7) \end{aligned} \quad (47)$$

3b. Let us compute the Poincare function of the space of moduli of metric connections.

At first incorrect count when both (g,T) are of the same order wrt G-action

$$\begin{aligned} &> HG := k \rightarrow \text{factor} \left( \text{expand} \left( \frac{n(n^2+1)}{2} \cdot \text{binomial}(n+k-1, k) - n \cdot \text{binomial}(n+k, k+1) \right) \right) : \\ &> \text{seq}(HG(k), k=0..4) \\ & \quad \frac{1}{2} n(n-1)^2, \frac{1}{2} n^3(n-1), \frac{1}{12} n^2(n-1)(3n+1)(n+1), \frac{1}{24} n^2(n-1)(2n+1)(n+2)(n+1), \\ & \quad \frac{1}{240} n^2(n-1)(5n+3)(n+3)(n+2)(n+1) \end{aligned} \quad (48)$$

$$\begin{aligned} &> PH := \text{factor} \left( \text{expand} \left( \sum_{k=0}^{\infty} HG(k) \cdot z^k \right) \right) \\ & \quad PH := \frac{1}{2} \frac{(n^2 z + 2(-z+1)^n + z - 2)n}{(-z+1)^n z} \end{aligned} \quad (49)$$

Now the correct "staggered" jet-approach: for 0-jets as before; for k-jets with k>0 the k-jet of the structure consists of (k+1)-jet of g and k-jet of T

$$\begin{aligned} &> \text{simplify} \left( \frac{n(n^2+1)}{2} - \frac{n(n+1)}{2} - \frac{n^2(n-1)}{2} \right), \text{factor} \left( \frac{n(n^2+1)}{2} - n^2 \right), \\ & \quad \text{factor} \left( \frac{n(n+1)}{2} + n^3 - n^2 - \frac{n \cdot n(n+1)}{2} \right) \\ & \quad 0, \frac{1}{2} n(n-1)^2, \frac{1}{2} n(n-1)^2 \end{aligned} \quad (50)$$

$$> HG0 := \frac{1}{2} n(n-1)^2 :$$

$$\begin{aligned} &> HG := k \rightarrow \text{factor} \left( \text{expand} \left( \frac{n(n+1)}{2} \cdot \text{binomial}(n+k, k+1) + \frac{n^2(n-1)}{2} \cdot \text{binomial}(n+k-1, k) - n \cdot \text{binomial}(n+k+1, k+2) \right) \right) : \\ &> \text{seq}(HG(k), k=0..4) \\ & \quad \frac{1}{2} n^2(n-1), \frac{1}{12} n^2(7n+1)(n-1), \frac{1}{24} n^2(n-1)(7n+2)(n+1), \frac{1}{240} n^2(n-1)(23n+9)(n+2)(n+1), \\ & \quad \frac{1}{720} n^2(n-1)(17n+8)(n+3)(n+2)(n+1) \\ &> PH := \text{factor} \left( \text{expand} \left( HG0 + \sum_{k=1}^{\infty} HG(k) \cdot z^k \right) \right) \\ & \quad PH := -\frac{1}{2} \frac{1}{(-z+1)^n z^2} (n((-z+1)^n z^2 n - n^2 z^2 - z(-z+1)^n n - (-z+1)^n z^2 + n z^2 \\ & \quad + z(-z+1)^n - z n - 2(-z+1)^n - z + 2)) \end{aligned} \quad (51)$$

$$\begin{aligned} &> \text{simplify} \left( \text{expand} \left( \frac{n - \text{binomial}(n, 2)(z^2 - z)}{z^2} - \frac{n(2 - (n+1)z - n(n-1)z^2)}{2z^2(1-z)^n} \right) \right) \end{aligned} \quad (52)$$





$$> \text{simplify}(\text{expand}(\text{subs}(n=1, HG(k)))) \quad (61)$$

$$> PH := \text{factor}\left(\text{expand}\left(HG1 \cdot z + HG2 \cdot z^2 + \sum_{k=3}^{\infty} HG(k) \cdot z^k\right)\right)$$

$$PH := \frac{8}{3} \left( (2n^2 + 4n + 3) (38n^2 + 67n + 30) (6n^2 (-z + 1)^n)^2 z^4 \right. \\ \left. + 3n ((-z + 1)^n)^2 z^4 - 6n^2 ((-z + 1)^n)^2 z^2 - 4n^3 z^3 - 3n ((-z + 1)^n)^2 z^2 - 6n^2 z^3 \right. \\ \left. - 6n ((-z + 1)^n)^2 z - 2n z^3 - 3(((-z + 1)^n)^2 + 3) \right) / \left( ((-z + 1)^n)^2 z^3 (24n^2 \right. \\ \left. + \sqrt{-32n^4 + 16n^3 + 64n^2 + 24n + 9} + 48n + 27) (-24n^2 - 48n - 27 \right. \\ \left. + \sqrt{-32n^4 + 16n^3 + 64n^2 + 24n + 9}) \right) \quad (62)$$

$$> \text{factor}(-32n^4 + 16n^3 + 64n^2 + 24n + 9 - (24n^2 + 48n + 27)^2) \\ - 8(2n^2 + 4n + 3)(38n^2 + 67n + 30) \quad (63)$$

$$> PHh := \frac{1}{3} \frac{1}{(1-z)^{2n} z^3} \left( ((1-z)^{2n} (6n^2 z^4 + 3n z^4 - 6n^2 z^2 - 3n z^2 - 6n z - 3) \right. \\ \left. - 4n^3 z^3 - 6n^2 z^3 - 2n z^3 + 3) \right) : \\ PH := \frac{1 + 2nz - n(2n+1)z^2(z^2-1)}{z^3} + \frac{2n(2n^2+3n+1)z^3-3}{3z^3(1-z)^{2n}} : \text{simplify}(PH \\ - PHh) \quad (64)$$

$$> \text{seq}(\text{series}(\text{simplify}(PH), z=0, 4), n=2..4) \\ 35z + 144z^2 + 316z^3 + O(z^4), 189z + 924z^2 + 2674z^3 + O(z^4), 594z + 3528z^2 \\ + 12684z^3 + O(z^4) \quad (65)$$

For n=1 (i.e. dim(M)=2n=2)

$$> HG0 := 0 : HG1 := 1 : HG2 := 5 : HG := k \rightarrow 3k :$$

$$> PH := \text{factor}\left(\text{expand}\left(HG1 \cdot z + HG2 \cdot z^2 + \sum_{k=3}^{\infty} HG(k) \cdot z^k\right)\right) \\ PH := -\frac{z(z^3 - 3z - 1)}{(z-1)^2} \quad (66)$$

$$> \text{series}(PH, z=0, 4) \\ z + 5z^2 + 9z^3 + O(z^4) \quad (67)$$

3d. Let us compute the Poincare function of the space of moduli of projective connections

$$> \text{factor}\left(\frac{n^2(n+1)}{2} - n\right) \\ \frac{1}{2} n(n+2)(n-1) \quad (68)$$

$$> HG := k \rightarrow \text{factor}\left(\text{expand}\left(\frac{n(n+2)(n-1)}{2} \cdot \text{binomial}(n+k-1, k) - n \cdot \text{binomial}(n+k \right. \right. \\ \left. \left. + 1, k+2)\right)\right) :$$

$$> \text{seq}(\text{factor}(\text{expand}(\text{binomial}(n+k+1, k+2))), k=0..3) \\ \frac{1}{2} n(n+1), \frac{1}{6} n(n+1)(n+2), \frac{1}{24} n(n+3)(n+2)(n+1), \frac{1}{120} n(n+4)(n \\ + 3)(n+2)(n+1) \quad (69)$$

$$\begin{aligned}
&> HG0 := HG(0) + n; HG1 := factor(HG(1) - n^2); HG2 := factor(HG(2) - n); \\
&\quad HG0 := 0 \\
&\quad HG1 := \frac{1}{3} n^2 (n^2 - 7) \\
&\quad HG2 := \frac{1}{24} n (n - 2) (5 n^3 + 16 n^2 + 15 n + 12)
\end{aligned} \tag{70}$$

$$\begin{aligned}
&> PH := factor\left(\exp\left(HG1 \cdot z + HG2 \cdot z^2 + \sum_{k=3}^{\infty} HG(k) \cdot z^k\right)\right) \\
PH &:= (4 (9 n^2 + 3 n - 32) (n^2 + n - 4) (2 n z^3 (-z + 1)^n + 2 (-z + 1)^n z^4 - n^2 z^2 \\
&\quad - 2 n (-z + 1)^n z - 2 (-z + 1)^n z^2 - n z^2 + 2 z^2 - 2 (-z + 1)^n + 2) n) / ((-z \\
&\quad + 1)^n z^2 (-9 n^2 - 5 n + 32 + \sqrt{n (9 n^3 - 6 n^2 - 31 n + 32)}) (9 n^2 \\
&\quad + \sqrt{n (9 n^3 - 6 n^2 - 31 n + 32)} + 5 n - 32))
\end{aligned} \tag{71}$$

$$\begin{aligned}
&> factor(n (9 n^3 - 6 n^2 - 31 n + 32) - (9 n^2 + 5 n - 32)^2) \\
&\quad - 8 (9 n^2 + 3 n - 32) (n^2 + n - 4)
\end{aligned} \tag{72}$$

$$\begin{aligned}
&> PH := \frac{n ((n + 2) (n - 1) z^2 - 2)}{2 z^2 (1 - z)^n} - n \left( z^2 + n z - 1 - \frac{z n + 1}{z^2} \right) : \\
&> seq\left(simplify\left(HG1 \cdot z + HG2 \cdot z^2 + \sum_{k=3}^{\infty} HG(k) \cdot z^k - \left( \frac{n ((n + 2) (n - 1) z^2 - 2)}{2 z^2 (1 - z)^n} - n \left( z^2 \right. \right. \right. \\
&\quad \left. \left. \left. + n z - 1 - \frac{z n + 1}{z^2} \right) \right) \right), n = 3..9) \\
&\quad 0, 0, 0, 0, 0, 0, 0
\end{aligned} \tag{73}$$

For n=2

$$\begin{aligned}
&> factor(expand(subs(n=2, HG1))), factor(expand(subs(n=2, HG2))), \\
&\quad factor(expand(subs(n=2, HG(3)))) , factor(expand(subs(n=2, HG(4)))) \\
&\quad -4, 0, 4, 6
\end{aligned} \tag{74}$$

$$> HG0 := 0 : HG1 := 0 : HG2 := 0 : HG3 := 0 : HG := k \rightarrow 2 (k - 1) :$$

$$\begin{aligned}
&> PH := factor\left(\exp\left(\sum_{k=4}^{\infty} HG(k) \cdot z^k\right)\right) \\
PH &:= -\frac{2 z^4 (2 z - 3)}{(z - 1)^2}
\end{aligned} \tag{75}$$

$$\begin{aligned}
&> series(PH, z=0, 7) \\
&\quad 6 z^4 + 8 z^5 + 10 z^6 + O(z^7)
\end{aligned} \tag{76}$$

4. Let us compute the Poincare function of the space of moduli of conformal connections, n>3.

$$\begin{aligned}
&> factor\left(\frac{1}{2} \cdot \frac{n (n - 1)}{2} \cdot \left(\frac{n (n - 1)}{2} + 1\right) - \frac{n (n - 1) (n - 2) (n - 3)}{24} - \frac{n (n + 1)}{2}\right) \\
&\quad \frac{1}{12} n (n - 3) (n + 2) (n + 1)
\end{aligned} \tag{77}$$

$$\begin{aligned}
&> factor\left(\frac{1}{2} \cdot \frac{n (n - 1)}{2} \cdot \left(\frac{n (n - 1)}{2} + 1\right) - \frac{n (n - 1) (n - 2) (n - 3)}{24} - \frac{n (n + 1)}{2} \right. \\
&\quad \left. - \frac{n (n - 1)}{2}\right) - 1
\end{aligned} \tag{78}$$

$$\frac{1}{12} n^2 (n^2 - 13) - 1 \quad (78)$$

$$> \text{simplify}\left(1 + n + \frac{n(n+1)}{2} - \frac{(n+1)(n+2)}{2}\right) \quad (79)$$

$$> \text{factor}\left(\left(\frac{n(n+1)}{2} - 1\right) \cdot \frac{(n+1)(n+2)}{2} - n \cdot \left(\frac{(n+1)(n+2)(n+3)}{6} - 1\right) + n\right) \quad (80)$$

$$\frac{1}{12} n^4 - \frac{13}{12} n^2 - 1$$

$$> HG2 := \frac{n^4 - 13n^2 - 12}{12} : HG3 := \text{factor}\left(\left(\frac{n(n+1)}{2} - 1\right) \cdot \frac{n(n+1)(n+2)}{6} - n \cdot \frac{n(n+1)(n+2)(n+3)}{24} - n\right) \quad (81)$$

$$HG3 := \frac{1}{24} n (n^4 + 2n^3 - 5n^2 - 14n - 32)$$

$$> HG := k \rightarrow \left(\frac{n(n+1)}{2} - 1\right) \cdot \text{binomial}(n+k-1, k) - n \cdot \text{binomial}(n+k, k+1) :$$

$$> PH := \text{factor}\left(\text{expand}\left(HG2 \cdot z^2 + HG3 \cdot z^3 + \sum_{k=4}^{\infty} HG(k) \cdot z^k\right)\right)$$

$$PH := -\frac{1}{2} \frac{1}{(-z+1)^n z} \left( (-z+1)^n z^3 n^2 + 2(-z+1)^n z^4 n - (-z+1)^n z^3 n - z(-z+1)^n n^2 - 2(-z+1)^n z^2 n + 2(-z+1)^n z^3 + z(-z+1)^n n - n^2 z - 2(-z+1)^n n - 2z(-z+1)^n - zn + 2n + 2z \right) \quad (82)$$

$$> \text{simplify}\left(\text{expand}\left(\frac{\text{binomial}(n+1, 2)}{(1-z)^n} - \frac{(n+z)}{z(1-z)^n} + n \left(\frac{1}{z} + z - z^3\right) + (\text{binomial}(n, 2) + 1)(1-z^2) - PH\right)\right) \quad (83)$$

$$0$$

For n=3

$$> HG3 := 1 : HG4 := 9 : HG := k \rightarrow k^2 - 4 :$$

$$> PH := \text{factor}\left(HG3 \cdot z^3 + HG4 \cdot z^4 + \sum_{k=5}^{\infty} HG(k) \cdot z^k\right) \quad (84)$$

$$PH := -\frac{z^3(z+1)(3z^3 - 8z^2 + 5z + 1)}{(z-1)^3}$$

$$> \text{expand}((z+1)(3z^3 - 8z^2 + 5z + 1)) \quad (85)$$

$$3z^4 - 5z^3 - 3z^2 + 6z + 1$$

$$> \text{simplify}\left(\text{expand}\left(\frac{n(k-1)}{2} \cdot \text{binomial}(n+k-1, k+1) - \text{binomial}(n+k-1, k) - \left(\frac{n(n+1)}{2} - 1\right) \cdot \text{binomial}(n+k-1, k) + n \cdot \text{binomial}(n+k, k+1)\right)\right) \quad (86)$$

$$0$$

>

4a. Let us compute the Poincare function of the space of Weyl conformal connections (n>2)

$$\begin{aligned}
& > HG0 := 0 : HG1 := factor\left( expand\left( \frac{n^2 (n^2 - 1)}{12} + \text{binomial}(n, 2) - \text{binomial}(n, 2) \right. \right. \\
& \quad \left. \left. - 1 \right) \right) \\
& \quad \quad \quad HG1 := \frac{1}{12} (n - 2) (n + 2) (n^2 + 3) \tag{87}
\end{aligned}$$

$$\begin{aligned}
& > HG1 := factor(expand((\text{binomial}(n + 1, 2) - 1) \cdot (1 + n + \text{binomial}(n + 1, 2)) + n \cdot (1 \\
& \quad + n) - n \cdot (n + \text{binomial}(n + 1, 2) + \text{binomial}(n + 2, 3)))) \\
& \quad \quad \quad HG1 := \frac{1}{12} (n - 2) (n + 2) (n^2 + 3) \tag{88}
\end{aligned}$$

$$\begin{aligned}
& > HG := k \rightarrow (\text{binomial}(n + 1, 2) - 1) \cdot \text{binomial}(n + k, k + 1) + n \cdot \text{binomial}(n + k - 1, k) \\
& \quad - n \cdot \text{binomial}(n + k + 1, k + 2) : \\
& > factor(expand(HG(2))) \\
& \quad \quad \quad \frac{1}{24} n (n - 1) (n + 1) (n^2 + 2n + 8) \tag{89}
\end{aligned}$$

$$\begin{aligned}
& > factor(expand(HG(1) - \text{binomial}(n, 2) - 1)) \\
& \quad \quad \quad \frac{1}{12} (n - 2) (n + 2) (n^2 + 3) \tag{90}
\end{aligned}$$

$$\begin{aligned}
& > PH := factor\left( expand\left( HG1 \cdot z + \sum_{k=2}^{\infty} HG(k) \cdot z^k \right) \right) \\
& PH := -\frac{1}{2} \frac{1}{(-z + 1)^n z^2} \left( (-z + 1)^n z^3 n^2 - (-z + 1)^n z^3 n - (-z + 1)^n z n^2 + 2(-z \right. \\
& \quad + 1)^n z^3 + (-z + 1)^n z n - n^2 z - 2n z^2 - 2(-z + 1)^n n - 2(-z + 1)^n z - z n + 2n \\
& \quad \left. + 2z \right) \tag{91}
\end{aligned}$$

$$\begin{aligned}
& > simplify\left( \frac{n z^2 + \left( \frac{n^2 + n}{2} - 1 \right) z - n}{(1 - z)^n z^2} - \frac{\left( \frac{n^2 - n}{2} + 1 \right) z (z^2 - 1) - n}{z^2} - PH \right) \\
& \quad \quad \quad 0 \tag{92}
\end{aligned}$$

For n=2:

$$\begin{aligned}
& > HG0 := 0 : HG1 := 1 : HG2 := 3 : HG := k \rightarrow 2k : \\
& > PHn2 := factor\left( expand\left( HG1 \cdot z + HG2 \cdot z^2 + \sum_{k=3}^{\infty} HG(k) \cdot z^k \right) \right) \\
& \quad \quad \quad PHn2 := -\frac{z(z^3 - z^2 - z - 1)}{(z - 1)^2} \tag{93}
\end{aligned}$$

$$\begin{aligned}
& > simplify(subs(n = 2, PH) - PHn2) \\
& \quad \quad \quad z(z - 1) \tag{94}
\end{aligned}$$

4b. Let us compute the Poincare function of the space of Einstein-Weyl structures (n>3)

$$\begin{aligned}
& > HG0 := 0 : HG1 := factor\left( expand\left( \frac{n^2 (n^2 - 1)}{12} + \text{binomial}(n, 2) - (\text{binomial}(n + 1, 2) \right. \right. \\
& \quad \left. \left. - 1) - (\text{binomial}(n, 2) + 1) \right) \right) \\
& \quad \quad \quad HG1 := \frac{1}{12} n (n - 3) (n + 2) (n + 1) \tag{95}
\end{aligned}$$

$$> HG := k \rightarrow (\text{binomial}(n + 1, 2) - 1) \cdot \text{binomial}(n + k, k + 1) + n \cdot \text{binomial}(n + k - 1, k)$$

$$- (\text{binomial}(n+1, 2) - 1) \cdot \text{binomial}(n+k-2, k-1) - n \cdot \text{binomial}(n+k+1, k+2) :$$

$$\begin{aligned} &> \text{factor}(\text{expand}(\text{HG}(2))) \\ &\quad \frac{1}{24} n (n-1) (n-2) (n^2 + 5n + 8) \end{aligned} \quad (96)$$

$$\begin{aligned} &> PH := \text{factor}\left(\text{expand}\left(HG1 \cdot z + \sum_{k=2}^{\infty} HG(k) \cdot z^k\right)\right) \\ PH &:= -\frac{1}{2} \frac{1}{(-z+1)^n z^2} \left( (-z+1)^n z^3 n^2 - (-z+1)^n z^3 n + n^2 z^3 - z(-z+1)^n n^2 + 2(-z+1)^n z^3 + n z^3 + z(-z+1)^n n - n^2 z - 2n z^2 - 2z^3 - 2(-z+1)^n n - 2z(-z+1)^n - z n + 2n + 2z \right) \end{aligned} \quad (97)$$

$$\begin{aligned} &> \text{simplify}\left(\frac{n z^2 - \left(\frac{n^2+n}{2} - 1\right) z (z^2 - 1) - n}{(1-z)^n z^2} - \frac{\left(\frac{n^2-n}{2} + 1\right) z (z^2 - 1) - n}{z^2} - PH\right) \\ &\quad 0 \end{aligned} \quad (98)$$

For n=3:

$$> HG0 := 0 : HG1 := 1 : HG2 := 7 : HG := k \rightarrow 4k :$$

$$\begin{aligned} &> PHn3 := \text{factor}\left(\text{expand}\left(HG1 \cdot z + HG2 \cdot z^2 + \sum_{k=3}^{\infty} HG(k) \cdot z^k\right)\right) \\ PHn3 &:= -\frac{z(z^3 + z^2 - 5z - 1)}{(z-1)^2} \end{aligned} \quad (99)$$

$$\begin{aligned} &> \text{simplify}(\text{subs}(n=3, PH) - PHn3) \\ &\quad z(z-1) \end{aligned} \quad (100)$$

>

5. Let us compute the Poincare function of the space of moduli of almost complex structures on  $M^{2n}$ . First n>3:

$$\begin{aligned} &> \text{factor}\left(2 \cdot \frac{n(n-1)}{2} \cdot n - 2n^2\right), \text{factor}\left(2n^2 + 2n^2 \cdot 2n - 4n^2 - 2n \cdot \frac{2n(2n+1)}{2} + 2 \cdot \frac{n(n+1)}{2} \cdot n\right) \\ &\quad n^2(n-3), n^2(n-3) \end{aligned} \quad (101)$$

$$> HG1 := n^2(n-3) :$$

$$\begin{aligned} &> HG2 := \text{factor}\left(2n^2 \cdot \frac{2n(2n+1)}{2} - 2n \cdot \frac{2n(2n+1)(2n+2)}{6} - 2 \cdot \frac{n(n+1)}{2} \cdot n + 2 \cdot \frac{n(n+1)(n+2)}{6} \cdot n\right) \\ &\quad HG2 := \frac{1}{3} n^2 (5n^2 - 6n - 5) \end{aligned} \quad (102)$$

$$> HG := k \rightarrow \text{simplify}(2n^2 \cdot \text{binomial}(2n+k-1, k) - 2n \cdot \text{binomial}(2n+k, k+1) - 2n \cdot \text{binomial}(n+k-1, k) + 2n \cdot \text{binomial}(n+k, k+1)) :$$

$$\begin{aligned} &> HG(0) \\ &\quad -2n \end{aligned} \quad (103)$$

$$\begin{aligned} &> \text{simplify}(\text{expand}(HG1 - HG(1))), \text{simplify}(\text{expand}(HG2 - HG(2))) \\ &\quad 0, 0 \end{aligned} \quad (104)$$

$$\begin{aligned}
& > PH := \text{simplify}\left(HG1 \cdot z + \text{expand}\left(\sum_{k=2}^{\infty} HG(k) \cdot z^k\right)\right) \\
PH &:= \frac{1}{12} \frac{1}{z} \left( (n^3 z^2 - 12 n^2 z^2 + 24 z (-z+1)^{-2n} n + 29 n z^2 - 24 (-z+1)^{-n} z - 6 z^2 \right. \\
&\quad \left. - 24 (-z+1)^{-2n} + 24 (-z+1)^{-n} + 24 z) n \right)
\end{aligned} \tag{105}$$

$$\begin{aligned}
& > PH := \text{simplify}\left(HG1 \cdot z + \text{expand}\left(\sum_{k=2}^{\infty} HG(k) \cdot z^k\right)\right) \\
PH &:= \frac{2 (z (-z+1)^{-2n} n - (-z+1)^{-2n} + z + (-z+1)^{1-n}) n}{z}
\end{aligned} \tag{106}$$

$$\begin{aligned}
& > \text{simplify}\left(\left\{ \text{seq}\left(\frac{2 (zn-1) n}{z (1-z)^{2n}} + \frac{2 n}{z (1-z)^{n-1}} + 0 \cdot \frac{n (n-3) (n^2-9n+2) z}{12} + 2 n \right. \right. \right. \\
&\quad \left. \left. \left. - PH, n=4..10 \right) \right\} \right) \\
&\quad \{0\}
\end{aligned} \tag{107}$$

For n=3

$$\begin{aligned}
& > HG1 := 2 : HG2 := 64 : \\
& > \text{eval}\left(\frac{1}{3} n^2 (5 n^2 - 6 n - 5), n=3\right) \\
&\quad 66
\end{aligned} \tag{108}$$

$$\begin{aligned}
& > \text{seq}(\text{expand}(\text{subs}(n=3, HG(k))), k=1..5) \\
&\quad 0, 66, 282, 792, 1806
\end{aligned} \tag{109}$$

$$\begin{aligned}
& > HG := k \rightarrow \text{simplify}(18 \cdot \text{binomial}(k+5, k) - 6 \cdot \text{binomial}(k+6, k+1) - 6 \cdot \text{binomial}(k+2, \\
&\quad k) + 6 \cdot \text{binomial}(k+3, k+1)) : \\
& > \text{seq}(\text{expand}(\text{subs}(n=3, HG(k))), k=1..5) \\
&\quad 0, 66, 282, 792, 1806
\end{aligned} \tag{110}$$

$$\begin{aligned}
& > \text{simplify}(\text{expand}(HG2 - HG(2))) \\
&\quad -2
\end{aligned} \tag{111}$$

$$\begin{aligned}
& > PH := \text{simplify}\left(HG1 \cdot z + HG2 \cdot z^2 + \text{expand}\left(\sum_{k=3}^{\infty} HG(k) \cdot z^k\right)\right) \\
PH &:= - \frac{2 z (z^7 - 7 z^6 + 18 z^5 - 17 z^4 - 10 z^3 + 36 z^2 - 26 z - 1)}{(z-1)^6}
\end{aligned} \tag{112}$$

For n=2

$$\begin{aligned}
& > HG1 := 0 : HG2 := 2 : HG3 := 24 : HG4 := 60 : HG5 := 116 : \\
& > HG := k \rightarrow \text{simplify}(\text{expand}(8 \cdot \text{binomial}(k+3, k) - 4 \cdot \text{binomial}(k+4, k+1) + 4)) : \\
&\quad HG(k) \\
&\quad \frac{2}{3} k^3 + 2 k^2 - \frac{8}{3} k - 4
\end{aligned} \tag{113}$$

$$\begin{aligned}
& > \text{seq}(HG(k), k=1..6); \text{seq}(HG(k) - HG||k, k=1..5); \\
&\quad -4, 4, 24, 60, 116, 196 \\
&\quad -4, 2, 0, 0, 0
\end{aligned} \tag{114}$$

$$\begin{aligned}
& > PH := \text{simplify}\left(HG1 \cdot z + HG2 \cdot z^2 + HG3 \cdot z^3 + HG4 \cdot z^4 + HG5 \cdot z^5 + \text{expand}\left(\sum_{k=6}^{\infty} HG(k) \cdot z^k\right)\right) \\
PH &:= - \frac{2 z^2 (z^4 - 6 z^3 + 12 z^2 - 8 z - 1)}{(z-1)^4}
\end{aligned} \tag{115}$$

$$\left[ \begin{array}{l} \textcolor{red}{> } PH := simplify\left(HG1 \cdot z + HG2 \cdot z^2 + expand\left(\sum_{k=3}^{\infty} HG(k) \cdot z^k\right)\right) \\ PH := - \frac{2 \, z^2 \, (z^4 - 6 \, z^3 + 12 \, z^2 - 8 \, z - 1)}{(z - 1)^4} \end{array} \right. \quad (116)$$
