# Supplementary material for: Poincare function for moduli of differential-geometric structures
Source: arXiv:1802.01322 source file (2018-02-05)

> with(DifferentialGeometry) : with(JetCalculus) : with(Tools) :

> DGsetup([x, y], [u], J, 4) :

We consider the action of the Lie pseudogroup  $x \mapsto X(x, y)$ ,  $y \mapsto y + c$ ,  $u \mapsto u + c'$  in the general and some singular strata.

It is clear that the Lie Algebra Sheaf  $\{f(x, y) * D_x, D_y, D_u\}$  is bracket-closed, i.e. the bulk of brackets is  $(f, g) \rightarrow f_x * g - f * g_x$ , so

on the level of  $k$ -jets we get a finite-dimensional Lie algebra of vector fields (in involution) and the number of diff.inv = codimension.

> X4 := Prolong(evalDG(f(x, y) \* D\_x), 4)

$$\begin{aligned}
 X4 := & f(x, y) D_x - \left( \frac{\partial}{\partial x} f(x, y) \right) u_1 D_{u_1} - \left( \frac{\partial}{\partial y} f(x, y) \right) u_1 D_{u_2} - \left( \left( \frac{\partial^2}{\partial x^2} f(x, y) \right) u_1 \right. \\
 & + 2 \left( \frac{\partial}{\partial x} f(x, y) \right) u_{1,1} \left. \right) D_{u_{1,1}} - \left( \left( \frac{\partial^2}{\partial y \partial x} f(x, y) \right) u_1 + \left( \frac{\partial}{\partial y} f(x, y) \right) u_{1,1} \right. \\
 & + \left. \left( \frac{\partial}{\partial x} f(x, y) \right) u_{1,2} \right) D_{u_{1,2}} - \left( \left( \frac{\partial^2}{\partial y^2} f(x, y) \right) u_1 + 2 \left( \frac{\partial}{\partial y} f(x, y) \right) u_{1,2} \right) D_{u_{2,2}} \\
 & - \left( \left( \frac{\partial^3}{\partial x^3} f(x, y) \right) u_1 + 3 \left( \frac{\partial^2}{\partial x^2} f(x, y) \right) u_{1,1} + 3 \left( \frac{\partial}{\partial x} f(x, y) \right) u_{1,1,1} \right) D_{u_{1,1,1}} \\
 & - \left( \left( \frac{\partial^3}{\partial y \partial x^2} f(x, y) \right) u_1 + 2 \left( \frac{\partial^2}{\partial y \partial x} f(x, y) \right) u_{1,1} + \left( \frac{\partial^2}{\partial x^2} f(x, y) \right) u_{1,2} \right. \\
 & + \left. \left( \frac{\partial}{\partial y} f(x, y) \right) u_{1,1,1} + 2 \left( \frac{\partial}{\partial x} f(x, y) \right) u_{1,1,2} \right) D_{u_{1,1,2}} - \left( \left( \frac{\partial^3}{\partial y^2 \partial x} f(x, y) \right) u_1 \right. \\
 & + 2 \left( \frac{\partial^2}{\partial y \partial x} f(x, y) \right) u_{1,2} + \left( \frac{\partial^2}{\partial y^2} f(x, y) \right) u_{1,1} + 2 \left( \frac{\partial}{\partial y} f(x, y) \right) u_{1,1,2} \\
 & + \left. \left( \frac{\partial}{\partial x} f(x, y) \right) u_{1,2,2} \right) D_{u_{1,2,2}} - \left( \left( \frac{\partial^3}{\partial y^3} f(x, y) \right) u_1 + 3 \left( \frac{\partial^2}{\partial y^2} f(x, y) \right) u_{1,2} \right. \\
 & + 3 \left( \frac{\partial}{\partial y} f(x, y) \right) u_{1,2,2} \left. \right) D_{u_{2,2,2}} - \left( \left( \frac{\partial^4}{\partial x^4} f(x, y) \right) u_1 + 4 \left( \frac{\partial^3}{\partial x^3} f(x, y) \right) u_{1,1} \right. \\
 & + 6 \left( \frac{\partial^2}{\partial x^2} f(x, y) \right) u_{1,1,1} + 4 \left( \frac{\partial}{\partial x} f(x, y) \right) u_{1,1,1,1} \left. \right) D_{u_{1,1,1,1}} - \left( \left( \frac{\partial^4}{\partial y \partial x^3} f(x, y) \right) u_1 \right. \\
 & + 3 \left( \frac{\partial^3}{\partial y \partial x^2} f(x, y) \right) u_{1,1} + \left( \frac{\partial^3}{\partial x^3} f(x, y) \right) u_{1,2} + 3 \left( \frac{\partial^2}{\partial y \partial x} f(x, y) \right) u_{1,1,1} \\
 & + 3 \left( \frac{\partial^2}{\partial x^2} f(x, y) \right) u_{1,1,2} + \left( \frac{\partial}{\partial y} f(x, y) \right) u_{1,1,1,1} + 3 \left( \frac{\partial}{\partial x} f(x, y) \right) u_{1,1,1,2} \left. \right) \\
 & D_{u_{1,1,1,2}} - \left( \left( \frac{\partial^4}{\partial y^2 \partial x^2} f(x, y) \right) u_1 + 2 \left( \frac{\partial^3}{\partial y \partial x^2} f(x, y) \right) u_{1,2} + 2 \left( \frac{\partial^3}{\partial y^2 \partial x} f(x, y) \right) u_{1,1} \right. \\
 & + 4 \left( \frac{\partial^2}{\partial y \partial x} f(x, y) \right) u_{1,1,2} + \left( \frac{\partial^2}{\partial x^2} f(x, y) \right) u_{1,2,2} + \left( \frac{\partial^2}{\partial y^2} f(x, y) \right) u_{1,1,1} \\
 & + 2 \left( \frac{\partial}{\partial y} f(x, y) \right) u_{1,1,1,2} + 2 \left( \frac{\partial}{\partial x} f(x, y) \right) u_{1,1,2,2} \left. \right) D_{u_{1,1,2,2}} - \left( \left( \frac{\partial^4}{\partial y^3 \partial x} f(x, y) \right) u_1 \right. \\
 & + 3 \left( \frac{\partial^3}{\partial y^2 \partial x} f(x, y) \right) u_{1,2} + 3 \left( \frac{\partial^2}{\partial y \partial x} f(x, y) \right) u_{1,2,2} + \left( \frac{\partial^3}{\partial y^3} f(x, y) \right) u_{1,1} \\
 & + 3 \left( \frac{\partial^2}{\partial y^2} f(x, y) \right) u_{1,1,2} + 3 \left( \frac{\partial}{\partial y} f(x, y) \right) u_{1,1,2,2} + \left( \frac{\partial}{\partial x} f(x, y) \right) u_{1,2,2,2} \left. \right)
 \end{aligned} \tag{1}$$

$$D_{-}u_{1,2,2,2} - \left( \left( \frac{\partial^4}{\partial y^4} f(x,y) \right) u_1 + 4 \left( \frac{\partial^3}{\partial y^3} f(x,y) \right) u_{1,2} + 6 \left( \frac{\partial^2}{\partial y^2} f(x,y) \right) u_{1,2,2} + 4 \left( \frac{\partial}{\partial y} f(x,y) \right) u_{1,2,2,2} \right) D_{-}u_{2,2,2,2}$$

Here the action is transitive in the complement to  $\{u_1 = 0\}$ , so no differential invariants

>

1. Consider the singular statum  $S[1]=\{u_1 = 0\}$

>  $X4 := DGsimplify(subs(u_1=0, Prolong(evalDG(f(x,y) \cdot D_{-}x), 4)))$

$$\begin{aligned} X4 := & f(x,y) D_{-}x - 2 \left( \frac{\partial}{\partial x} f(x,y) \right) u_{1,1} D_{-}u_{1,1} - \left( \left( \frac{\partial}{\partial y} f(x,y) \right) u_{1,1} + \left( \frac{\partial}{\partial x} f(x,y) \right) u_{1,2} \right) D_{-}u_{1,2} - 2 \left( \frac{\partial}{\partial y} f(x,y) \right) u_{1,2} D_{-}u_{2,2} - \left( 3 \left( \frac{\partial^2}{\partial x^2} f(x,y) \right) u_{1,1} \right. \\ & + 3 \left( \frac{\partial}{\partial x} f(x,y) \right) u_{1,1,1} \left. \right) D_{-}u_{1,1,1} - \left( 2 \left( \frac{\partial^2}{\partial y \partial x} f(x,y) \right) u_{1,1} + \left( \frac{\partial^2}{\partial x^2} f(x,y) \right) u_{1,2} \right. \\ & + \left( \frac{\partial}{\partial y} f(x,y) \right) u_{1,1,1} + 2 \left( \frac{\partial}{\partial x} f(x,y) \right) u_{1,1,2} \left. \right) D_{-}u_{1,1,2} - \left( 2 \left( \frac{\partial^2}{\partial y \partial x} f(x,y) \right) u_{1,2} + \left( \frac{\partial^2}{\partial y^2} f(x,y) \right) u_{1,1} + 2 \left( \frac{\partial}{\partial y} f(x,y) \right) u_{1,1,2} + \left( \frac{\partial}{\partial x} f(x,y) \right) u_{1,2,2} \right) \\ & D_{-}u_{1,2,2} - \left( 3 \left( \frac{\partial^2}{\partial y^2} f(x,y) \right) u_{1,2} + 3 \left( \frac{\partial}{\partial y} f(x,y) \right) u_{1,2,2} \right) D_{-}u_{2,2,2} \\ & - \left( 4 \left( \frac{\partial^3}{\partial x^3} f(x,y) \right) u_{1,1} + 6 \left( \frac{\partial^2}{\partial x^2} f(x,y) \right) u_{1,1,1} + 4 \left( \frac{\partial}{\partial x} f(x,y) \right) u_{1,1,1,1} \right) D_{-}u_{1,1,1,1} - \left( 3 \left( \frac{\partial^3}{\partial y \partial x^2} f(x,y) \right) u_{1,1} + \left( \frac{\partial^3}{\partial x^3} f(x,y) \right) u_{1,2} \right. \\ & + 3 \left( \frac{\partial^2}{\partial y \partial x} f(x,y) \right) u_{1,1,1} + 3 \left( \frac{\partial^2}{\partial x^2} f(x,y) \right) u_{1,1,2} + \left( \frac{\partial}{\partial y} f(x,y) \right) u_{1,1,1,1} \\ & + 3 \left( \frac{\partial}{\partial x} f(x,y) \right) u_{1,1,1,2} \left. \right) D_{-}u_{1,1,1,2} - \left( 2 \left( \frac{\partial^3}{\partial y \partial x^2} f(x,y) \right) u_{1,2} \right. \\ & + 2 \left( \frac{\partial^3}{\partial y^2 \partial x} f(x,y) \right) u_{1,1} + 4 \left( \frac{\partial^2}{\partial y \partial x} f(x,y) \right) u_{1,1,2} + \left( \frac{\partial^2}{\partial x^2} f(x,y) \right) u_{1,2,2} \\ & + \left( \frac{\partial^2}{\partial y^2} f(x,y) \right) u_{1,1,1} + 2 \left( \frac{\partial}{\partial y} f(x,y) \right) u_{1,1,1,2} + 2 \left( \frac{\partial}{\partial x} f(x,y) \right) u_{1,1,2,2} \left. \right) \\ & D_{-}u_{1,1,2,2} - \left( 3 \left( \frac{\partial^3}{\partial y^2 \partial x} f(x,y) \right) u_{1,2} + 3 \left( \frac{\partial^2}{\partial y \partial x} f(x,y) \right) u_{1,2,2} + \left( \frac{\partial^3}{\partial y^3} f(x,y) \right) u_{1,1} + 3 \left( \frac{\partial^2}{\partial y^2} f(x,y) \right) u_{1,1,2} + 3 \left( \frac{\partial}{\partial y} f(x,y) \right) u_{1,1,2,2} + \left( \frac{\partial}{\partial x} f(x,y) \right) u_{1,2,2,2} \right) D_{-}u_{1,2,2,2} - \left( 4 \left( \frac{\partial^3}{\partial y^3} f(x,y) \right) u_{1,2} + 6 \left( \frac{\partial^2}{\partial y^2} f(x,y) \right) u_{1,2,2} + 4 \left( \frac{\partial}{\partial y} f(x,y) \right) u_{1,2,2,2} \right) D_{-}u_{2,2,2,2} \end{aligned} \quad (2)$$

>  $simplify(LieDerivative(X4, u_2));$

$$\begin{aligned}
& \text{simplify} \left( \text{LieDerivative} \left( X4, u_{2,2} - \frac{u_{1,2}^2}{u_{1,1}} \right) \right); \\
& \text{simplify} \left( \text{LieDerivative} \left( X4, u_{2,2,2} - \frac{u_{1,2}^3 u_{1,1,1}}{u_{1,1}^3} + \frac{3 u_{1,2}^2 u_{1,1,2}}{u_{1,1}^2} - \frac{3 u_{1,2} u_{1,2,2}}{u_{1,1}} \right) \right); \\
& \quad 0 \\
& \quad 0 \\
& \quad 0
\end{aligned} \tag{3}$$

Here everything is clear and the Poincare polynomial is  $P(z)=z+z^2+z^3+\dots=\frac{z}{1-z}$ .

>

2. Consider the singular statum  $S[2]=\{u_1=0, u_{1,1}=0\}$

$$\begin{aligned}
& > X4 := DG\text{simplify}(\text{subs}([u_1=0, u_{1,1}=0], \text{Prolong}(\text{evalDG}(f(x,y) \cdot D_x), 4))) \\
& X4 := f(x,y) D_x - \left( \frac{\partial}{\partial x} f(x,y) \right) u_{1,2} D_{u_{1,2}} - 2 \left( \frac{\partial}{\partial y} f(x,y) \right) u_{1,2} D_{u_{2,2}} \\
& \quad - 3 \left( \frac{\partial}{\partial x} f(x,y) \right) u_{1,1,1} D_{u_{1,1,1}} - \left( \left( \frac{\partial^2}{\partial x^2} f(x,y) \right) u_{1,2} + \left( \frac{\partial}{\partial y} f(x,y) \right) u_{1,1,1} \right. \\
& \quad \left. + 2 \left( \frac{\partial}{\partial x} f(x,y) \right) u_{1,1,2} \right) D_{u_{1,1,2}} - \left( 2 \left( \frac{\partial^2}{\partial y \partial x} f(x,y) \right) u_{1,2} + 2 \left( \frac{\partial}{\partial y} f(x,y) \right) u_{1,1,2} \right. \\
& \quad \left. + \left( \frac{\partial}{\partial x} f(x,y) \right) u_{1,2,2} \right) D_{u_{1,2,2}} - \left( 3 \left( \frac{\partial^2}{\partial y^2} f(x,y) \right) u_{1,2} + 3 \left( \frac{\partial}{\partial y} f(x,y) \right) u_{1,2,2} \right) D_{u_{2,2,2}} \\
& \quad - \left( 6 \left( \frac{\partial^2}{\partial x^2} f(x,y) \right) u_{1,1,1} + 4 \left( \frac{\partial}{\partial x} f(x,y) \right) u_{1,1,1,1} \right) D_{u_{1,1,1,1}} - \left( \left( \frac{\partial^3}{\partial x^3} f(x,y) \right) u_{1,2} + 3 \left( \frac{\partial^2}{\partial y \partial x} f(x,y) \right) u_{1,1,1} \right. \\
& \quad \left. + 3 \left( \frac{\partial^2}{\partial x^2} f(x,y) \right) u_{1,1,2} + \left( \frac{\partial}{\partial y} f(x,y) \right) u_{1,1,1,1} + 3 \left( \frac{\partial}{\partial x} f(x,y) \right) u_{1,1,1,2} \right) D_{u_{1,1,1,2}} \\
& \quad - \left( 2 \left( \frac{\partial^3}{\partial y \partial x^2} f(x,y) \right) u_{1,2} + 4 \left( \frac{\partial^2}{\partial y \partial x} f(x,y) \right) u_{1,1,2} + \left( \frac{\partial^2}{\partial x^2} f(x,y) \right) u_{1,2,2} \right. \\
& \quad \left. + \left( \frac{\partial^2}{\partial y^2} f(x,y) \right) u_{1,1,1} + 2 \left( \frac{\partial}{\partial y} f(x,y) \right) u_{1,1,1,2} + 2 \left( \frac{\partial}{\partial x} f(x,y) \right) u_{1,1,2,2} \right) D_{u_{1,1,2,2}} \\
& \quad - \left( 3 \left( \frac{\partial^3}{\partial y^2 \partial x} f(x,y) \right) u_{1,2} + 3 \left( \frac{\partial^2}{\partial y \partial x} f(x,y) \right) u_{1,2,2} + 3 \left( \frac{\partial^2}{\partial y^2} f(x,y) \right) u_{1,1,2} \right. \\
& \quad \left. + 3 \left( \frac{\partial}{\partial y} f(x,y) \right) u_{1,1,2,2} + \left( \frac{\partial}{\partial x} f(x,y) \right) u_{1,2,2,2} \right) D_{u_{1,2,2,2}} \\
& \quad - \left( 4 \left( \frac{\partial^3}{\partial y^3} f(x,y) \right) u_{1,2} + 6 \left( \frac{\partial^2}{\partial y^2} f(x,y) \right) u_{1,2,2} + 4 \left( \frac{\partial}{\partial y} f(x,y) \right) u_{1,2,2,2} \right) D_{u_{2,2,2,2}}
\end{aligned} \tag{4}$$

$$\begin{aligned}
& > \text{simplify}(\text{LieDerivative}(X4, u_2)); \\
& RES3 := \text{simplify}(\text{LieDerivative}(X4, u_{2,2,2} - F(u_{1,1,1}, u_{1,1,2}, u_{1,2,2}, u_{1,2}, u_{2,2}))); \\
& RES4 := \text{simplify}(\text{LieDerivative}(X4, u_{2,2,2,2} - F(u_{1,1,1}, u_{1,1,1,2}, u_{1,1,2,2}, u_{1,1,2}, u_{1,2,2,2}, u_{1,1,1}, u_{1,1,2}, u_{1,2,2}, u_{2,2}))) :
\end{aligned}$$

$$\begin{aligned}
RES3 := & \left( \frac{\partial}{\partial x} f(x, y) \right) u_{1,2} \left( \frac{\partial}{\partial u_{1,2}} F(u_{1,1,1}, u_{1,1,2}, u_{1,2,2}, u_{1,2}, u_{2,2}) \right) + 2 \left( \frac{\partial}{\partial y} f(x, \right. \\
& y) \left. \right) u_{1,2} \left( \frac{\partial}{\partial u_{2,2}} F(u_{1,1,1}, u_{1,1,2}, u_{1,2,2}, u_{1,2}, u_{2,2}) \right) + 3 \left( \frac{\partial}{\partial x} f(x, \right. \\
& y) \left. \right) u_{1,1,1} \left( \frac{\partial}{\partial u_{1,1,1}} F(u_{1,1,1}, u_{1,1,2}, u_{1,2,2}, u_{1,2}, u_{2,2}) \right) + \left( \frac{\partial}{\partial u_{1,1,2}} F(u_{1,1,1}, \right. \\
& u_{1,1,2}, u_{1,2,2}, u_{1,2}, u_{2,2}) \left. \right) \left( \frac{\partial^2}{\partial x^2} f(x, y) \right) u_{1,2} + \left( \frac{\partial}{\partial u_{1,1,2}} F(u_{1,1,1}, u_{1,1,2}, u_{1,2,2}, \right. \\
& u_{1,2}, u_{2,2}) \left. \right) \left( \frac{\partial}{\partial y} f(x, y) \right) u_{1,1,1} + 2 \left( \frac{\partial}{\partial u_{1,1,2}} F(u_{1,1,1}, u_{1,1,2}, u_{1,2,2}, u_{1,2}, \right. \\
& u_{2,2}) \left. \right) \left( \frac{\partial}{\partial x} f(x, y) \right) u_{1,1,2} + 2 \left( \frac{\partial}{\partial u_{1,2,2}} F(u_{1,1,1}, u_{1,1,2}, u_{1,2,2}, u_{1,2}, \right. \\
& u_{2,2}) \left. \right) \left( \frac{\partial^2}{\partial y \partial x} f(x, y) \right) u_{1,2} + 2 \left( \frac{\partial}{\partial u_{1,2,2}} F(u_{1,1,1}, u_{1,1,2}, u_{1,2,2}, u_{1,2}, \right. \\
& u_{2,2}) \left. \right) \left( \frac{\partial}{\partial y} f(x, y) \right) u_{1,1,2} + \left( \frac{\partial}{\partial u_{1,2,2}} F(u_{1,1,1}, u_{1,1,2}, u_{1,2,2}, u_{1,2}, \right. \\
& u_{2,2}) \left. \right) \left( \frac{\partial}{\partial x} f(x, y) \right) u_{1,2,2} - 3 \left( \frac{\partial^2}{\partial y^2} f(x, y) \right) u_{1,2} - 3 \left( \frac{\partial}{\partial y} f(x, y) \right) u_{1,2,2}
\end{aligned} \tag{5}$$

$$\begin{aligned}
> \text{coeff} \left( RES3, \frac{\partial^2}{\partial y^2} f(x, y) \right) \\
& -3 u_{1,2}
\end{aligned} \tag{6}$$

$$\begin{aligned}
> \text{coeff} \left( RES4, \frac{\partial^3}{\partial y^3} f(x, y) \right) \\
& -4 u_{1,2}
\end{aligned} \tag{7}$$

$$\begin{aligned}
> RES3 := \text{simplify}(\text{LieDerivative}(X4, F(u_{1,1,1}, u_{1,2}))); \\
RES4 := \text{simplify}(\text{LieDerivative}(X4, F(u_{1,1,1,1}, u_{1,1,1}, u_{1,1,2}, u_{1,2}, u_{2,2}))); \\
RES3 := - \left( \frac{\partial}{\partial x} f(x, y) \right) \left( u_{1,2} \left( \frac{\partial}{\partial u_{1,2}} F(u_{1,1,1}, u_{1,2}) \right) + 3 u_{1,1,1} \left( \frac{\partial}{\partial u_{1,1,1}} F(u_{1,1,1}, \right. \right. \\
& u_{1,2}) \left. \right) \left. \right) \\
RES4 := - \left( \frac{\partial}{\partial x} f(x, y) \right) u_{1,2} \left( \frac{\partial}{\partial u_{1,2}} F(u_{1,1,1,1}, u_{1,1,1}, u_{1,1,2}, u_{1,2}, u_{2,2}) \right) - 2 \left( \frac{\partial}{\partial y} f(x, \right. \\
& y) \left. \right) u_{1,2} \left( \frac{\partial}{\partial u_{2,2}} F(u_{1,1,1,1}, u_{1,1,1}, u_{1,1,2}, u_{1,2}, u_{2,2}) \right) - 3 \left( \frac{\partial}{\partial x} f(x, \right. \\
& y) \left. \right) u_{1,1,1} \left( \frac{\partial}{\partial u_{1,1,1}} F(u_{1,1,1,1}, u_{1,1,1}, u_{1,1,2}, u_{1,2}, u_{2,2}) \right) - \left( \frac{\partial}{\partial u_{1,1,2}} F(u_{1,1,1,1}, \right. \\
& u_{1,1,1}, u_{1,1,2}, u_{1,2}, u_{2,2}) \left. \right) \left( \frac{\partial^2}{\partial x^2} f(x, y) \right) u_{1,2} - \left( \frac{\partial}{\partial u_{1,1,2}} F(u_{1,1,1,1}, u_{1,1,1}, u_{1,1,2}, \right. \\
& u_{1,2}, u_{2,2}) \left. \right) \left( \frac{\partial}{\partial y} f(x, y) \right) u_{1,1,1} - 2 \left( \frac{\partial}{\partial u_{1,1,2}} F(u_{1,1,1,1}, u_{1,1,1}, u_{1,1,2}, u_{1,2}, \right.
\end{aligned} \tag{8}$$

$$u_{2,2}) \left( \frac{\partial}{\partial x} f(x,y) \right) u_{1,1,2} - 6 \left( \frac{\partial}{\partial u_{1,1,1}} F(u_{1,1,1}, u_{1,1}, u_{1,1,2}, u_{1,2}, u_{2,2}) \right) \left( \frac{\partial^2}{\partial x^2} f(x,y) \right) u_{1,1,1} - 4 \left( \frac{\partial}{\partial u_{1,1,1}} F(u_{1,1,1}, u_{1,1}, u_{1,1,2}, u_{1,2}, u_{2,2}) \right) \left( \frac{\partial}{\partial x} f(x,y) \right) u_{1,1,1,1}$$

$$\begin{aligned} &> \text{pdsolve} \left( u_{1,2} \left( \frac{\partial}{\partial u_{1,2}} F(u_{1,1,1}, u_{1,2}) \right) + 3 u_{1,1,1} \left( \frac{\partial}{\partial u_{1,1,1}} F(u_{1,1,1}, u_{1,2}) \right) \right) \\ &F(u_{1,1,1}, u_{1,2}) = -FI \left( \frac{u_{1,2}}{u_{1,1,1}^{(1/3)}} \right) \end{aligned} \quad (9)$$

$$\begin{aligned} &> \text{coeff} \left( RES4, \frac{\partial^2}{\partial x^2} f(x,y) \right) \\ &- \left( \frac{\partial}{\partial u_{1,1,2}} F(u_{1,1,1}, u_{1,1}, u_{1,1,2}, u_{1,2}, u_{2,2}) \right) u_{1,2} - 6 \left( \frac{\partial}{\partial u_{1,1,1}} F(u_{1,1,1}, u_{1,1}, u_{1,1,2}, u_{1,2}, u_{2,2}) \right) u_{1,1,1} \end{aligned} \quad (10)$$

$$\begin{aligned} &> \text{pdsolve}(\%) \\ &F(u_{1,1,1}, u_{1,1}, u_{1,1,2}, u_{1,2}, u_{2,2}) = -FI \left( u_{1,1,1}, u_{1,2}, \right. \\ &\quad \left. \frac{1}{6} \frac{-u_{1,2} u_{1,1,1,1} + 6 u_{1,1,2} u_{1,1,1}}{u_{1,1,1}}, u_{2,2} \right) \end{aligned} \quad (11)$$

$$\begin{aligned} &> RES4 := \text{simplify} \left( \text{LieDerivative} \left( X4, F \left( u_{1,1,1}, u_{1,2}, \frac{1}{6} \frac{-u_{1,2} u_{1,1,1,1} + 6 u_{1,1,2} u_{1,1,1}}{u_{1,1,1}}, u_{2,2} \right) \right) \right); \\ &RES4 := -\frac{1}{3} \frac{1}{u_{1,1,1}} \left( 3 D_1(f)(x,y) u_{1,2} D_2(F) \left( u_{1,1,1}, u_{1,2}, \right. \right. \\ &\quad \left. \left. - \frac{1}{6} \frac{u_{1,2} u_{1,1,1,1} - 6 u_{1,1,2} u_{1,1,1}}{u_{1,1,1}}, u_{2,2} \right) u_{1,1,1} - D_1(f)(x,y) u_{1,2} D_3(F) \left( u_{1,1,1}, \right. \right. \\ &\quad \left. \left. u_{1,2}, - \frac{1}{6} \frac{u_{1,2} u_{1,1,1,1} - 6 u_{1,1,2} u_{1,1,1}}{u_{1,1,1}}, u_{2,2} \right) u_{1,1,1,1} + 6 D_2(f)(x, \right. \\ &\quad \left. y) u_{1,2} D_4(F) \left( u_{1,1,1}, u_{1,2}, - \frac{1}{6} \frac{u_{1,2} u_{1,1,1,1} - 6 u_{1,1,2} u_{1,1,1}}{u_{1,1,1}}, u_{2,2} \right) u_{1,1,1} \right. \\ &\quad \left. + 9 D_1(f)(x,y) D_1(F) \left( u_{1,1,1}, u_{1,2}, - \frac{1}{6} \frac{u_{1,2} u_{1,1,1,1} - 6 u_{1,1,2} u_{1,1,1}}{u_{1,1,1}}, u_{2,2} \right) u_{1,1,1}^2 \right. \\ &\quad \left. + 3 D_3(F) \left( u_{1,1,1}, u_{1,2}, - \frac{1}{6} \frac{u_{1,2} u_{1,1,1,1} - 6 u_{1,1,2} u_{1,1,1}}{u_{1,1,1}}, u_{2,2} \right) u_{1,1,1}^2 D_2(f)(x,y) \right. \\ &\quad \left. + 6 D_3(F) \left( u_{1,1,1}, u_{1,2}, - \frac{1}{6} \frac{u_{1,2} u_{1,1,1,1} - 6 u_{1,1,2} u_{1,1,1}}{u_{1,1,1}}, u_{2,2} \right) u_{1,1,1} D_1(f)(x, \right. \end{aligned} \quad (12)$$

$$y) u_{1,1,2} \Big)$$

$$\begin{aligned} &> \text{solve} \left( -\frac{1}{6} \frac{u_{1,2} u_{1,1,1,1} - 6 u_{1,1,2} u_{1,1,1}}{u_{1,1,1}} = q, u_{1,1,1,1} \right) \\ &\quad - \frac{6 (q - u_{1,1,2}) u_{1,1,1}}{u_{1,2}} \end{aligned} \quad (13)$$

$$\begin{aligned} &> \text{simplify} \left( -\text{subs} \left( u_{1,1,1,1} = -\frac{6 (q - u_{1,1,2}) u_{1,1,1}}{u_{1,2}}, [\text{coeff}(\text{RES4}, D_1(f)(x, y)), \right. \right. \\ &\quad \left. \left. \text{coeff}(\text{RES4}, D_2(f)(x, y)) \right] \right) \\ &[u_{1,2} D_2(F)(u_{1,1,1}, u_{1,2}, q, u_{2,2}) + 2 D_3(F)(u_{1,1,1}, u_{1,2}, q, u_{2,2}) q + 3 D_1(F)(u_{1,1,1}, \\ &\quad u_{1,2}, q, u_{2,2}) u_{1,1,1}, 2 u_{1,2} D_4(F)(u_{1,1,1}, u_{1,2}, q, u_{2,2}) + D_3(F)(u_{1,1,1}, u_{1,2}, q, \\ &\quad u_{2,2}) u_{1,1,1}] \end{aligned} \quad (14)$$

$$\begin{aligned} &> \text{pdsolve}(\%) \\ &\quad \left\{ F(u_{1,1,1}, u_{1,2}, q, u_{2,2}) = -FI \left( \frac{u_{1,2}}{u_{1,1,1}^{(1/3)}}, \frac{-2 u_{1,2} q + u_{2,2} u_{1,1,1}}{u_{1,1,1}} \right) \right\} \end{aligned} \quad (15)$$

$$\begin{aligned} &> \text{simplify} \left( \text{subs} \left( q = -\frac{1}{6} \frac{u_{1,2} u_{1,1,1,1} - 6 u_{1,1,2} u_{1,1,1}}{u_{1,1,1}}, \frac{-2 u_{1,2} q + u_{2,2} u_{1,1,1}}{u_{1,1,1}} \right) \right. \\ &\quad \left. \cdot \frac{3 u_{1,1,1}^2}{u_{1,2}^6} \right) \\ &\quad \frac{u_{1,2}^2 u_{1,1,1,1} - 6 u_{1,2} u_{1,1,2} u_{1,1,1} + 3 u_{2,2} u_{1,1,1}^2}{u_{1,2}^6} \end{aligned} \quad (16)$$

$$\begin{aligned} &> \text{simplify} \left( \text{LieDerivative} \left( X4, \frac{u_{1,1,1}}{u_{1,2}^3} \right) \right) \\ &\quad 0 \end{aligned} \quad (17)$$

$$\begin{aligned} &> \text{simplify} \left( \text{LieDerivative} \left( X4, \frac{u_{1,2}^2 u_{1,1,1,1} - 6 u_{1,2} u_{1,1,2} u_{1,1,1} + 3 u_{2,2} u_{1,1,1}^2}{u_{1,2}^6} \right) \right) \\ &\quad 0 \end{aligned} \quad (18)$$

Thus we see one new differential invariant in every order except for order 2. So  $P(z) = z + z^3 + z^4 + \dots = \frac{z - z^2 + z^3}{1 - z}$ .

>

3. Consider the singular statum  $S[3] = \{u_1 = 0, u_{1,1} = 0, u_{1,2} = 0\}$

$$\begin{aligned} &> X4 := \text{DGsimplify}(\text{subs}([u_1 = 0, u_{1,1} = 0, u_{1,2} = 0], \text{Prolong}(\text{evalDG}(f(x, y) \cdot D_x), 4))) \\ X4 &:= f(x, y) D_x - 3 \left( \frac{\partial}{\partial x} f(x, y) \right) u_{1,1,1} D_{u_{1,1,1}} - \left( \left( \frac{\partial}{\partial y} f(x, y) \right) u_{1,1,1} \right. \\ &\quad \left. + 2 \left( \frac{\partial}{\partial x} f(x, y) \right) u_{1,1,2} \right) D_{u_{1,1,2}} - \left( 2 \left( \frac{\partial}{\partial y} f(x, y) \right) u_{1,1,2} + \left( \frac{\partial}{\partial x} f(x, \right. \right. \end{aligned} \quad (19)$$

$$\begin{aligned}
& y) \Big) u_{1,2,2} \Big) D_{-} u_{1,2,2} - 3 \left( \frac{\partial}{\partial y} f(x,y) \right) u_{1,2,2} D_{-} u_{2,2,2} - \left( 6 \left( \frac{\partial^2}{\partial x^2} f(x,y) \right) u_{1,1,1} \right. \\
& + 4 \left( \frac{\partial}{\partial x} f(x,y) \right) u_{1,1,1,1} \Big) D_{-} u_{1,1,1,1} - \left( 3 \left( \frac{\partial^2}{\partial y \partial x} f(x,y) \right) u_{1,1,1} + 3 \left( \frac{\partial^2}{\partial x^2} f(x, \right. \right. \\
& y) \Big) u_{1,1,2} + \left( \frac{\partial}{\partial y} f(x,y) \right) u_{1,1,1,1} + 3 \left( \frac{\partial}{\partial x} f(x,y) \right) u_{1,1,1,2} \Big) D_{-} u_{1,1,1,2} \\
& - \left( 4 \left( \frac{\partial^2}{\partial y \partial x} f(x,y) \right) u_{1,1,2} + \left( \frac{\partial^2}{\partial x^2} f(x,y) \right) u_{1,2,2} + \left( \frac{\partial^2}{\partial y^2} f(x,y) \right) u_{1,1,1} \right. \\
& + 2 \left( \frac{\partial}{\partial y} f(x,y) \right) u_{1,1,1,2} + 2 \left( \frac{\partial}{\partial x} f(x,y) \right) u_{1,1,2,2} \Big) D_{-} u_{1,1,2,2} - \left( 3 \left( \frac{\partial^2}{\partial y \partial x} f(x, \right. \right. \\
& y) \Big) u_{1,2,2} + 3 \left( \frac{\partial^2}{\partial y^2} f(x,y) \right) u_{1,1,2} + 3 \left( \frac{\partial}{\partial y} f(x,y) \right) u_{1,1,2,2} + \left( \frac{\partial}{\partial x} f(x, \right. \\
& y) \Big) u_{1,2,2,2} \Big) D_{-} u_{1,2,2,2} - \left( 6 \left( \frac{\partial^2}{\partial y^2} f(x,y) \right) u_{1,2,2} + 4 \left( \frac{\partial}{\partial y} f(x, \right. \right. \\
& y) \Big) u_{1,2,2,2} \Big) D_{-} u_{2,2,2,2}
\end{aligned}$$

> simplify(LieDerivative(X4,  $\mathbf{u_2}$ ));

simplify(LieDerivative(X4,  $\mathbf{u_{2,2}}$ ));

RES := simplify(LieDerivative(X4,  $u_{2,2,2} - F(u_{1,1,1}, u_{1,1,2}, u_{1,2,2})$ ));

0  
0

$$\begin{aligned}
RES := & 3 \left( \frac{\partial}{\partial x} f(x,y) \right) u_{1,1,1} \left( \frac{\partial}{\partial u_{1,1,1}} F(u_{1,1,1}, u_{1,1,2}, u_{1,2,2}) \right) + \left( \frac{\partial}{\partial u_{1,1,2}} F(u_{1,1,1}, \right. \\
& u_{1,1,2}, u_{1,2,2}) \Big) \left( \frac{\partial}{\partial y} f(x,y) \right) u_{1,1,1} + 2 \left( \frac{\partial}{\partial u_{1,1,2}} F(u_{1,1,1}, u_{1,1,2}, \right. \\
& u_{1,2,2}) \Big) \left( \frac{\partial}{\partial x} f(x,y) \right) u_{1,1,2} + 2 \left( \frac{\partial}{\partial u_{1,2,2}} F(u_{1,1,1}, u_{1,1,2}, u_{1,2,2}) \right) \left( \frac{\partial}{\partial y} f(x, \right. \\
& y) \Big) u_{1,1,2} + \left( \frac{\partial}{\partial u_{1,2,2}} F(u_{1,1,1}, u_{1,1,2}, u_{1,2,2}) \right) \left( \frac{\partial}{\partial x} f(x,y) \right) u_{1,2,2} - 3 \left( \frac{\partial}{\partial y} f(x, \right. \\
& y) \Big) u_{1,2,2}
\end{aligned} \tag{20}$$

> coeff(RES,  $\frac{\partial}{\partial x} f(x,y)$ ); coeff(RES,  $\frac{\partial}{\partial y} f(x,y)$ )

$$\begin{aligned}
& 3 u_{1,1,1} \left( \frac{\partial}{\partial u_{1,1,1}} F(u_{1,1,1}, u_{1,1,2}, u_{1,2,2}) \right) + 2 \left( \frac{\partial}{\partial u_{1,1,2}} F(u_{1,1,1}, u_{1,1,2}, u_{1,2,2}) \right) u_{1,1,2} \\
& + \left( \frac{\partial}{\partial u_{1,2,2}} F(u_{1,1,1}, u_{1,1,2}, u_{1,2,2}) \right) u_{1,2,2} \\
& \left( \frac{\partial}{\partial u_{1,1,2}} F(u_{1,1,1}, u_{1,1,2}, u_{1,2,2}) \right) u_{1,1,1} + 2 \left( \frac{\partial}{\partial u_{1,2,2}} F(u_{1,1,1}, u_{1,1,2}, u_{1,2,2}) \right) u_{1,1,2} \\
& - 3 u_{1,2,2}
\end{aligned} \tag{21}$$

> pdsolve( [ 3 u\_{1,1,1} \left( \frac{\partial}{\partial u\_{1,1,1}} F(u\_{1,1,1}, u\_{1,1,2}, u\_{1,2,2}) \right) + 2 \left( \frac{\partial}{\partial u\_{1,1,2}} F(u\_{1,1,1}, u\_{1,1,2}, u\_{1,2,2}) \right) u\_{1,1,2} + \left( \frac{\partial}{\partial u\_{1,2,2}} F(u\_{1,1,1}, u\_{1,1,2}, u\_{1,2,2}) \right) u\_{1,2,2} - 3 u\_{1,2,2} ] )

$$\begin{aligned}
& \left. \begin{aligned} & u_{1,2,2}) \right) u_{1,1,2} + \left( \frac{\partial}{\partial u_{1,2,2}} F(u_{1,1,1}, u_{1,1,2}, u_{1,2,2}) \right) u_{1,2,2} = 0, \left( \frac{\partial}{\partial u_{1,1,2}} F(u_{1,1,1}, \right. \\ & \left. u_{1,1,2}, u_{1,2,2}) \right) u_{1,1,1} + 2 \left( \frac{\partial}{\partial u_{1,2,2}} F(u_{1,1,1}, u_{1,1,2}, u_{1,2,2}) \right) u_{1,1,2} - 3 u_{1,2,2} = 0 \left. \vphantom{\frac{\partial}{\partial u_{1,2,2}}} \right) \Bigg] \\ & \left\{ F(u_{1,1,1}, u_{1,1,2}, u_{1,2,2}) \right. \\ & \left. = \frac{-F1 \left( \frac{-u_{1,1,2}^2 + u_{1,1,1} u_{1,2,2}}{u_{1,1,1}^{(4/3)}} \right) u_{1,1,1}^2 - 2 u_{1,1,2}^3 + 3 u_{1,1,2} u_{1,1,1} u_{1,2,2}}{u_{1,1,1}^2} \right\} \end{aligned} \quad (22)
\end{aligned}$$

$$\begin{aligned}
& \text{> simplify} \left( \text{LieDerivative} \left( X4, u_{2,2,2} - \frac{-2 u_{1,1,2}^3 + 3 u_{1,1,2} u_{1,1,1} u_{1,2,2}}{u_{1,1,1}^2} \right) \right) \\ & \quad \quad \quad 0 \quad \quad \quad (23)
\end{aligned}$$

$$\begin{aligned}
& \text{> simplify} \left( \text{LieDerivative} \left( X4, \frac{-u_{1,1,2}^2 + u_{1,1,1} u_{1,2,2}}{u_{1,1,1}^{(4/3)}} \right) \right) \\ & \quad \quad \quad 0 \quad \quad \quad (24)
\end{aligned}$$

It is clear (from the expansion of the Lie Algebra Sheaf) that we get 2 new differential invariants every order >2. So  $P(z)=z+z^2+2z^3+2z^4+\dots=\frac{z+z^3}{1-z}$ .

>

4. Consider the singular statum  $S[4]=\{u_1=0, u_{1,1}=0, u_{1,2}=0, u_{1,1,1}=0\}$

>  $X4 := \text{DGsimplify}(\text{subs}([u_1=0, u_{1,1}=0, u_{1,2}=0, u_{1,1,1}=0], \text{Prolong}(\text{evalDG}(f(x, y) \cdot D_x), 4)))$

$$\begin{aligned}
X4 := & f(x, y) D_x - 2 \left( \frac{\partial}{\partial x} f(x, y) \right) u_{1,1,2} D_{u_{1,1,2}} - \left( 2 \left( \frac{\partial}{\partial y} f(x, y) \right) u_{1,1,2} \right. \\ & + \left( \frac{\partial}{\partial x} f(x, y) \right) u_{1,2,2} \Big) D_{u_{1,2,2}} - 3 \left( \frac{\partial}{\partial y} f(x, y) \right) u_{1,2,2} D_{u_{2,2,2}} - 4 \left( \frac{\partial}{\partial x} f(x, \right. \\ & \left. y) \right) u_{1,1,1,1} D_{u_{1,1,1,1}} - \left( 3 \left( \frac{\partial^2}{\partial x^2} f(x, y) \right) u_{1,1,2} + \left( \frac{\partial}{\partial y} f(x, y) \right) u_{1,1,1,1} \right. \\ & + 3 \left( \frac{\partial}{\partial x} f(x, y) \right) u_{1,1,1,2} \Big) D_{u_{1,1,1,2}} - \left( 4 \left( \frac{\partial^2}{\partial y \partial x} f(x, y) \right) u_{1,1,2} + \left( \frac{\partial^2}{\partial x^2} f(x, \right. \right. \\ & \left. y) \right) u_{1,2,2} + 2 \left( \frac{\partial}{\partial y} f(x, y) \right) u_{1,1,1,2} + 2 \left( \frac{\partial}{\partial x} f(x, y) \right) u_{1,1,2,2} \Big) D_{u_{1,1,2,2}} \\ & - \left( 3 \left( \frac{\partial^2}{\partial y \partial x} f(x, y) \right) u_{1,2,2} + 3 \left( \frac{\partial^2}{\partial y^2} f(x, y) \right) u_{1,1,2} + 3 \left( \frac{\partial}{\partial y} f(x, y) \right) u_{1,1,2,2} \right. \\ & + \left( \frac{\partial}{\partial x} f(x, y) \right) u_{1,2,2,2} \Big) D_{u_{1,2,2,2}} - \left( 6 \left( \frac{\partial^2}{\partial y^2} f(x, y) \right) u_{1,2,2} + 4 \left( \frac{\partial}{\partial y} f(x, \right. \right. \\ & \left. y) \right) u_{1,2,2,2} \Big) D_{u_{2,2,2,2}} \end{aligned} \quad (25)$$

>  $\text{simplify}(\text{LieDerivative}(X4, u_2));$



*simplify*(*LieDerivative*(*X4*,  $\mathbf{u_{2,2}}$ ));

*RES3* := *simplify*(*LieDerivative*(*X4*,  $u_{2,2,2} - F(u_{1,1,2}, u_{1,2,2})$ ));

*RES4* := *simplify*(*LieDerivative*(*X4*,  $u_{2,2,2,2} - F(u_{1,1,1,1}, u_{1,1,1,2}, u_{1,1,2,2}, u_{1,2,2,2}, u_{1,1,2,2}, u_{1,2,2,2})$ )) :

0  
0

$$\begin{aligned} RES3 := & 2 \left( \frac{\partial}{\partial x} f(x, y) \right) u_{1,1,2} \left( \frac{\partial}{\partial u_{1,1,2}} F(u_{1,1,2}, u_{1,2,2}) \right) + 2 \left( \frac{\partial}{\partial u_{1,2,2}} F(u_{1,1,2}, \right. \\ & \left. u_{1,2,2}) \right) \left( \frac{\partial}{\partial y} f(x, y) \right) u_{1,1,2} + \left( \frac{\partial}{\partial u_{1,2,2}} F(u_{1,1,2}, u_{1,2,2}) \right) \left( \frac{\partial}{\partial x} f(x, y) \right) u_{1,2,2} \\ & - 3 \left( \frac{\partial}{\partial y} f(x, y) \right) u_{1,2,2} \end{aligned} \quad (26)$$

$$\begin{aligned} > \text{coeff} \left( RES3, \frac{\partial}{\partial x} f(x, y) \right); \text{coeff} \left( RES3, \frac{\partial}{\partial y} f(x, y) \right); \\ & 2 u_{1,1,2} \left( \frac{\partial}{\partial u_{1,1,2}} F(u_{1,1,2}, u_{1,2,2}) \right) + \left( \frac{\partial}{\partial u_{1,2,2}} F(u_{1,1,2}, u_{1,2,2}) \right) u_{1,2,2} \\ & 2 \left( \frac{\partial}{\partial u_{1,2,2}} F(u_{1,1,2}, u_{1,2,2}) \right) u_{1,1,2} - 3 u_{1,2,2} \end{aligned} \quad (27)$$

$$\begin{aligned} > \text{pdsolve} \left( \left[ 2 u_{1,1,2} \left( \frac{\partial}{\partial u_{1,1,2}} F(u_{1,1,2}, u_{1,2,2}) \right) + \left( \frac{\partial}{\partial u_{1,2,2}} F(u_{1,1,2}, u_{1,2,2}) \right) u_{1,2,2} = 0, \right. \right. \\ & \left. \left. 2 \left( \frac{\partial}{\partial u_{1,2,2}} F(u_{1,1,2}, u_{1,2,2}) \right) u_{1,1,2} - 3 u_{1,2,2} = 0 \right] \right) \\ & \left\{ F(u_{1,1,2}, u_{1,2,2}) = \frac{3}{4} \frac{u_{1,2,2}^2}{u_{1,1,2}} + \_CI \right\} \end{aligned} \quad (28)$$

$$\begin{aligned} > \text{simplify} \left( \text{LieDerivative} \left( X4, \mathbf{u_{2,2,2}} - \frac{3}{4} \frac{u_{1,2,2}^2}{u_{1,1,2}} \right) \right) \\ & 0 \end{aligned} \quad (29)$$

$$\begin{aligned} > \left[ \text{coeff} \left( RES4, \frac{\partial^2}{\partial x^2} f(x, y) \right), \text{coeff} \left( RES4, \frac{\partial^2}{\partial y \partial x} f(x, y) \right), \text{coeff} \left( RES4, \frac{\partial^2}{\partial y^2} f(x, y) \right) \right] \\ & \left[ 3 \left( \frac{\partial}{\partial u_{1,1,1,2}} F(u_{1,1,1,1}, u_{1,1,1,2}, u_{1,1,2,2}, u_{1,2,2,2}, u_{1,1,2,2}, u_{1,2,2,2}) \right) u_{1,1,2} \right. \\ & + \left( \frac{\partial}{\partial u_{1,1,2,2}} F(u_{1,1,1,1}, u_{1,1,1,2}, u_{1,1,2,2}, u_{1,2,2,2}, u_{1,1,2,2}, u_{1,2,2,2}) \right) u_{1,2,2}, \\ & 4 \left( \frac{\partial}{\partial u_{1,1,2,2}} F(u_{1,1,1,1}, u_{1,1,1,2}, u_{1,1,2,2}, u_{1,2,2,2}, u_{1,1,2,2}, u_{1,2,2,2}) \right) u_{1,1,2} \\ & + 3 \left( \frac{\partial}{\partial u_{1,2,2,2}} F(u_{1,1,1,1}, u_{1,1,1,2}, u_{1,1,2,2}, u_{1,2,2,2}, u_{1,1,2,2}, u_{1,2,2,2}) \right) u_{1,2,2}, \\ & \left. 3 \left( \frac{\partial}{\partial u_{1,2,2,2}} F(u_{1,1,1,1}, u_{1,1,1,2}, u_{1,1,2,2}, u_{1,2,2,2}, u_{1,1,2,2}, u_{1,2,2,2}) \right) u_{1,1,2} - 6 u_{1,2,2} \right] \end{aligned} \quad (30)$$

$$\begin{aligned} > \text{pdsolve}(\%) \\ & \left\{ F(u_{1,1,1,1}, u_{1,1,1,2}, u_{1,1,2,2}, u_{1,2,2,2}, u_{1,1,2,2}, u_{1,2,2,2}) = \frac{2 u_{1,2,2} u_{1,2,2,2}}{u_{1,1,2}} \right\} \end{aligned} \quad (31)$$

$$\left. + \frac{1}{2} \frac{u_{1,2,2}^3 u_{1,1,1,2}}{u_{1,1,2}^3} - \frac{3}{2} \frac{u_{1,2,2}^2 u_{1,1,2,2}}{u_{1,1,2}^2} + \text{FI}(u_{1,1,1,1}, u_{1,1,2}, u_{1,2,2}) \right\}$$

$$\begin{aligned} &> \text{RES4} := \text{simplify} \left( \text{LieDerivative} \left( X4, u_{2,2,2,2} - \frac{2 u_{1,2,2} u_{1,2,2,2}}{u_{1,1,2}} - \frac{1}{2} \frac{u_{1,2,2}^3 u_{1,1,1,2}}{u_{1,1,2}^3} \right. \right. \\ &\quad \left. \left. + \frac{3}{2} \frac{u_{1,2,2}^2 u_{1,1,2,2}}{u_{1,1,2}^2} + \text{FI}(u_{1,1,1,1}, u_{1,1,2}, u_{1,2,2}) \right) \right) \end{aligned} \quad (32)$$

$$\begin{aligned} \text{RES4} := & -\frac{1}{2} \frac{1}{u_{1,1,2}^3} \left( 4 \left( \frac{\partial}{\partial x} f(x, y) \right) \left( \frac{\partial}{\partial u_{1,1,2}} \text{FI}(u_{1,1,1,1}, u_{1,1,2}, u_{1,2,2}) \right) u_{1,1,2}^4 \right. \\ & + 4 \left( \frac{\partial}{\partial y} f(x, y) \right) u_{1,1,2}^4 \left( \frac{\partial}{\partial u_{1,2,2}} \text{FI}(u_{1,1,1,1}, u_{1,1,2}, u_{1,2,2}) \right) - u_{1,2,2}^3 \left( \frac{\partial}{\partial y} f(x, \right. \\ & y) \left. \right) u_{1,1,1,1} + 8 \left( \frac{\partial}{\partial x} f(x, y) \right) u_{1,1,1,1} \left( \frac{\partial}{\partial u_{1,1,1,1}} \text{FI}(u_{1,1,1,1}, u_{1,1,2}, u_{1,2,2}) \right) u_{1,1,2}^3 \\ & \left. + 2 \left( \frac{\partial}{\partial x} f(x, y) \right) u_{1,2,2} \left( \frac{\partial}{\partial u_{1,2,2}} \text{FI}(u_{1,1,1,1}, u_{1,1,2}, u_{1,2,2}) \right) u_{1,1,2}^3 \right) \end{aligned}$$

$$\begin{aligned} &> \left[ \text{coeff} \left( \text{RES4}, \frac{\partial}{\partial x} f(x, y) \right), \text{coeff} \left( \text{RES4}, \frac{\partial}{\partial y} f(x, y) \right) \right] \\ &\left[ -\frac{1}{2} \frac{1}{u_{1,1,2}^3} \left( 4 \left( \frac{\partial}{\partial u_{1,1,2}} \text{FI}(u_{1,1,1,1}, u_{1,1,2}, u_{1,2,2}) \right) u_{1,1,2}^4 \right. \right. \end{aligned} \quad (33)$$

$$\left. + 8 u_{1,1,1,1} \left( \frac{\partial}{\partial u_{1,1,1,1}} \text{FI}(u_{1,1,1,1}, u_{1,1,2}, u_{1,2,2}) \right) u_{1,1,2}^3 \right.$$

$$\left. + 2 u_{1,2,2} \left( \frac{\partial}{\partial u_{1,2,2}} \text{FI}(u_{1,1,1,1}, u_{1,1,2}, u_{1,2,2}) \right) u_{1,1,2}^3 \right),$$

$$\left. - \frac{1}{2} \frac{4 u_{1,1,2}^4 \left( \frac{\partial}{\partial u_{1,2,2}} \text{FI}(u_{1,1,1,1}, u_{1,1,2}, u_{1,2,2}) \right) - u_{1,2,2}^3 u_{1,1,1,1}}{u_{1,1,2}^3} \right]$$

$$\begin{aligned} &> \text{pdsolve}(\%) \\ &\left\{ \text{FI}(u_{1,1,1,1}, u_{1,1,2}, u_{1,2,2}) = \frac{1}{16} \frac{u_{1,2,2}^4 u_{1,1,1,1}}{u_{1,1,2}^4} + \text{FI} \left( \frac{u_{1,1,2}}{\sqrt{u_{1,1,1,1}}} \right) \right\} \end{aligned} \quad (34)$$

$$\begin{aligned} &> \text{simplify} \left( \text{LieDerivative} \left( X4, u_{2,2,2,2} - \frac{2 u_{1,2,2} u_{1,2,2,2}}{u_{1,1,2}} - \frac{1}{2} \frac{u_{1,2,2}^3 u_{1,1,1,2}}{u_{1,1,2}^3} \right. \right. \\ &\quad \left. \left. + \frac{3}{2} \frac{u_{1,2,2}^2 u_{1,1,2,2}}{u_{1,1,2}^2} + \frac{1}{16} \frac{u_{1,2,2}^4 u_{1,1,1,1}}{u_{1,1,2}^4} \right) \right) \end{aligned} \quad (35)$$

$$\begin{aligned} & \text{> simplify}\left(\text{LieDerivative}\left(X4, \frac{u_{1,1,1,1}}{u_{1,1,2}^2}\right)\right) \\ & \quad \quad \quad 0 \end{aligned} \tag{36}$$

$$\text{> } X5 := \text{DGsimplify}\left(\text{subs}\left([u_1=0, u_{1,1}=0, u_{1,2}=0, u_{1,1,1}=0], \text{Prolong}(\text{evalDG}(f(x, y) \cdot D_x), 5)\right)\right)$$

$$\begin{aligned} X5 := & f(x, y) D_x - 2 \left( \frac{\partial}{\partial x} f(x, y) \right) u_{1,1,2} D_{u_{1,1,2}} - \left( 2 \left( \frac{\partial}{\partial y} f(x, y) \right) u_{1,1,2} \right. \\ & + \left( \frac{\partial}{\partial x} f(x, y) \right) u_{1,2,2} \left. \right) D_{u_{1,2,2}} - 3 \left( \frac{\partial}{\partial y} f(x, y) \right) u_{1,2,2} D_{u_{2,2,2}} - 4 \left( \frac{\partial}{\partial x} f(x, y) \right) u_{1,1,1,1} D_{u_{1,1,1,1}} \\ & - \left( 3 \left( \frac{\partial^2}{\partial x^2} f(x, y) \right) u_{1,1,2} + \left( \frac{\partial}{\partial y} f(x, y) \right) u_{1,1,1,1} \right. \\ & + 3 \left( \frac{\partial}{\partial x} f(x, y) \right) u_{1,1,1,2} \left. \right) D_{u_{1,1,1,2}} - \left( 4 \left( \frac{\partial^2}{\partial y \partial x} f(x, y) \right) u_{1,1,2} + \left( \frac{\partial^2}{\partial x^2} f(x, y) \right) u_{1,2,2} \right. \\ & + 2 \left( \frac{\partial}{\partial y} f(x, y) \right) u_{1,1,1,2} + 2 \left( \frac{\partial}{\partial x} f(x, y) \right) u_{1,1,2,2} \left. \right) D_{u_{1,1,2,2}} \\ & - \left( 3 \left( \frac{\partial^2}{\partial y \partial x} f(x, y) \right) u_{1,2,2} + 3 \left( \frac{\partial^2}{\partial y^2} f(x, y) \right) u_{1,1,2} + 3 \left( \frac{\partial}{\partial y} f(x, y) \right) u_{1,1,2,2} \right. \\ & + \left( \frac{\partial}{\partial x} f(x, y) \right) u_{1,2,2,2} \left. \right) D_{u_{1,2,2,2}} - \left( 6 \left( \frac{\partial^2}{\partial y^2} f(x, y) \right) u_{1,2,2} + 4 \left( \frac{\partial}{\partial y} f(x, y) \right) u_{1,2,2,2} \right. \\ & \left. \right) D_{u_{2,2,2,2}} - \left( 10 \left( \frac{\partial^2}{\partial x^2} f(x, y) \right) u_{1,1,1,1} + 5 \left( \frac{\partial}{\partial x} f(x, y) \right) u_{1,1,1,1,1} \right. \\ & \left. \right) D_{u_{1,1,1,1,1}} - \left( 4 \left( \frac{\partial^3}{\partial x^3} f(x, y) \right) u_{1,1,2} + 4 \left( \frac{\partial^2}{\partial y \partial x} f(x, y) \right) u_{1,1,1,1} \right. \\ & + 6 \left( \frac{\partial^2}{\partial x^2} f(x, y) \right) u_{1,1,1,2} + \left( \frac{\partial}{\partial y} f(x, y) \right) u_{1,1,1,1,1} + 4 \left( \frac{\partial}{\partial x} f(x, y) \right) u_{1,1,1,1,2} \left. \right) \\ & D_{u_{1,1,1,1,2}} - \left( 6 \left( \frac{\partial^3}{\partial y \partial x^2} f(x, y) \right) u_{1,1,2} + \left( \frac{\partial^3}{\partial x^3} f(x, y) \right) u_{1,2,2} + 6 \left( \frac{\partial^2}{\partial y \partial x} f(x, y) \right) u_{1,1,1,2} \right. \\ & + 3 \left( \frac{\partial^2}{\partial x^2} f(x, y) \right) u_{1,1,2,2} + \left( \frac{\partial^2}{\partial y^2} f(x, y) \right) u_{1,1,1,1} + 2 \left( \frac{\partial}{\partial y} f(x, y) \right) u_{1,1,1,1,2} \\ & + 3 \left( \frac{\partial}{\partial x} f(x, y) \right) u_{1,1,1,2,2} \left. \right) D_{u_{1,1,1,2,2}} - \left( 3 \left( \frac{\partial^3}{\partial y \partial x^2} f(x, y) \right) u_{1,2,2} + 6 \left( \frac{\partial^3}{\partial y^2 \partial x} f(x, y) \right) u_{1,1,2} \right. \\ & + 6 \left( \frac{\partial^2}{\partial y \partial x} f(x, y) \right) u_{1,1,2,2} + \left( \frac{\partial^2}{\partial x^2} f(x, y) \right) u_{1,2,2,2} + 3 \left( \frac{\partial^2}{\partial y^2} f(x, y) \right) u_{1,1,1,2} \\ & + 3 \left( \frac{\partial}{\partial y} f(x, y) \right) u_{1,1,1,2,2} + 2 \left( \frac{\partial}{\partial x} f(x, y) \right) u_{1,1,2,2,2} \left. \right) D_{u_{1,1,2,2,2}} - \left( 6 \left( \frac{\partial^3}{\partial y^2 \partial x} f(x, y) \right) u_{1,2,2} + 4 \left( \frac{\partial^2}{\partial y \partial x} f(x, y) \right) u_{1,2,2,2} \right. \\ & + 4 \left( \frac{\partial^3}{\partial y^3} f(x, y) \right) u_{1,1,2} + 6 \left( \frac{\partial^2}{\partial y^2} f(x, y) \right) u_{1,1,2,2} + 4 \left( \frac{\partial}{\partial y} f(x, y) \right) u_{1,1,2,2,2} \\ & + \left( \frac{\partial}{\partial x} f(x, y) \right) u_{1,1,2,2,2,2} \left. \right) D_{u_{1,2,2,2,2}} - \left( 10 \left( \frac{\partial^3}{\partial y^3} f(x, y) \right) u_{1,2,2} \right. \end{aligned} \tag{37}$$

$$+ 10 \left( \frac{\partial^2}{\partial y^2} f(x, y) \right) u_{1,2,2,2} + 5 \left( \frac{\partial}{\partial y} f(x, y) \right) u_{1,2,2,2} \right) D_{-} u_{2,2,2,2}$$

It is clear (from the expansion of the Lie Algebra Sheaf) that we get 2 new differential invariants every order  $> 2$ . So  $P(z) = z + z^2 + z^3 + 2z^4 + 2z^5 + \dots = \frac{z + z^4}{1 - z}$ .

>

5. Consider the singular statum  $S[5] = \{u_1 = 0, u_{1,1} = 0, u_{1,2} = 0, u_{1,1,1} = 0, u_{1,1,2} = 0\}$

>  $X4 := DGsimplify(subs([u_1 = 0, u_{1,1} = 0, u_{1,2} = 0, u_{1,1,1} = 0, u_{1,1,2} = 0],$   
 $Prolong(evalDG(f(x, y) \cdot D_{-}x), 4)))$

$$\begin{aligned} X4 := & f(x, y) D_{-}x - \left( \frac{\partial}{\partial x} f(x, y) \right) u_{1,2,2} D_{-}u_{1,2,2} - 3 \left( \frac{\partial}{\partial y} f(x, y) \right) u_{1,2,2} D_{-}u_{2,2,2} \\ & - 4 \left( \frac{\partial}{\partial x} f(x, y) \right) u_{1,1,1,1} D_{-}u_{1,1,1,1} - \left( \left( \frac{\partial}{\partial y} f(x, y) \right) u_{1,1,1,1} + 3 \left( \frac{\partial}{\partial x} f(x, \right. \right. \\ & \left. \left. y) \right) u_{1,1,1,2} \right) D_{-}u_{1,1,1,2} - \left( \left( \frac{\partial^2}{\partial x^2} f(x, y) \right) u_{1,2,2} + 2 \left( \frac{\partial}{\partial y} f(x, y) \right) u_{1,1,1,2} \right. \\ & \left. + 2 \left( \frac{\partial}{\partial x} f(x, y) \right) u_{1,1,2,2} \right) D_{-}u_{1,1,2,2} - \left( 3 \left( \frac{\partial^2}{\partial y \partial x} f(x, y) \right) u_{1,2,2} + 3 \left( \frac{\partial}{\partial y} f(x, \right. \right. \\ & \left. \left. y) \right) u_{1,1,2,2} + \left( \frac{\partial}{\partial x} f(x, y) \right) u_{1,2,2,2} \right) D_{-}u_{1,2,2,2} - \left( 6 \left( \frac{\partial^2}{\partial y^2} f(x, y) \right) u_{1,2,2} \right. \\ & \left. + 4 \left( \frac{\partial}{\partial y} f(x, y) \right) u_{1,2,2,2} \right) D_{-}u_{2,2,2,2} \end{aligned} \quad (38)$$

>  $simplify(LieDerivative(X4, u_2));$   
 $simplify(LieDerivative(X4, u_{2,2}));$   
 $RES3 := simplify(LieDerivative(X4, u_{2,2,2} - F(u_{1,2,2})));$   
 $RES4 := simplify(LieDerivative(X4, u_{2,2,2,2} - F(u_{1,1,1,1}, u_{1,1,1,2}, u_{1,1,2,2}, u_{1,2,2,2}, u_{1,1,2},$   
 $u_{1,2,2})))$

$$\begin{aligned} RES3 := & u_{1,2,2} \left( \left( \frac{\partial}{\partial x} f(x, y) \right) \left( \frac{d}{du_{1,2,2}} F(u_{1,2,2}) \right) - 3 \left( \frac{\partial}{\partial y} f(x, y) \right) \right) \\ RES4 := & \left( \frac{\partial}{\partial x} f(x, y) \right) u_{1,2,2} \left( \frac{\partial}{\partial u_{1,2,2}} F(u_{1,1,1,1}, u_{1,1,1,2}, u_{1,1,2,2}, u_{1,2,2,2}, u_{1,1,2}, \right. \\ & \left. u_{1,2,2}) \right) + 4 \left( \frac{\partial}{\partial x} f(x, y) \right) u_{1,1,1,1} \left( \frac{\partial}{\partial u_{1,1,1,1}} F(u_{1,1,1,1}, u_{1,1,1,2}, u_{1,1,2,2}, u_{1,2,2,2}, \right. \\ & \left. u_{1,1,2}, u_{1,2,2}) \right) + \left( \frac{\partial}{\partial u_{1,1,1,2}} F(u_{1,1,1,1}, u_{1,1,1,2}, u_{1,1,2,2}, u_{1,2,2,2}, u_{1,1,2}, \right. \\ & \left. u_{1,2,2}) \right) \left( \frac{\partial}{\partial y} f(x, y) \right) u_{1,1,1,1} + 3 \left( \frac{\partial}{\partial u_{1,1,1,2}} F(u_{1,1,1,1}, u_{1,1,1,2}, u_{1,1,2,2}, u_{1,2,2,2}, \right. \\ & \left. u_{1,1,2}, u_{1,2,2}) \right) \left( \frac{\partial}{\partial x} f(x, y) \right) u_{1,1,1,2} + \left( \frac{\partial}{\partial u_{1,1,2,2}} F(u_{1,1,1,1}, u_{1,1,1,2}, u_{1,1,2,2}, \right. \\ & \left. u_{1,2,2,2}, u_{1,1,2}, u_{1,2,2}) \right) \left( \frac{\partial^2}{\partial x^2} f(x, y) \right) u_{1,2,2} + 2 \left( \frac{\partial}{\partial u_{1,1,2,2}} F(u_{1,1,1,1}, u_{1,1,1,2}, \right. \end{aligned} \quad (39)$$

$$\begin{aligned}
& u_{1,1,2,2}, u_{1,2,2,2}, u_{1,1,2}, u_{1,2,2} \Big) \left( \frac{\partial}{\partial y} f(x, y) \right) u_{1,1,1,2} + 2 \left( \frac{\partial}{\partial u_{1,1,2,2}} F(u_{1,1,1,1}, \right. \\
& u_{1,1,1,2}, u_{1,1,2,2}, u_{1,2,2,2}, u_{1,1,2}, u_{1,2,2} \Big) \left( \frac{\partial}{\partial x} f(x, y) \right) u_{1,1,2,2} \\
& + 3 \left( \frac{\partial}{\partial u_{1,2,2,2}} F(u_{1,1,1,1}, u_{1,1,1,2}, u_{1,1,2,2}, u_{1,2,2,2}, u_{1,1,2}, u_{1,2,2} \Big) \left( \frac{\partial^2}{\partial y \partial x} f(x, \right. \right. \\
& y) \Big) u_{1,2,2} + 3 \left( \frac{\partial}{\partial u_{1,2,2,2}} F(u_{1,1,1,1}, u_{1,1,1,2}, u_{1,1,2,2}, u_{1,2,2,2}, u_{1,1,2}, \right. \\
& u_{1,2,2} \Big) \left( \frac{\partial}{\partial y} f(x, y) \right) u_{1,1,2,2} + \left( \frac{\partial}{\partial u_{1,2,2,2}} F(u_{1,1,1,1}, u_{1,1,1,2}, u_{1,1,2,2}, u_{1,2,2,2}, \right. \\
& u_{1,1,2}, u_{1,2,2} \Big) \left( \frac{\partial}{\partial x} f(x, y) \right) u_{1,2,2,2} - 6 \left( \frac{\partial^2}{\partial y^2} f(x, y) \right) u_{1,2,2} - 4 \left( \frac{\partial}{\partial y} f(x, \right. \\
& y) \Big) u_{1,2,2,2}
\end{aligned}$$

$$\begin{aligned}
& > \text{coeff} \left( \text{RES3}, \frac{\partial}{\partial y} f(x, y) \right) \\
& \qquad \qquad \qquad -3 u_{1,2,2} \tag{40}
\end{aligned}$$

$$\begin{aligned}
& > \text{coeff} \left( \text{RES4}, \frac{\partial^2}{\partial y^2} f(x, y) \right) \\
& \qquad \qquad \qquad -6 u_{1,2,2} \tag{41}
\end{aligned}$$

$$\begin{aligned}
& > \text{RES4} := \text{simplify}(\text{LieDerivative}(X4, F(u_{1,1,1,1}, u_{1,1,2}))) \\
& \text{RES4} := -2 \left( \frac{\partial}{\partial x} f(x, y) \right) \left( u_{1,1,2} \left( \frac{\partial}{\partial u_{1,1,2}} F(u_{1,1,1,1}, u_{1,1,2}) \right) \right. \\
& \quad \left. + 2 u_{1,1,1,1} \left( \frac{\partial}{\partial u_{1,1,1,1}} F(u_{1,1,1,1}, u_{1,1,2}) \right) \right) \tag{42}
\end{aligned}$$

$$\begin{aligned}
& > \text{pdsolve} \left( \frac{\%}{-2 \left( \frac{\partial}{\partial x} f(x, y) \right)} \right) \\
& \qquad \qquad \qquad F(u_{1,1,1,1}, u_{1,1,2}) = -FI \left( \frac{u_{1,1,2}}{\sqrt{u_{1,1,1,1}}} \right) \tag{43}
\end{aligned}$$

$$\begin{aligned}
& > \text{simplify} \left( \text{LieDerivative} \left( X4, \frac{u_{1,1,1,1}}{u_{1,1,2}^2} \right) \right) \\
& \qquad \qquad \qquad 0 \tag{44}
\end{aligned}$$

We see no invariants of order 3, but then we get 1 new diff.inv. every order starting from 4.

Therefore  $P(z) = z + z^2 + z^4 + z^5 + \dots = \frac{z - z^3 + z^4}{1 - z}$ .

>

6. Consider the singular statum  $S[6] = \{u_1 = 0, u_{1,1} = 0, u_{1,2} = 0, u_{1,1,1} = 0, u_{1,1,2} = 0, u_{1,2,2} = 0\}$

$$\begin{aligned}
& > X5 := \text{DGsimplify}(\text{subs}([u_1 = 0, u_{1,1} = 0, u_{1,2} = 0, u_{1,1,1} = 0, u_{1,1,2} = 0, u_{1,2,2} = 0], \\
& \quad \text{Prolong}(\text{evalDG}(f(x, y) \cdot D_x), 5))) \\
& X5 := f(x, y) D_x - 4 \left( \frac{\partial}{\partial x} f(x, y) \right) u_{1,1,1,1} D_{u_{1,1,1,1}} - \left( \left( \frac{\partial}{\partial y} f(x, y) \right) u_{1,1,1,1} \right. \tag{45}
\end{aligned}$$

$$\begin{aligned}
& + 3 \left( \frac{\partial}{\partial x} f(x, y) \right) u_{1, 1, 1, 2} \Big) D_{-} u_{1, 1, 1, 2} - \left( 2 \left( \frac{\partial}{\partial y} f(x, y) \right) u_{1, 1, 1, 2} + 2 \left( \frac{\partial}{\partial x} f(x, \right. \right. \\
& y) \Big) u_{1, 1, 2, 2} \Big) D_{-} u_{1, 1, 2, 2} - \left( 3 \left( \frac{\partial}{\partial y} f(x, y) \right) u_{1, 1, 2, 2} + \left( \frac{\partial}{\partial x} f(x, \right. \right. \\
& y) \Big) u_{1, 2, 2, 2} \Big) D_{-} u_{1, 2, 2, 2} - 4 \left( \frac{\partial}{\partial y} f(x, y) \right) u_{1, 2, 2, 2} D_{-} u_{2, 2, 2, 2} - \left( 10 \left( \frac{\partial^2}{\partial x^2} f(x, \right. \right. \\
& y) \Big) u_{1, 1, 1, 1} + 5 \left( \frac{\partial}{\partial x} f(x, y) \right) u_{1, 1, 1, 1, 1} \Big) D_{-} u_{1, 1, 1, 1, 1} - \left( 4 \left( \frac{\partial^2}{\partial y \partial x} f(x, y) \right) u_{1, 1, 1, 1} \right. \\
& + 6 \left( \frac{\partial^2}{\partial x^2} f(x, y) \right) u_{1, 1, 1, 2} + \left( \frac{\partial}{\partial y} f(x, y) \right) u_{1, 1, 1, 1, 1} + 4 \left( \frac{\partial}{\partial x} f(x, y) \right) u_{1, 1, 1, 1, 2} \Big) \\
& D_{-} u_{1, 1, 1, 1, 2} - \left( 6 \left( \frac{\partial^2}{\partial y \partial x} f(x, y) \right) u_{1, 1, 1, 2} + 3 \left( \frac{\partial^2}{\partial x^2} f(x, y) \right) u_{1, 1, 2, 2} + \left( \frac{\partial^2}{\partial y^2} f(x, \right. \right. \\
& y) \Big) u_{1, 1, 1, 1} + 2 \left( \frac{\partial}{\partial y} f(x, y) \right) u_{1, 1, 1, 1, 2} + 3 \left( \frac{\partial}{\partial x} f(x, y) \right) u_{1, 1, 1, 2, 2} \Big) D_{-} u_{1, 1, 1, 2, 2} \\
& - \left( 6 \left( \frac{\partial^2}{\partial y \partial x} f(x, y) \right) u_{1, 1, 2, 2} + \left( \frac{\partial^2}{\partial x^2} f(x, y) \right) u_{1, 2, 2, 2} + 3 \left( \frac{\partial^2}{\partial y^2} f(x, y) \right) u_{1, 1, 1, 2} \right. \\
& + 3 \left( \frac{\partial}{\partial y} f(x, y) \right) u_{1, 1, 1, 2, 2} + 2 \left( \frac{\partial}{\partial x} f(x, y) \right) u_{1, 1, 2, 2, 2} \Big) D_{-} u_{1, 1, 2, 2, 2} \\
& - \left( 4 \left( \frac{\partial^2}{\partial y \partial x} f(x, y) \right) u_{1, 2, 2, 2} + 6 \left( \frac{\partial^2}{\partial y^2} f(x, y) \right) u_{1, 1, 2, 2} + 4 \left( \frac{\partial}{\partial y} f(x, \right. \right. \\
& y) \Big) u_{1, 1, 2, 2, 2} + \left( \frac{\partial}{\partial x} f(x, y) \right) u_{1, 2, 2, 2, 2} \Big) D_{-} u_{1, 2, 2, 2, 2} - \left( 10 \left( \frac{\partial^2}{\partial y^2} f(x, y) \right) u_{1, 2, 2, 2} \right. \\
& + 5 \left( \frac{\partial}{\partial y} f(x, y) \right) u_{1, 2, 2, 2, 2} \Big) D_{-} u_{2, 2, 2, 2, 2}
\end{aligned}$$

Even without calculations it is visible here that there are 3 differential invariants in every order  $> 3$ ,  
whence  $P(z) = z + z^2 + z^3 + 3z^4 + 3z^5 + \dots = \frac{z + 2z^4}{1 - z}$ .

>

This will continue with all infinite strata of finite codimension until we arrive to the infinite stratum  $S[\infty] = \{u_1 = 0, u_{1,1} = 0, u_{1,2} = 0, u_{1,1,1} = 0, u_{1,1,2} = 0, u_{1,2,2} = 0, \dots\} = E^\infty(\infty)$ , where  $E$  is the equation  $[u_1 = 0]$ .

For this equation all  $u_2, u_{2,2}, u_{2,2,2}, \dots$  are invariants **and** so  $P(z) = z + z^2 + z^3 + z^4 + z^5 + \dots = \frac{z + 2z^4}{1 - z}$

>

$\mathbb{R}^3(u_{1,1}, u_{1,2}, u_{2,2})$

>  $DGsetup([r, s, t], M) :$

>  $pdsolve([2r \operatorname{diff}(F(r, s, t), r) + s \operatorname{diff}(F(r, s, t), s) = 0, r \operatorname{diff}(F(r, s, t), s) + 2s \operatorname{diff}(F(r, s, t), t) = 0])$

$$\left\{ F(r, s, t) = \_FI \left( \frac{-s^2 + tr}{r} \right) \right\} \quad (46)$$

>  $c1 := [x, x*y, 5 + x*y^2] : c2 := [x, x*y, -5 + x*y^2] : c3 := [x, x*y, x*y^2] : c4 := [0, 5*x, 3*y] : c5 := [0, 0, 2*x*y] :$   
 $plot3d(\{c1, c2, c3, c4, c5\}, x = -2..2, y = -2..2, grid = [25, 15], color = \sin(x)) ;$

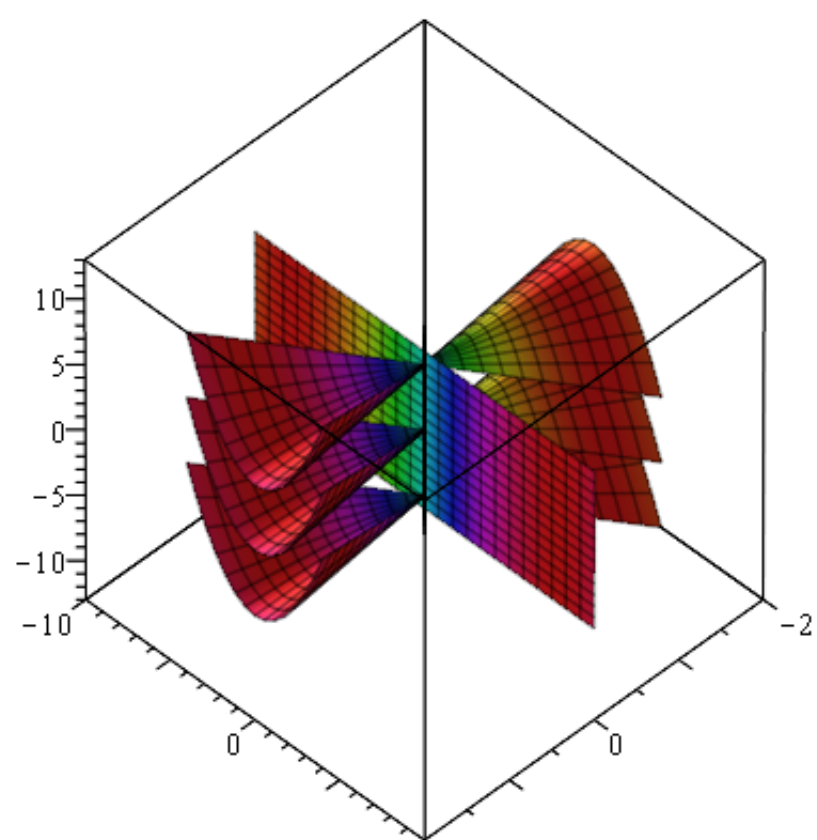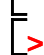

Supplement: Supplementary file 4 [file Ex_of_higher_singularities_and_Poincare_function.pdf]
