# Supplementary material for: Poincare function for moduli of differential-geometric structures
Source: arXiv:1802.01322 source file (2018-02-05)
Supplement: Supplementary file 5 [file VF2Dsing-2017.pdf]

```

> with(DifferentialGeometry) : Preferences("ShowFramePrompt",false) :
> DGsetup([x, y], M) :
In this worksheet we compute the number of differential invariants depending on order for the
vector field  $v(x, y) = y \cdot D_x + x \cdot (x \cdot a(x) + y \cdot b(x)) \cdot D_y$  singular at the origin.
> n := 20 :
> A := add(a[i] x^i, i=0..n) : B := add(b[i] x^i, i=0..n) : C := x \cdot A + y \cdot B :
P := (add(add(p[i, j] x^i y^j, j=0..n), i=0..n)) : Q := y \cdot diff(P, x) + x \cdot C \cdot diff(P, y) :
> u := evalDG(P \cdot D_x + Q \cdot D_y) : v := evalDG(y \cdot D_x + x \cdot C \cdot D_y) :
> w := LieDerivative(u, v) :
> LieDerivative(w, x)
0 (1)
> ineq := {a_0 \neq 0, b_0 \neq 0} :
> ss := {} :
>
> m := 1 :
wY := LieDerivative(w, y) : Y := (i, j) \rightarrow subs(ss, subs({x=0, y=0}, diff(wY, x$ i, y$ j))) :
Y(0, 0) := subs({x=0, y=0}, wY) :
simplify([seq([seq(Y(k-i, i), i=0..k)], k=0..m)])
[0], [2 a_0 p_{0,0}, b_0 p_{0,0}] (2)
> ss := {p_{0,0}=0} :
>
> m := 2 :
wY := LieDerivative(w, y) : Y := (i, j) \rightarrow subs(ss, subs({x=0, y=0}, diff(wY, x$ i, y$ j))) :
Y(0, 0) := subs({x=0, y=0}, wY) :
simplify([seq([seq(Y(k-i, i), i=0..k)], k=0..m)])
[0], [0, 0], [2 a_0 p_{1,0}, b_0 p_{1,0}, -4 p_{2,0}] (3)
> ss := ss union {b_0=1, p_{2,0}=0, p_{1,0}=0}
ss := {b_0=1, p_{0,0}=0, p_{1,0}=0, p_{2,0}=0} (4)
> m := 3 :
wY := LieDerivative(w, y) : Y := (i, j) \rightarrow subs(ss, subs({x=0, y=0}, diff(wY, x$ i, y$ j))) :
Y(0, 0) := subs({x=0, y=0}, wY) :
simplify([seq([seq(Y(k-i, i), i=0..k)], k=0..m)])
[0], [0, 0], [0, 0, 0], [0, -6 a_0 p_{1,1}, -4 a_0 p_{0,2} - 4 p_{1,1} - 12 p_{3,0}, -6 p_{0,2} - 12 p_{2,1}] (5)
> solve(%[-1], {p_{1,1}, p_{2,1}, p_{3,0}})
{p_{1,1}=0, p_{2,1}=-\frac{1}{2} p_{0,2}, p_{3,0}=-\frac{1}{3} a_0 p_{0,2}} (6)
> ss := ss union {b_1=0, op(%)}
ss := {b_0=1, b_1=0, p_{0,0}=0, p_{1,0}=0, p_{1,1}=0, p_{2,0}=0, p_{2,1}=-\frac{1}{2} p_{0,2}, p_{3,0}=-\frac{1}{3} a_0 p_{0,2}} (7)
>
> m := 4 :
wY := LieDerivative(w, y) : Y := (i, j) \rightarrow subs(ss, subs({x=0, y=0}, diff(wY, x$ i, y$ j))) :
Y(0, 0) := subs({x=0, y=0}, wY) :
simplify([seq([seq(Y(k-i, i), i=0..k)], k=0..m)])
[0], [0, 0], [0, 0, 0], [0, 0, 0, 0], [-40 a_0^2 p_{0,2}, -8 a_0 p_{0,2}, -28 a_0 p_{1,2} - 12 a_1 p_{0,2} - 48 p_{4,0} - 24 a_0 p_{0,3} - 30 p_{1,2} - 36 p_{3,1}, -48 p_{0,3} - 48 p_{2,2}] (8)

```

$$\begin{aligned} &> \text{solve}(\%[-1], \{p_{0,2}, \text{seq}(p_{k,m-k} \ k=2..m)\}) \\ &\quad \left\{ p_{0,2}=0, p_{2,2}=-p_{0,3}, p_{3,1}=-\frac{2}{3} a_0 p_{0,3} - \frac{5}{6} p_{1,2}, p_{4,0}=-\frac{7}{12} a_0 p_{1,2} \right\} \end{aligned} \quad (9)$$

$$\begin{aligned} &> ss := \text{subs}(\%[1..1], ss) \text{ union } \{b_2=0, \text{op}(\%)\} \\ ss &:= \left\{ b_0=1, b_1=0, b_2=0, p_{0,0}=0, p_{0,2}=0, p_{1,0}=0, p_{1,1}=0, p_{2,0}=0, p_{2,1}=0, p_{2,2}= \right. \\ &\quad \left. -p_{0,3}, p_{3,0}=0, p_{3,1}=-\frac{2}{3} a_0 p_{0,3} - \frac{5}{6} p_{1,2}, p_{4,0}=-\frac{7}{12} a_0 p_{1,2} \right\} \end{aligned} \quad (10)$$

$$\begin{aligned} &> m := 5 : \\ wY &:= \text{LieDerivative}(w, y) : Y := (i, j) \rightarrow \text{subs}(ss, \text{subs}(\{x=0, y=0\}, \text{diff}(wY, x\$i, y\$j))) : \\ Y(0, 0) &:= \text{subs}(\{x=0, y=0\}, wY) : \\ \text{simplify} &([\text{seq}([\text{seq}(Y(k-i, i), i=0..k)], k=0..m)]) \\ &[[0], [0, 0], [0, 0, 0], [0, 0, 0, 0], [0, 0, 0, 0, 0], [-100 a_0^2 p_{1,2}, 70 a_0 p_{1,2}, 48 a_0 p_{0,3} \\ &\quad -96 a_1 p_{1,2} + 36 p_{1,2} - 240 p_{5,0}, -132 a_0 p_{1,3} - 72 a_1 p_{0,3} + 36 p_{0,3} - 144 p_{4,1}, \\ &\quad -144 a_0 p_{0,4} - 192 p_{1,3} - 144 p_{3,2}, -360 p_{0,4} - 240 p_{2,3}]] \end{aligned} \quad (11)$$

$$\begin{aligned} &> \text{solve}(\%[-1], \{p_{1,2}, \text{seq}(p_{k,m-k} \ k=2..m)\}) \\ &\quad \left\{ p_{1,2}=0, p_{2,3}=-\frac{3}{2} p_{0,4}, p_{3,2}=-a_0 p_{0,4} - \frac{4}{3} p_{1,3}, p_{4,1}=-\frac{11}{12} a_0 p_{1,3} - \frac{1}{2} a_1 p_{0,3} \right. \\ &\quad \left. + \frac{1}{4} p_{0,3}, p_{5,0}=\frac{1}{5} a_0 p_{0,3} \right\} \end{aligned} \quad (12)$$

$$\begin{aligned} &> ss := \text{subs}(\%[1..1], ss) \text{ union } \{b_3=0, \text{op}(\%)\} \\ ss &:= \left\{ b_0=1, b_1=0, b_2=0, b_3=0, p_{0,0}=0, p_{0,2}=0, p_{1,0}=0, p_{1,1}=0, p_{1,2}=0, p_{2,0}=0, p_{2,1} \right. \\ &\quad =0, p_{2,2}=-p_{0,3}, p_{2,3}=-\frac{3}{2} p_{0,4}, p_{3,0}=0, p_{3,1}=-\frac{2}{3} a_0 p_{0,3}, p_{3,2}=-a_0 p_{0,4} \\ &\quad \left. -\frac{4}{3} p_{1,3}, p_{4,0}=0, p_{4,1}=-\frac{11}{12} a_0 p_{1,3} - \frac{1}{2} a_1 p_{0,3} + \frac{1}{4} p_{0,3}, p_{5,0}=\frac{1}{5} a_0 p_{0,3} \right\} \end{aligned} \quad (13)$$

$$\begin{aligned} &> m := 6 : \\ wY &:= \text{LieDerivative}(w, y) : Y := (i, j) \rightarrow \text{subs}(ss, \text{subs}(\{x=0, y=0\}, \text{diff}(wY, x\$i, y\$j))) : \\ Y(0, 0) &:= \text{subs}(\{x=0, y=0\}, wY) : \\ \text{simplify} &([\text{seq}([\text{seq}(Y(k-i, i), i=0..k)], k=0..m)]) \\ &[[0], [0, 0], [0, 0, 0], [0, 0, 0, 0], [0, 0, 0, 0, 0], [0, 0, 0, 0, 0, 0], [1008 a_0^2 p_{0,3}, 600 a_0^2 p_{1,3} \\ &\quad + 144 a_0 p_{0,3}, 240 a_0^2 p_{0,4} + 864 a_0 p_{1,3} + 240 a_1 p_{0,3} - 1440 p_{6,0}, 576 a_0 p_{0,4} \\ &\quad - 468 a_1 p_{1,3} - 288 a_2 p_{0,3} + 408 p_{1,3} - 720 p_{5,1}, -720 a_0 p_{1,4} - 432 a_1 p_{0,4} \\ &\quad + 432 p_{0,4} - 576 p_{4,2}, -960 a_0 p_{0,5} - 1320 p_{1,4} - 720 p_{3,3}, -2880 p_{0,5} - 1440 p_{2,4}]] \end{aligned} \quad (14)$$

$$\begin{aligned} &> \text{solve}(\%[-1], \{p_{0,3}, p_{1,3}, \text{seq}(p_{k,m-k} \ k=2..m)\}) \\ &\quad \left\{ p_{0,3}=0, p_{1,3}=0, p_{2,4}=-2 p_{0,5}, p_{3,3}=-\frac{4}{3} a_0 p_{0,5} - \frac{11}{6} p_{1,4}, p_{4,2}=-\frac{5}{4} a_0 p_{1,4} \right. \\ &\quad \left. -\frac{3}{4} a_1 p_{0,4} + \frac{3}{4} p_{0,4}, p_{5,1}=\frac{4}{5} a_0 p_{0,4}, p_{6,0}=\frac{1}{6} a_0^2 p_{0,4} \right\} \end{aligned} \quad (15)$$

$$\begin{aligned} &> ss := \text{subs}(\%[1..2], ss) \text{ union } \{a_4=0, b_4=0, \text{op}(\%)\} \end{aligned} \quad (16)$$

$$_{SS} := \left\{ a_4 = 0, b_0 = 1, b_1 = 0, b_2 = 0, b_3 = 0, b_4 = 0, p_{0,0} = 0, p_{0,2} = 0, p_{0,3} = 0, p_{1,0} = 0, p_{1,1} = 0, p_{1,2} = 0, p_{1,3} = 0, p_{2,0} = 0, p_{2,1} = 0, p_{2,2} = 0, p_{2,3} = -\frac{3}{2} p_{0,4}, p_{2,4} = -2 p_{0,5}, p_{3,0} = 0, p_{3,1} = 0, p_{3,2} = -a_0 p_{0,4}, p_{3,3} = -\frac{4}{3} a_0 p_{0,5} - \frac{11}{6} p_{1,4}, p_{4,0} = 0, p_{4,1} = 0, p_{4,2} = -\frac{5}{4} a_0 p_{1,4} - \frac{3}{4} a_1 p_{0,4} + \frac{3}{4} p_{0,4} p_{5,0} = 0, p_{5,1} = \frac{4}{5} a_0 p_{0,4}, p_{6,0} = \frac{1}{6} a_0^2 p_{0,4} \right\} \quad (16)$$

>

```

> solve(%[-1], {p0, 5, p1, 5, seq(pk, m-k | k=2..m)}) :
ss := subs(%[1..2], ss) union {a7=0, b7=0, op(%)} :

```

$$\left[ [0], [0, 0], [0, 0, 0], [0, 0, 0, 0], [0, 0, 0, 0, 0], [0, 0, 0, 0, 0, 0], [0, 0, 0, 0, 0, 0, 0], [0, \right. \quad (20)$$

```

> solve(%[-1], {p0, 6, seq(p_k m - k k=2..m)}) :
ss := subs(%[1..1], ss) union {b8=0, op(%) } :

```

171\

$$\begin{aligned}
& \left[ [0], [0, 0], [0, 0, 0], [0, 0, 0, 0], [0, 0, 0, 0, 0], [0, 0, 0, 0, 0, 0], [0, 0, 0, 0, 0, 0, 0], [0, \right. \\
& \quad 0, 0, 0, 0, 0, 0, 0], [0, 0, 0, 0, 0, 0, 0, 0], [0, 0, 0, 0, 0, 0, 0, 0, 0], [0, 0, 0, 0, 0, 0, \\
& \quad 0, 0, 0, 0, 0], \left[ -19747200 a_0^4 p_{1,6}, 57140400 a_0^3 p_{1,6}, 14938560 a_0^3 p_{0,7} - 40735440 \right. \\
& \quad a_0^2 a_1 p_{1,6} + 58417632 a_0^2 p_{1,6} - 79833600 p_{11,0} - 12009600 a_0^3 p_{1,7} - 14515200 \\
& \quad a_0^2 a_1 p_{0,7} + 22397472 a_0^2 p_{0,7} - 53937432 a_0 a_1 p_{1,6} + 27952992 a_0 p_{1,6} \\
& \quad - 21772800 p_{10,1}, -5644800 a_0^3 p_{0,8} - 29664000 a_0^2 p_{1,7} - 27385344 a_0 a_1 p_{0,7} \\
& \quad + 11854080 a_0 a_2 p_{1,6} + 5515776 a_1^2 p_{1,6} + 15220224 a_0 p_{0,7} - 22105152 a_1 p_{1,6} \\
& \quad + 6077376 p_{1,6} - 8709120 p_{9,2}, -19333440 a_0^2 p_{0,8} + 12610080 a_0 a_1 p_{1,7} \\
& \quad + 7741440 a_0 a_2 p_{0,7} + 3628800 a_1^2 p_{0,7} - 30790080 a_0 p_{1,7} - 15422400 a_1 p_{0,7} \\
& \quad + 11658240 a_2 p_{1,6} + 4536000 p_{0,7} - 4838400 p_{8,3}, 9000000 a_0^2 p_{1,8} \\
& \quad + 10584000 a_0 a_1 p_{0,8} - 27155520 a_0 p_{0,8} + 15992640 a_1 p_{1,7} + 10264320 a_2 p_{0,7} \\
& \quad - 3283200 a_3 p_{1,6} - 13443840 p_{1,7} - 3628800 p_{7,4}, 9676800 a_0^2 p_{0,9} \\
& \quad + 29443680 a_0 p_{1,8} + 17992800 a_1 p_{0,8} - 4717440 a_2 p_{1,7} - 3628800 a_3 p_{0,7} \\
& \quad - 15876000 p_{0,8} - 3628800 p_{6,5}, 42577920 a_0 p_{0,9} - 9192960 a_1 p_{1,8} \\
& \quad - 6773760 a_2 p_{0,8} + 30965760 p_{1,8} - 4838400 p_{5,6}, -25401600 a_0 p_{1,9} \\
& \quad - 17418240 a_1 p_{0,9} + 60963840 p_{0,9} - 8709120 p_{4,7}, -65318400 a_0 p_{0,10} \\
& \quad \left. - 94348800 p_{1,9} - 21772800 p_{3,8}, -359251200 p_{0,10} - 79833600 p_{2,9} \right] ]
\end{aligned}$$

(21)

> solve(%[-1], {p<sub>1,6</sub>, seq(p<sub>k,m-k</sub> k=2..m)}) :  
ss := subs(%[1..1], ss) **union**{b<sub>9</sub>=0, op(%)} :

>

> m := 12 :  
wY := LieDerivative(w, y) : Y := (i, j) → subs(ss, subs({x=0, y=0}, diff(wY, x\$ i, y\$ j))) :  
Y(0, 0) := subs({x=0, y=0}, wY) :  
simplify([seq([seq(Y(k-i, i), i=0..k)], k=0..m)])

$$\begin{aligned}
& \left[ [0], [0, 0], [0, 0, 0], [0, 0, 0, 0], [0, 0, 0, 0, 0], [0, 0, 0, 0, 0, 0], [0, 0, 0, 0, 0, 0, 0], [0, \right. \\
& \quad 0, 0, 0, 0, 0, 0, 0], [0, 0, 0, 0, 0, 0, 0, 0], [0, 0, 0, 0, 0, 0, 0, 0, 0], [0, 0, 0, 0, 0, 0, \\
& \quad 0, 0, 0, 0, 0, 0], [0, 0, 0, 0, 0, 0, 0, 0, 0, 0], \left[ 1165207680 a_0^4 p_{0,7}, 232848000 a_0^4 p_{1,7} \right. \\
& \quad + 89631360 a_0^3 p_{0,7}, 51744000 a_0^4 p_{0,8} + 568675200 a_0^3 p_{1,7} + 415356480 a_0^2 a_1 p_{0,7} \\
& \quad - 139518720 a_0^2 p_{0,7} - 958003200 p_{12,0}, 188112960 a_0^3 p_{0,8} - 286506720 a_0^2 a_1 p_{1,7} \\
& \quad - 127733760 a_0^2 a_2 p_{0,7} - 119750400 a_0 a_1^2 p_{0,7} + 565655040 a_0^2 p_{1,7} \\
& \quad + 386424000 a_0 a_1 p_{0,7} - 78874560 a_0 p_{0,7} - 239500800 p_{11,1}, -90604800 a_0^3 p_{1,8} \\
& \quad - 127008000 a_0^2 a_1 p_{0,8} + 265120128 a_0^2 p_{0,8} - 438267456 a_0 a_1 p_{1,7} \\
& \quad - 221958144 a_0 a_2 p_{0,7} - 104509440 a_1^2 p_{0,7} + 303025536 a_0 p_{1,7} + 120839040 a_1 p_{0,7} \\
& \quad \left. - 16329600 p_{0,7} - 87091200 p_{10,2}, -51609600 a_0^3 p_{0,9} - 260521920 a_0^2 p_{1,8} \right]
\end{aligned}$$

(22)



$$\begin{aligned}
& -1226534400 a_2 p_{0,8} + 933638400 p_{1,8} - 261273600 p_{9,4} - 2181997440 a_0^2 p_{0,10} \\
& + 981771840 a_0 a_1 p_{1,9} + 650280960 a_0 a_2 p_{0,9} + 304819200 a_1^2 p_{0,9} \\
& - 3386396160 a_0 p_{1,9} - 1913587200 a_1 p_{0,9} + 972518400 a_2 p_{1,8} + 681609600 a_3 p_{0,8} \\
& + 889056000 p_{0,9} - 203212800 p_{8,5} + 853977600 a_0^2 p_{1,10} + 1066867200 a_0 a_1 p_{0,10} \\
& - 3814594560 a_0 p_{0,10} + 1603445760 a_1 p_{1,9} + 1091543040 a_2 p_{0,9} \\
& - 251596800 a_3 p_{1,8} - 1884072960 p_{1,9} - 203212800 p_{7,6} + 1161216000 a_0^2 p_{0,11} \\
& + 3514855680 a_0 p_{1,10} + 2253484800 a_1 p_{0,10} - 444165120 a_2 p_{1,9} \\
& - 348364800 a_3 p_{0,9} - 2743372800 p_{0,10} - 261273600 p_{6,7} + 6241536000 a_0 p_{0,11} \\
& - 1045094400 a_1 p_{1,10} - 783820800 a_2 p_{0,10} + 4565030400 p_{1,10} - 435456000 p_{5,8} \\
& - 3432844800 a_0 p_{1,11} - 2395008000 a_1 p_{0,11} + 10777536000 p_{0,11} - 958003200 p_{4,9} \\
& - 10538035200 a_0 p_{0,12} - 15328051200 p_{1,11} - 2874009600 p_{3,10} \\
& - 68497228800 p_{0,12} - 12454041600 p_{2,11} ] ]
\end{aligned}$$

> solve( %[ -1 ], { p<sub>0,8</sub>, seq( p<sub>k,m-k</sub> k=2..m ) } ) :  
ss := subs( %[ 1..1 ], ss ) union { b<sub>11</sub> = 0, op( % ) } :

>

> m := 14 :  
wY := LieDerivative( w, y ) : Y := ( i, j ) → subs( ss, subs( { x = 0, y = 0 }, diff( wY, x\$ i, y\$ j ) ) ) :  
Y( 0, 0 ) := subs( { x = 0, y = 0 }, wY ) :  
simplify( [ seq( [ seq( Y( k - i, i ), i = 0..k ), k = 0..m ) ] ] )

$$\begin{aligned}
& [ [ 0 ], [ 0, 0 ], [ 0, 0, 0 ], [ 0, 0, 0, 0 ], [ 0, 0, 0, 0, 0 ], [ 0, 0, 0, 0, 0, 0 ], [ 0, 0, 0, 0, 0, 0, 0 ], [ 0, \\
& 0, 0, 0, 0, 0, 0, 0 ], [ 0, 0, 0, 0, 0, 0, 0, 0 ], [ 0, 0, 0, 0, 0, 0, 0, 0, 0 ], [ 0, 0, 0, 0, 0, 0, 0, 0, 0, 0 ], \\
& 0, 0, 0, 0, 0 ], [ 0, 0, 0, 0, 0, 0, 0, 0, 0, 0 ], [ 0, 0, 0, 0, 0, 0, 0, 0, 0, 0, 0 ], [ 0, 0, \\
& 0, 0, 0, 0, 0, 0 ], [ 0, 0, 0, 0, 0, 0, 0, 0, 0, 0, 0 ], [ 0, 0, 0, 0, 0, 0, 0, 0, 0, 0, 0, 0 ], [ 0, 0, \\
& 0, 0, 0, 0, 0, 0, 0, 0, 0, 0, 0 ], [ 31792992000 a_0^5 p_{1,8} - 126089275200 a_0^4 p_{1,8} \\
& - 25893504000 a_0^4 p_{0,9} + 78177153600 a_0^3 a_1 p_{1,8} - 154549489536 a_0^3 p_{1,8} \\
& - 174356582400 p_{14,0} + 15136070400 a_0^4 p_{1,9} + 22140518400 a_0^3 a_1 p_{0,9} \\
& - 46006272000 a_0^3 p_{0,9} + 138679756704 a_0^2 a_1 p_{1,8} - 97272080064 a_0^2 p_{1,8} \\
& - 37362124800 p_{13,1} + 5588352000 a_0^4 p_{0,10} + 42806949120 a_0^3 p_{1,9} + 54552960000 \\
& a_0^2 a_1 p_{0,9} - 20460211200 a_0^2 a_2 p_{1,8} - 19070251200 a_0 a_1^2 p_{1,8} - 40213324800 a_0^2 p_{0,9} \\
& + 97814852928 a_0 a_1 p_{1,8} - 35972546688 a_0 p_{1,8} - 11496038400 p_{12,2} + 21242995200 \\
& a_0^3 p_{0,10} - 18329587200 a_0^2 a_1 p_{1,9} - 10218700800 a_0^2 a_2 p_{0,9} - 9580032000 a_0 a_1^2 p_{0,9} \\
& + 55139149440 a_0^2 p_{1,9} + 51349248000 a_0 a_1 p_{0,9} - 33632478720 a_0 a_2 p_{1,8} \\
& - 15725145600 a_1^2 p_{1,8} - 19833984000 a_0 p_{0,9} + 27815097600 a_1 p_{1,8} \\
& - 6382800000 p_{1,8} - 4790016000 p_{11,3} - 7038144000 a_0^3 p_{1,10} - 11430720000 \\
& a_0^2 a_1 p_{0,10} + 35744094720 a_0^2 p_{0,10} - 37135100160 a_0 a_1 p_{1,9} - 21857402880 a_0 a_2 p_{0,9}
\end{aligned} \tag{24}$$

$$\begin{aligned}
& + 6153408000 a_0 a_3 p_{1,8} - 10276761600 a_1^2 p_{0,9} + 5486745600 a_1 a_2 p_{1,8} \\
& + 38294415360 a_0 p_{1,9} + 18985881600 a_1 p_{0,9} - 16808601600 a_2 p_{1,8} \\
& - 4572288000 p_{0,9} - 2612736000 p_{10,4} - 5419008000 a_0^3 p_{0,11} - 26270213760 \\
& a_0^2 p_{1,10} - 29750353920 a_0 a_1 p_{0,10} + 6970199040 a_0 a_2 p_{1,9} + 4877107200 a_0 a_3 p_{0,9} \\
& + 3250134720 a_1^2 p_{1,9} + 4389396480 a_1 a_2 p_{0,9} + 31875379200 a_0 p_{0,10} \\
& - 22863193920 a_1 p_{1,9} - 13992652800 a_2 p_{0,9} + 7256995200 a_3 p_{1,8} \\
& + 12087532800 p_{1,9} - 1828915200 p_{9,5} - 25808025600 a_0^2 p_{0,11} \\
& + 10069194240 a_0 a_1 p_{1,10} + 6827950080 a_0 a_2 p_{0,10} + 3200601600 a_1^2 p_{0,10} \\
& - 39789066240 a_0 p_{1,10} - 23318668800 a_1 p_{0,10} + 10199347200 a_2 p_{1,9} \\
& + 7315660800 a_3 p_{0,9} + 12802406400 p_{0,10} - 1625702400 p_{8,6} - 9565516800 a_0^2 p_{1,11} \\
& + 12192768000 a_0 a_1 p_{0,11} - 49729075200 a_0 p_{0,11} + 18302215680 a_1 p_{1,10} \\
& + 12697896960 a_2 p_{0,10} - 2569190400 a_3 p_{1,9} - 24561895680 p_{1,10} \\
& - 1828915200 p_{7,7} - 14370048000 a_0^2 p_{0,12} + 43429478400 a_0 p_{1,11} \\
& + 28304640000 a_1 p_{0,11} - 4964198400 a_2 p_{1,10} - 3919104000 a_3 p_{0,10} \\
& - 39191040000 p_{0,11} - 2612736000 p_{6,8} - 84304281600 a_0 p_{0,12} \\
& - 12693542400 a_1 p_{1,11} - 9580032000 a_2 p_{0,11} + 61791206400 p_{1,11} \\
& - 4790016000 p_{5,9} - 45026150400 a_0 p_{1,12} - 31614105600 a_1 p_{0,12} \\
& + 158070528000 p_{0,12} - 11496038400 p_{4,10} - 149448499200 a_0 p_{0,13} \\
& - 217945728000 p_{1,12} - 37362124800 p_{3,11} - 1046139494400 p_{0,13} \\
& - 174356582400 p_{2,12} ] ]
\end{aligned}$$

> solve( %[-1], {p<sub>1,8</sub>, seq(p<sub>k,m-k</sub> k=2..m)} ) :  
ss := subs( %[1..1], ss) **union** {b<sub>12</sub>=0, op(%) } :

>

> m := 15 :  
wY := LieDerivative(w, y) : Y := (i, j) → subs(ss, subs( {x=0, y=0}, diff(wY, x\$i, y\$j) ) ) :  
Y(0, 0) := subs( {x=0, y=0}, wY) :  
simplify( [seq( [seq( Y(k-i, i), i=0..k) ], k=0..m) ] )

$$\begin{aligned}
& [ [0], [0, 0], [0, 0, 0], [0, 0, 0, 0], [0, 0, 0, 0, 0], [0, 0, 0, 0, 0, 0], [0, 0, 0, 0, 0, 0, 0], [0, \\
& 0, 0, 0, 0, 0, 0, 0], [0, 0, 0, 0, 0, 0, 0, 0], [0, 0, 0, 0, 0, 0, 0, 0, 0], [0, 0, 0, 0, 0, 0, \\
& 0, 0, 0, 0, 0], [0, 0, 0, 0, 0, 0, 0, 0, 0, 0], [0, 0, 0, 0, 0, 0, 0, 0, 0, 0], [0, 0, \\
& 0, 0, 0, 0, 0, 0, 0, 0, 0, 0, 0], [0, 0, 0, 0, 0, 0, 0, 0, 0, 0, 0, 0], [ \\
& -3107220480000 a_0^5 p_{0,9} - 466161696000 a_0^5 p_{1,9} - 194201280000 a_0^4 p_{0,9} \\
& - 84756672000 a_0^5 p_{0,10} - 1314349545600 a_0^4 p_{1,9} - 1189895616000 a_0^3 a_1 p_{0,9} \\
& + 609902092800 a_0^3 p_{0,9} - 2615348736000 p_{15,0} - 349552869120 a_0^4 p_{0,10} \\
& + 615899531520 a_0^3 a_1 p_{1,9} + 247973806080 a_0^3 a_2 p_{0,9} + 348713164800 a_0^2 a_1^2 p_{0,9}
\end{aligned} \tag{25}$$



$$\begin{aligned}
& -1555465339584 a_0^3 p_{1,9} - 1498746412800 a_0^2 a_1 p_{0,9} + 440103456000 a_0^2 p_{0,9} \\
& - 523069747200 p_{14,1}, 126965836800 a_0^4 p_{1,10} + 217945728000 a_0^3 a_1 p_{0,10} \\
& - 573788427264 a_0^3 p_{0,10} + 1234343549952 a_0^2 a_1 p_{1,9} + 573236269056 a_0^2 a_2 p_{0,9} \\
& + 539291934720 a_0 a_1^2 p_{0,9} - 1082687233536 a_0^2 p_{1,9} - 819526533120 a_0 a_1 p_{0,9} \\
& + 155557324800 a_0 p_{0,9} - 149448499200 p_{13,2}, 56770560000 a_0^4 p_{0,11} \\
& + 410788944000 a_0^3 p_{1,10} + 580270521600 a_0^2 a_1 p_{0,10} - 172858752000 a_0^2 a_2 p_{1,9} \\
& - 102187008000 a_0^2 a_3 p_{0,9} - 161194017600 a_0 a_1^2 p_{1,9} - 183936614400 a_0 a_1 a_2 p_{0,9} \\
& - 28740096000 a_1^3 p_{0,9} - 530525064960 a_0^2 p_{0,10} + 991997340480 a_0 a_1 p_{1,9} \\
& + 502200483840 a_0 a_2 p_{0,9} + 236946124800 a_1^2 p_{0,9} - 450314484480 a_0 p_{1,9} \\
& - 188247628800 a_1 p_{0,9} + 25147584000 p_{0,9} - 57480192000 p_{12,3}, 238351680000 \\
& a_0^3 p_{0,11} - 170648208000 a_0^2 a_1 p_{1,10} - 100590336000 a_0^2 a_2 p_{0,10} - 94303440000 a_0 \\
& a_1^2 p_{0,10} + 600191942400 a_0^2 p_{1,10} + 602608118400 a_0 a_1 p_{0,10} \\
& - 324177500160 a_0 a_2 p_{1,9} - 201616128000 a_0 a_3 p_{0,9} - 151583011200 a_1^2 p_{1,9} \\
& - 182344089600 a_1 a_2 p_{0,9} - 285021504000 a_0 p_{0,10} + 319419331200 a_1 p_{1,9} \\
& + 171403776000 a_2 p_{0,9} - 89646912000 p_{1,9} - 28740096000 p_{11,4}, -71922816000 \\
& a_0^3 p_{1,11} - 121927680000 a_0^2 a_1 p_{0,11} + 443544595200 a_0^2 p_{0,11} \\
& - 390271089600 a_0 a_1 p_{1,10} - 239692400640 a_0 a_2 p_{0,10} + 57480192000 a_0 a_3 p_{1,9} \\
& - 112649745600 a_1^2 p_{0,10} + 51301071360 a_1 a_2 p_{1,9} + 36578304000 a_1 a_3 p_{0,9} \\
& + 17557585920 a_2^2 p_{0,9} + 468224064000 a_0 p_{1,10} + 246389169600 a_1 p_{0,10} \\
& - 182946677760 a_2 p_{1,9} - 117965030400 a_3 p_{0,9} - 72013536000 p_{0,10} \\
& - 18289152000 p_{10,5}, -62589542400 a_0^3 p_{0,12} - 299965317120 a_0^2 p_{1,11} \\
& - 351422668800 a_0 a_1 p_{0,11} + 71612190720 a_0 a_2 p_{1,10} + 51209625600 a_0 a_3 p_{0,10} \\
& + 33408184320 a_1^2 p_{1,10} + 46088663040 a_1 a_2 p_{0,10} + 435920486400 a_0 p_{0,11} \\
& - 268561198080 a_1 p_{1,10} - 170141368320 a_2 p_{0,10} + 76156416000 a_3 p_{1,9} \\
& + 164526888960 p_{1,10} - 14631321600 p_{9,6}, -327924495360 a_0^2 p_{0,12} \\
& + 112996477440 a_0 a_1 p_{1,11} + 78033715200 a_0 a_2 p_{0,11} + 36578304000 a_1^2 p_{0,11} \\
& - 503210050560 a_0 p_{1,11} - 303295104000 a_1 p_{0,11} + 116493189120 a_2 p_{1,10} \\
& + 85044556800 a_3 p_{0,10} - 14631321600 a_5 p_{0,9} + 192036096000 p_{0,11} \\
& - 14631321600 p_{8,7}, 116484480000 a_0^2 p_{1,12} + 150885504000 a_0 a_1 p_{0,12} \\
& - 691199308800 a_0 p_{0,12} + 226306483200 a_1 p_{1,11} + 159376896000 a_2 p_{0,11} \\
& - 28740096000 a_3 p_{1,10} - 341484595200 p_{1,11} - 18289152000 p_{7,8}, 191600640000 \\
& a_0^2 p_{0,13} + 578394432000 a_0 p_{1,12} + 382003776000 a_1 p_{0,12} - 60354201600 a_2 p_{1,11}
\end{aligned}$$

[illegible]

$$\begin{aligned}
& -3410671380480 a_0 a_2 p_{1,10} - 2208872332800 a_0 a_3 p_{0,10} - 1594988236800 a_1^2 p_{1,10} \\
& - 1996391577600 a_1 a_2 p_{0,10} - 4164773760000 a_0 p_{0,11} + 3898456732800 a_1 p_{1,10} \\
& + 2215600128000 a_2 p_{0,10} - 1292342688000 p_{1,10} - 201180672000 p_{11,5}, \\
& -804045312000 a_0^3 p_{1,12} - 1408264704000 a_0^2 a_1 p_{0,12} + 5838263101440 a_0^2 p_{0,12} \\
& - 4460852874240 a_0 a_1 p_{1,11} - 2828722176000 a_0 a_2 p_{0,11} \\
& + 591349248000 a_0 a_3 p_{1,10} - 1329011712000 a_1^2 p_{0,11} + 528190709760 a_1 a_2 p_{1,10} \\
& + 384072192000 a_1 a_3 p_{0,10} + 184354652160 a_2^2 p_{0,10} + 6101568829440 a_0 p_{1,11} \\
& + 3356059392000 a_1 p_{0,11} - 2148725698560 a_2 p_{1,10} - 1432040601600 a_3 p_{0,10} \\
& - 1152216576000 p_{0,11} - 146313216000 p_{10,6}, -780337152000 a_0^3 p_{0,13} \\
& - 3708125568000 a_0^2 p_{1,12} - 4460846100480 a_0 a_1 p_{0,12} + 804722688000 a_0 a_2 p_{1,11} \\
& + 585252864000 a_0 a_3 p_{0,11} + 375567736320 a_1^2 p_{1,11} + 526727577600 a_1 a_2 p_{0,11} \\
& + 6284884193280 a_0 p_{0,12} - 3395899261440 a_1 p_{1,11} - 2209329561600 a_2 p_{0,11} \\
& + 870258816000 a_3 p_{1,10} + 2364970245120 p_{1,11} - 131681894400 p_{9,7}, \\
& -4464991641600 a_0^2 p_{0,13} + 1378087603200 a_0 a_1 p_{1,12} + 965667225600 a_0 a_2 p_{0,12} \\
& + 452656512000 a_1^2 p_{0,12} - 6828037171200 a_0 p_{1,12} - 4208029056000 a_1 p_{0,12} \\
& + 1441185177600 a_2 p_{1,11} + 1066867200000 a_3 p_{0,11} - 164602368000 a_5 p_{0,10} \\
& + 3017710080000 p_{0,12} - 146313216000 p_{8,8}, 1532805120000 a_0^2 p_{1,13} \\
& + 2011806720000 a_0 a_1 p_{0,13} - 10225726156800 a_0 p_{0,13} + 3015794073600 a_1 p_{1,12} \\
& + 2149759180800 a_2 p_{0,12} - 349671168000 a_3 p_{1,11} - 5053945881600 p_{1,12} \\
& - 201180672000 p_{7,9}, 2739889152000 a_0^2 p_{0,14} + 8263735603200 a_0 p_{1,13} \\
& + 5518098432000 a_1 p_{0,13} - 793226649600 a_2 p_{1,12} - 632282112000 a_3 p_{0,12} \\
& - 9484231680000 p_{0,13} - 344881152000 p_{6,10}, 18780694732800 a_0 p_{0,14} \\
& - 2353813862400 a_1 p_{1,13} - 1793381990400 a_2 p_{0,13} + 13811532134400 p_{1,13} \\
& - 747242496000 p_{5,11}, -9589612032000 a_0 p_{1,14} - 6799906713600 a_1 p_{0,14} \\
& + 40799440281600 p_{0,14} - 2092278988800 p_{4,12}, -36614882304000 a_0 p_{0,15} \\
& - 53614649088000 p_{1,14} - 7846046208000 p_{3,13}, -292919058432000 p_{0,15} \\
& - 41845579776000 p_{2,14}] ]
\end{aligned}$$

```

> solve(%[-1], {p0,10, seq(p_{k,m-k} k=2..m)}) :
ss := subs(%[1..1], ss) union {b14=0, op(%)} :

```

```

> m := 17 :
wY := LieDerivative(w, y) : Y := (i, j) → subs(ss, subs({x=0, y=0}, diff(wY, x$i, y$j))) :
Y(0, 0) := subs({x=0, y=0}, wY) :
simplify([seq([seq(Y(k-i, i), i=0..k)], k=0..m)])

```

```

[ [0], [0, 0], [0, 0, 0], [0, 0, 0, 0], [0, 0, 0, 0, 0], [0, 0, 0, 0, 0, 0], [0, 0, 0, 0, 0, 0, 0], [0,
(27)

```

$$\begin{aligned}
& [0, 0, 0, 0, 0, 0, 0], [0, 0, 0, 0, 0, 0, 0, 0, 0, 0], [0, 0, 0, 0, 0, 0, 0, 0, 0, 0, 0], [0, 0, 0, 0, 0, 0, \\
& 0, 0, 0, 0, 0], [0, 0, 0, 0, 0, 0, 0, 0, 0, 0, 0, 0, 0], [0, 0, 0, 0, 0, 0, 0, 0, 0, 0, 0, 0, 0], [0, 0, \\
& 0, 0, 0, 0, 0, 0, 0, 0, 0, 0, 0, 0, 0], [0, 0, 0, 0, 0, 0, 0, 0, 0, 0, 0, 0, 0, 0], [0, 0, 0, 0, 0, 0, \\
& 0, 0, 0, 0, 0, 0, 0, 0, 0, 0, 0, 0], [0, 0, 0, 0, 0, 0, 0, 0, 0, 0, 0, 0, 0, 0], [0, 0, 0, 0, 0, 0, 0, 0, 0, 0, 0, 0], [ \\
& -94043670336000 a_0^6 p_{1,10}, 473272920288000 a_0^5 p_{1,10}, 80269862400000 a_0^5 p_{0,11} \\
& - 263503110528000 a_0^4 a_1 p_{1,10} + 664469371987200 a_0^4 p_{1,10} \\
& - 711374856192000 p_{17,0}, -36701767872000 a_0^5 p_{1,11} - 61993451520000 a_0^4 a_1 p_{0,11} \\
& + 162178684012800 a_0^4 p_{0,11} - 567913782643200 a_0^3 a_1 p_{1,10} + 502405184206080 \\
& a_0^3 p_{1,10} - 125536739328000 p_{16,1}, -11187880704000 a_0^5 p_{0,12} - 115299497779200 \\
& a_0^4 p_{1,11} - 182738687040000 a_0^3 a_1 p_{0,11} + 61157646950400 a_0^3 a_2 p_{1,10} \\
& + 85593585168000 a_0^2 a_1^2 p_{1,10} + 167896444584960 a_0^3 p_{0,11} - 534544826618880 \\
& a_0^2 a_1 p_{1,10} + 246070799009280 a_0^2 p_{1,10} - 31384184832000 p_{15,2}, -46347715814400 \\
& a_0^4 p_{0,12} + 48118076697600 a_0^3 a_1 p_{1,11} + 24797380608000 a_0^3 a_2 p_{0,11} \\
& + 34871316480000 a_0^2 a_1^2 p_{0,11} - 171829468661760 a_0^3 p_{1,11} - 225489905222400 \\
& a_0^2 a_1 p_{0,11} + 131733872017920 a_0^2 a_2 p_{1,10} + 123238588536000 a_0 a_1^2 p_{1,10} \\
& + 107827456089600 a_0^2 p_{0,11} - 264272793350400 a_0 a_1 p_{1,10} \\
& + 75480476486400 a_0 p_{1,10} - 10461394944000 p_{14,3}, 11860611840000 a_0^4 p_{1,12} \\
& + 23974030080000 a_0^3 a_1 p_{0,12} - 88355198131200 a_0^3 p_{0,12} + 124231878489600 \\
& a_0^2 a_1 p_{1,11} + 68070917376000 a_0^2 a_2 p_{0,11} - 17281693440000 a_0^2 a_3 p_{1,10} \\
& + 63978647040000 a_0 a_1^2 p_{0,11} - 30863749593600 a_0 a_1 a_2 p_{1,10} - 4799596032000 \\
& a_1^3 p_{1,10} - 151600721402880 a_0^2 p_{1,11} - 142048867968000 a_0 a_1 p_{0,11} \\
& + 112195142184960 a_0 a_2 p_{1,10} + 52609631155200 a_1^2 p_{1,10} \\
& + 42138144000000 a_0 p_{0,11} - 57900994387200 a_1 p_{1,10} + 11351389248000 p_{1,10} \\
& - 4483454976000 p_{13,4}, 7153090560000 a_0^4 p_{0,13} + 48723528672000 a_0^3 p_{1,12} \\
& + 77626679961600 a_0^2 a_1 p_{0,12} - 16566749337600 a_0^2 a_2 p_{1,11} - 10729635840000 \\
& a_0^2 a_3 p_{0,11} - 15461992022400 a_0 a_1^2 p_{1,11} - 19313344512000 a_0 a_1 a_2 p_{0,11} \\
& - 3017710080000 a_1^3 p_{0,11} - 97749497260800 a_0^2 p_{0,12} \\
& + 126536222131200 a_0 a_1 p_{1,11} + 72520842240000 a_0 a_2 p_{0,11} \\
& - 33927012000000 a_0 a_3 p_{1,10} + 34158801600000 a_1^2 p_{0,11} \\
& - 30420607795200 a_1 a_2 p_{1,10} - 78957019814400 a_0 p_{1,11} \\
& - 38915886240000 a_1 p_{0,11} + 37668889036800 a_2 p_{1,10} + 7921488960000 p_{0,11} \\
& - 2414168064000 p_{12,5}, 36457189171200 a_0^3 p_{0,13} - 19583719142400 a_0^2 a_1 p_{1,12}
\end{aligned}$$

$$\begin{aligned}
& -12392729395200 a_0^2 a_2 p_{0,12} - 11618183808000 a_0 a_1^2 p_{0,12} + 88687842969600 \\
& a_0^2 p_{1,12} + 97902338688000 a_0 a_1 p_{0,12} - 39016695029760 a_0 a_2 p_{1,11} \\
& - 26049848832000 a_0 a_3 p_{0,11} - 18248306227200 a_1^2 p_{1,11} \\
& - 23532042240000 a_1 a_2 p_{0,11} + 4799073484800 a_1 a_3 p_{1,10} + 2297117491200 \\
& a_2^2 p_{1,10} - 63023198515200 a_0 p_{0,12} + 50735123712000 a_1 p_{1,11} \\
& + 30091751424000 a_2 p_{0,11} - 19699042406400 a_3 p_{1,10} - 19387720396800 p_{1,11} \\
& - 1609445376000 p_{11,6}, -9769890816000 a_0^3 p_{1,13} - 17557585920000 a_0^2 a_1 p_{0,13} \\
& + 81675067944960 a_0^2 p_{0,13} - 55189767467520 a_0 a_1 p_{1,12} \\
& - 35881435054080 a_0 a_2 p_{0,12} + 6652025856000 a_0 a_3 p_{1,11} - 16853910796800 \\
& a_1^2 p_{0,12} + 5945437532160 a_1 a_2 p_{1,11} + 4389396480000 a_1 a_3 p_{0,11} + 2106910310400 \\
& a_2^2 p_{0,11} + 84747149061120 a_0 p_{1,12} + 48238095628800 a_1 p_{0,12} \\
& - 27168169512960 a_2 p_{1,11} - 18572633856000 a_3 p_{0,11} - 19011573504000 p_{0,12} \\
& - 1316818944000 p_{10,7}, -10461394944000 a_0^3 p_{0,14} - 49387155148800 a_0^2 p_{1,13} \\
& - 60690721996800 a_0 a_1 p_{0,13} + 9824932454400 a_0 a_2 p_{1,12} \\
& + 7242504192000 a_0 a_3 p_{0,12} + 4586919321600 a_1^2 p_{1,12} + 6518253772800 a_1 a_2 p_{0,12} \\
& + 95707654963200 a_0 p_{0,13} - 46073857536000 a_1 p_{1,12} - 30613950259200 a_2 p_{0,12} \\
& + 10770568704000 a_3 p_{1,11} - 1536288768000 a_5 p_{1,10} + 35943147878400 p_{1,12} \\
& - 1316818944000 p_{9,8}, -64947826944000 a_0^2 p_{0,14} + 18156555648000 a_0 a_1 p_{1,13} \\
& + 12875563008000 a_0 a_2 p_{0,13} + 6035420160000 a_1^2 p_{0,13} - 99059446886400 a_0 p_{1,13} \\
& - 62164827648000 a_1 p_{0,13} + 19213712179200 a_2 p_{1,12} + 14384418048000 a_3 p_{0,12} \\
& - 2011806720000 a_5 p_{0,11} + 49792216320000 p_{0,13} - 1609445376000 p_{8,9}, \\
& 21679612416000 a_0^2 p_{1,14} + 28768836096000 a_0 a_1 p_{0,14} - 160657136640000 a_0 p_{0,14} \\
& + 43110144000000 a_1 p_{1,13} + 31039303680000 a_2 p_{0,13} - 4598415360000 a_3 p_{1,12} \\
& - 79437625344000 p_{1,13} - 2414168064000 p_{7,10}, 41845579776000 a_0^2 p_{0,15} \\
& + 126122079283200 a_0 p_{1,14} + 84998833920000 a_1 p_{0,14} - 11208637440000 a_2 p_{1,13} \\
& - 8966909952000 a_3 p_{0,13} - 160283515392000 p_{0,14} - 4483454976000 p_{6,11}, \\
& 307565011353600 a_0 p_{0,15} - 35568742809600 a_1 p_{1,14} - 27199626854400 a_2 p_{0,14} \\
& + 226489200537600 p_{1,14} - 10461394944000 p_{5,12}, -154305575424000 a_0 p_{1,15} \\
& - 109844646912000 a_1 p_{0,15} + 713990204928000 p_{0,15} - 31384184832000 p_{4,13}, \\
& -627683696640000 a_0 p_{0,16} - 920602755072000 p_{1,15} - 125536739328000 p_{3,14}, \\
& -5335311421440000 p_{0,16} - 711374856192000 p_{2,15}]
\end{aligned}$$

> solve(%[-1], {p<sub>1,10</sub>, seq(p<sub>k,m-k</sub> k=2..m)}) :



$$\begin{aligned}
& - 3210199895577600 a_0 a_1 p_{1,11} - 1625753825280000 a_0 a_2 p_{0,11} \\
& - 767947340160000 a_1^2 p_{0,11} + 1082545934284800 a_0 p_{1,11} \\
& + 465625480320000 a_1 p_{0,11} - 58845346560000 p_{0,11} - 62768369664000 p_{14,4}, \\
& 131442829056000 a_0^4 p_{1,13} + 278970531840000 a_0^3 a_1 p_{0,13} - 1171854666178560 \\
& a_0^3 p_{0,13} + 1412199155646720 a_0^2 a_1 p_{1,12} + 812286506465280 a_0^2 a_2 p_{0,12} \\
& - 177700013568000 a_0^2 a_3 p_{1,11} + 763222468377600 a_0 a_1^2 p_{0,12} \\
& - 317569726172160 a_0 a_1 a_2 p_{1,11} - 209227898880000 a_0 a_1 a_3 p_{0,11} \\
& - 100429391462400 a_0 a_2^2 p_{0,11} - 49403686147200 a_1^3 p_{1,11} - 94152554496000 \\
& a_1^2 a_2 p_{0,11} - 1962931364997120 a_0^2 p_{1,12} - 1956223853337600 a_0 a_1 p_{0,12} \\
& + 1315101070080000 a_0 a_2 p_{1,11} + 793527114240000 a_0 a_3 p_{0,11} \\
& + 616528571299200 a_1^2 p_{1,11} + 719778721536000 a_1 a_2 p_{0,11} \\
& + 681801297408000 a_0 p_{0,12} - 783038231136000 a_1 p_{1,11} \\
& - 415803870720000 a_2 p_{0,11} + 180262454400000 p_{1,11} - 31384184832000 p_{13,5}, \\
& 89503045632000 a_0^4 p_{0,14} + 598844490854400 a_0^3 p_{1,13} + 991802830233600 a_0^2 a_1 p_{0,13} \\
& - 185855175475200 a_0^2 a_2 p_{1,12} - 123927293952000 a_0^2 a_3 p_{0,12} \\
& - 173521682611200 a_0 a_1^2 p_{1,12} - 223069129113600 a_0 a_1 a_2 p_{0,12} \\
& - 34854551424000 a_1^3 p_{0,12} - 1417782657392640 a_0^2 p_{0,13} \\
& + 1595234405882880 a_0 a_1 p_{1,12} + 950828650168320 a_0 a_2 p_{0,12} \\
& - 388377071308800 a_0 a_3 p_{1,11} + 447613583155200 a_1^2 p_{0,12} \\
& - 348311778877440 a_1 a_2 p_{1,11} - 236387289600000 a_1 a_3 p_{0,11} - 113626843545600 \\
& a_2^2 p_{0,11} - 1130076111790080 a_0 p_{1,12} - 586109710771200 a_1 p_{0,12} \\
& + 489816167178240 a_2 p_{1,11} + 305191079424000 a_3 p_{0,11} + 139418205696000 p_{0,12} \\
& - 19313344512000 p_{12,6}, 498342813696000 a_0^3 p_{0,14} - 238336390656000 a_0^2 a_1 p_{1,13} \\
& - 154506756096000 a_0^2 a_2 p_{0,13} - 144850083840000 a_0 a_1^2 p_{0,13} \\
& + 1199450993448960 a_0^2 p_{1,13} + 1367188313702400 a_0 a_1 p_{0,13} \\
& - 483028209377280 a_0 a_2 p_{1,12} - 330258191155200 a_0 a_3 p_{0,12} \\
& + 48283361280000 a_0 a_5 p_{0,11} - 225942616166400 a_1^2 p_{1,12} \\
& - 298218732134400 a_1 a_2 p_{0,12} + 54072661708800 a_1 a_3 p_{1,11} + 25888660439040 \\
& a_2^2 p_{1,11} + 38626689024000 a_2 a_3 p_{0,11} - 995866273382400 a_0 p_{0,13} \\
& + 703978287667200 a_1 p_{1,12} + 431572777574400 a_2 p_{0,12} \\
& - 249065939404800 a_3 p_{1,11} - 304562847052800 p_{1,12} - 14485008384000 p_{11,7}, \\
& - 128276628480000 a_0^3 p_{1,14} - 235381386240000 a_0^2 a_1 p_{0,14} + 1213793538048000
\end{aligned}$$

$$\begin{aligned}
& a_0^2 p_{0,14} - 735549979852800 a_0 a_1 p_{1,13} - 487900230451200 a_0 a_2 p_{0,13} \\
& + 81282216960000 a_0 a_3 p_{1,12} - 229126496256000 a_1^2 p_{0,13} \\
& + 72688405708800 a_1 a_2 p_{1,12} + 54318781440000 a_1 a_3 p_{0,12} + 26073015091200 \\
& a_2^2 p_{0,12} + 1252714943692800 a_0 p_{1,13} + 732809742336000 a_1 p_{0,13} \\
& - 368585983180800 a_2 p_{1,12} - 257108898816000 a_3 p_{0,12} + 72425041920000 a_5 p_{0,11} \\
& - 325912688640000 p_{0,13} - 13168189440000 p_{10,8} - 150214901760000 a_0^3 p_{0,15} \\
& - 705474514483200 a_0^2 p_{1,14} - 882244306944000 a_0 a_1 p_{0,14} \\
& + 129560352768000 a_0 a_2 p_{1,13} + 96566722560000 a_0 a_3 p_{0,13} + 60505087104000 \\
& a_1^2 p_{1,13} + 86910050304000 a_1 a_2 p_{0,13} + 1539319541760000 a_0 p_{0,14} \\
& - 668382067584000 a_1 p_{1,13} - 451794309120000 a_2 p_{0,13} \\
& + 143638209792000 a_3 p_{1,12} - 18709802496000 a_5 p_{1,11} - 16094453760000 a_6 p_{0,11} \\
& + 577316678400000 p_{1,13} - 14485008384000 p_{9,9} - 1006064304537600 a_0^2 p_{0,15} \\
& + 257068662681600 a_0 a_1 p_{1,14} + 184120551014400 a_0 a_2 p_{0,14} + 86306508288000 \\
& a_1^2 p_{0,14} - 1531302970982400 a_0 p_{1,14} - 975525078528000 a_1 p_{0,14} \\
& + 274755317760000 a_2 p_{1,13} + 207618453504000 a_3 p_{0,13} - 26555848704000 a_5 p_{0,12} \\
& + 863065082880000 p_{0,14} - 19313344512000 p_{8,10} - 328039455744000 a_0^2 p_{1,15} \\
& + 439378587648000 a_0 a_1 p_{0,15} - 2673932547686400 a_0 p_{0,15} \\
& + 658245914726400 a_1 p_{1,14} + 477936300441600 a_2 p_{0,14} - 65010097152000 a_3 p_{1,13} \\
& - 1322731304294400 p_{1,14} - 31384184832000 p_{7,11} - 679990671360000 a_0^2 p_{0,16} \\
& + 2048341130035200 a_0 p_{1,15} + 1391365527552000 a_1 p_{0,15} \\
& - 169474598092800 a_2 p_{1,14} - 135998134272000 a_3 p_{0,14} - 2855960819712000 p_{0,15} \\
& - 62768369664000 p_{6,12} - 5335311421440000 a_0 p_{0,16} - 572761373184000 a_1 p_{1,15} \\
& - 439378587648000 a_2 p_{0,15} + 3933484498944000 p_{1,15} - 156920924160000 p_{5,13} \\
& - 2636271525888000 a_0 p_{1,16} - 1883051089920000 a_1 p_{0,16} \\
& + 13181357629440000 p_{0,16} - 502146957312000 p_{4,14} \\
& - 11381997699072000 a_0 p_{0,17} - 16717309120512000 p_{1,16} \\
& - 2134124568576000 p_{3,15} - 102437979291648000 p_{0,17} \\
& - 12804747411456000 p_{2,16} ] ]
\end{aligned}$$

```

> solve( %[ -1 ], { p0,11, p1,11, seq( pk,m-k k=2..m ) } ) :
ss := subs( %[ 1..2 ], ss ) union { a16 = 0, b16 = 0, op( % ) } :
>
> m := 19 :
wY := LieDerivative( w, y ) : Y := ( i, j ) → subs( ss, subs( { x = 0, y = 0 }, diff( wY, x$ i, y$ j ) ) ) :
Y( 0, 0 ) := subs( { x = 0, y = 0 }, wY ) :
simplify( [ seq( [ seq( Y( k - i, i ), i = 0..k ), k = 0..m ) ] )

```



$$\begin{aligned}
& [ [0], [0, 0], [0, 0, 0], [0, 0, 0, 0], [0, 0, 0, 0, 0], [0, 0, 0, 0, 0, 0], [0, 0, 0, 0, 0, 0, 0], [0, \\
& 0, 0, 0, 0, 0, 0, 0], [0, 0, 0, 0, 0, 0, 0, 0], [0, 0, 0, 0, 0, 0, 0, 0, 0], [0, 0, 0, 0, 0, 0, \\
& 0, 0, 0, 0, 0], [0, 0, 0, 0, 0, 0, 0, 0, 0, 0], [0, 0, 0, 0, 0, 0, 0, 0, 0, 0], [0, 0, \\
& 0, 0, 0, 0, 0, 0, 0, 0, 0, 0, 0], [0, 0, 0, 0, 0, 0, 0, 0, 0, 0, 0, 0], [0, 0, 0, 0, 0, 0, \\
& 0, 0, 0, 0, 0, 0, 0, 0, 0, 0, 0], [0, 0, 0, 0, 0, 0, 0, 0, 0, 0, 0, 0, 0], [0, 0, 0, 0, 0, 0, \\
& 0, 0, 0, 0, 0, 0, 0, 0, 0, 0, 0, 0], [0, 0, 0, 0, 0, 0, 0, 0, 0, 0, 0, 0, 0, 0], [0, 0, 0, 0, 0, 0, \\
& 0, 0, 0, 0, 0, 0, 0, 0, 0, 0, 0, 0, 0], [0, 0, 0, 0, 0, 0, 0, 0, 0, 0, 0, 0, 0, 0, 0], \\
& [48182472898560000 a_0^7 p_{0, 12}, 2409123644928000 a_0^6 p_{0, 12}, 16433559305856000 \\
& a_0^6 p_{1, 12} + 21682112804352000 a_0^5 a_1 p_{0, 12} - 54405409118860800 a_0^5 p_{0, 12} \\
& - 243290200817664000 p_{19, 0}, 3372443762688000 a_0^6 p_{0, 13} + 50819711802048000 \\
& a_0^5 p_{1, 12} + 79053483411302400 a_0^4 a_1 p_{0, 12} - 71976027552549120 a_0^4 p_{0, 12} \\
& - 38414242234368000 p_{18, 1}, 14255927562240000 a_0^5 p_{0, 13} - 20927526778368000 \\
& a_0^4 a_1 p_{1, 12} - 9129310654464000 a_0^4 a_2 p_{0, 12} - 17117457477120000 a_0^3 a_1^2 p_{0, 12} \\
& + 75523187929651200 a_0^4 p_{1, 12} + 111202721402572800 a_0^3 a_1 p_{0, 12} \\
& - 53297084311511040 a_0^3 p_{0, 12} - 8536498274304000 p_{17, 2}, -3356068826880000 \\
& a_0^5 p_{1, 13} - 7439214182400000 a_0^4 a_1 p_{0, 13} + 27644096880691200 a_0^4 p_{0, 13} \\
& - 56608254699494400 a_0^3 a_1 p_{1, 12} - 27153477924249600 a_0^3 a_2 p_{0, 12} \\
& - 38279318460768000 a_0^2 a_1^2 p_{0, 12} + 69985588419072000 a_0^3 p_{1, 12} \\
& + 85800349093536000 a_0^2 a_1 p_{0, 12} - 25665742783296000 a_0^2 p_{0, 12} \\
& - 2510734786560000 p_{16, 3}, -1454424491520000 a_0^5 p_{0, 14} - 13382418478464000 \\
& a_0^4 p_{1, 13} - 25457712134400000 a_0^3 a_1 p_{0, 13} + 5786313781248000 a_0^3 a_2 p_{1, 12} \\
& + 3356364211200000 a_0^3 a_3 p_{0, 12} + 8103147867360000 a_0^2 a_1^2 p_{1, 12} \\
& + 9062183370240000 a_0^2 a_1 a_2 p_{0, 12} + 2831932303200000 a_0 a_1^3 p_{0, 12} \\
& + 32413805512058880 a_0^3 p_{0, 13} - 67297620162044160 a_0^2 a_1 p_{1, 12} \\
& - 34472331969546240 a_0^2 a_2 p_{0, 12} - 32470456517452800 a_0 a_1^2 p_{0, 12} \\
& + 42621790305576960 a_0^2 p_{1, 12} + 37463597337196800 a_0 a_1 p_{0, 12} \\
& - 7719956221824000 a_0 p_{0, 12} - 941525544960000 p_{15, 4}, -7205668823808000 \\
& a_0^4 p_{0, 14} + 5430454638336000 a_0^3 a_1 p_{1, 13} + 3124469956608000 a_0^3 a_2 p_{0, 13} \\
& + 4393785876480000 a_0^2 a_1^2 p_{0, 13} - 24945751901790720 a_0^3 p_{1, 13} \\
& - 37511380789908480 a_0^2 a_1 p_{0, 13} + 15709238202792960 a_0^2 a_2 p_{1, 12} \\
& + 9520654003660800 a_0^2 a_3 p_{0, 12} + 14697621886872960 a_0 a_1^2 p_{1, 12} \\
& + 17199335328215040 a_0 a_1 a_2 p_{0, 12} + 2693302474262400 a_1^3 p_{0, 12} \\
& + 24465745645286400 a_0^2 p_{0, 13} - 41519180188402560 a_0 a_1 p_{1, 12}
\end{aligned}$$

$$\begin{aligned}
& - 22323313287475200 a_0 a_2 p_{0,12} - 10534908038054400 a_1^2 p_{0,12} \\
& + 16126414728076800 a_0 p_{1,12} + 7480796411088000 a_1 p_{0,12} \\
& - 1132772921280000 p_{0,12} - 439378587648000 p_{14,5} + 1584022099968000 a_0^4 p_{1,14} \\
& + 3490618779648000 a_0^3 a_1 p_{0,14} - 16448356166860800 a_0^3 p_{0,14} \\
& + 17373312761978880 a_0^2 a_1 p_{1,13} + 10370815358238720 a_0^2 a_2 p_{0,13} \\
& - 1995980507136000 a_0^2 a_3 p_{1,12} + 9742080157286400 a_0 a_1^2 p_{0,13} \\
& - 3569087288954880 a_0 a_1 a_2 p_{1,12} - 2416582232064000 a_0 a_1 a_3 p_{0,12} \\
& - 1159959471390720 a_0 a_2^2 p_{0,12} - 555419599257600 a_1^3 p_{1,12} - 1087462004428800 \\
& a_1^2 a_2 p_{0,12} - 27084646125895680 a_0^2 p_{1,13} - 28287005773824000 a_0 a_1 p_{0,13} \\
& + 16580961204756480 a_0 a_2 p_{1,12} + 10391062181068800 a_0 a_3 p_{0,12} \\
& + 7772154434150400 a_1^2 p_{1,12} + 9417000931430400 a_1 a_2 p_{0,12} \\
& + 11312967123763200 a_0 p_{0,13} - 11183433769267200 a_1 p_{1,12} \\
& - 6240946334515200 a_2 p_{0,12} + 2954341826150400 p_{1,12} - 251073478656000 p_{13,6}, \\
& 1201719214080000 a_0^4 p_{0,15} + 7932029346662400 a_0^3 p_{1,14} + 13546634669568000 \\
& a_0^2 a_1 p_{0,14} - 2264604604416000 a_0^2 a_2 p_{1,13} - 1545067560960000 a_0^2 a_3 p_{0,13} \\
& - 2114962109568000 a_0 a_1^2 p_{1,13} - 2781121609728000 a_0 a_1 a_2 p_{0,13} \\
& - 434550251520000 a_1^3 p_{0,13} - 21660766577049600 a_0^2 p_{0,14} \\
& + 21574456785423360 a_0 a_1 p_{1,13} + 13261204513751040 a_0 a_2 p_{0,13} \\
& - 4810657920768000 a_0 a_3 p_{1,12} + 6240141611827200 a_1^2 p_{0,13} \\
& - 4315268352245760 a_1 a_2 p_{1,12} - 2994171941376000 a_1 a_3 p_{0,12} \\
& - 1439023504343040 a_2^2 p_{0,12} - 17099890642114560 a_0 p_{1,13} \\
& - 9227674591027200 a_1 p_{0,13} + 6792058472693760 a_2 p_{1,12} \\
& + 4369764904243200 a_3 p_{0,12} + 2509527702528000 p_{0,13} - 173820100608000 p_{12,7}, \\
& 7266048427008000 a_0^3 p_{0,15} - 3133351081728000 a_0^2 a_1 p_{1,14} - 2071356198912000 \\
& a_0^2 a_2 p_{0,14} - 1941896436480000 a_0 a_1^2 p_{0,14} + 17345590088601600 a_0^2 p_{1,14} \\
& + 20289303740160000 a_0 a_1 p_{0,14} - 6440992033996800 a_0 a_2 p_{1,13} \\
& - 4488816310272000 a_0 a_3 p_{0,13} + 597506595840000 a_0 a_5 p_{0,12} \\
& - 3013207029504000 a_1^2 p_{1,13} - 4052040007680000 a_1 a_2 p_{0,13} \\
& + 661607460864000 a_1 a_3 p_{1,12} + 316826637926400 a_2^2 p_{1,12} \\
& + 478005276672000 a_2 a_3 p_{0,12} - 16491132403200000 a_0 p_{0,14} \\
& + 10397952923904000 a_1 p_{1,13} + 6544903680000000 a_2 p_{0,13} \\
& - 3378977441280000 a_3 p_{1,12} - 5022501603840000 p_{1,13} - 144850083840000 p_{11,8},
\end{aligned}$$

$$\begin{aligned}
& -1810434447360000 a_0^3 p_{1,15} - 3379835289600000 a_0^2 a_1 p_{0,15} + 19132161198796800 \\
& a_0^2 p_{0,15} - 10512982937318400 a_0 a_1 p_{1,14} - 7089239008051200 a_0 a_2 p_{0,14} \\
& + 1072580382720000 a_0 a_3 p_{1,13} - 3328685103744000 a_1^2 p_{0,14} \\
& + 959631805440000 a_1 a_2 p_{1,13} + 724250419200000 a_1 a_3 p_{0,13} + 347640201216000 \\
& a_2^2 p_{0,13} + 19664358800486400 a_0 p_{1,14} + 11763184777344000 a_1 p_{0,14} \\
& - 5346807459840000 a_2 p_{1,13} - 3791450944512000 a_3 p_{0,13} \\
& + 975927439872000 a_5 p_{0,12} - 5825689309440000 p_{0,14} - 144850083840000 p_{10,9}, \\
& -2301506887680000 a_0^3 p_{0,16} - 10763464848998400 a_0^2 p_{1,15} \\
& - 13659041017036800 a_0 a_1 p_{0,15} + 1835733395865600 a_0 a_2 p_{1,14} \\
& + 1380904132608000 a_0 a_3 p_{0,14} + 857512496332800 a_1^2 p_{1,14} \\
& + 1242813719347200 a_1 a_2 p_{0,14} + 26121298452480000 a_0 p_{0,15} \\
& - 10331685142732800 a_1 p_{1,14} - 7083858862080000 a_2 p_{0,14} \\
& + 2054571982848000 a_3 p_{1,13} - 246245142528000 a_5 p_{1,12} \\
& - 212446789632000 a_6 p_{0,12} + 9787554653184000 p_{1,14} - 173820100608000 p_{9,10}, \\
& -16544696103936000 a_0^2 p_{0,16} + 3893208128409600 a_0 a_1 p_{1,15} \\
& + 2812022960947200 a_0 a_2 p_{0,15} + 1318135762944000 a_1^2 p_{0,15} \\
& - 25140674880921600 a_0 p_{1,15} - 16220392860672000 a_1 p_{0,15} \\
& + 4196513857536000 a_2 p_{1,14} + 3195956155392000 a_3 p_{0,14} \\
& - 376610217984000 a_5 p_{0,13} + 15707784508416000 p_{0,15} - 251073478656000 p_{8,11}, \\
& 5288235144192000 a_0^2 p_{1,16} + 7139902049280000 a_0 a_1 p_{0,16} \\
& - 47029200970752000 a_0 p_{0,16} + 10694684051251200 a_1 p_{1,15} \\
& + 7820938860134400 a_2 p_{0,15} - 983371124736000 a_3 p_{1,14} \\
& - 23274511471411200 p_{1,15} - 439378587648000 p_{7,12}, 11716762337280000 a_0^2 p_{0,17} \\
& + 35278439099904000 a_0 p_{1,16} + 24126592089600000 a_1 p_{0,16} \\
& - 2730424080384000 a_2 p_{1,15} - 2196892938240000 a_3 p_{0,15} \\
& - 53549265369600000 p_{0,16} - 941525544960000 p_{6,13}, 97751274356736000 a_0 p_{0,17} \\
& - 9791865667584000 a_1 p_{1,16} - 7532204359680000 a_2 p_{0,16} \\
& + 72141779533824000 p_{1,16} - 2510734786560000 p_{5,14}, \\
& -47662115364864000 a_0 p_{1,17} - 34145993097216000 a_1 p_{0,17} \\
& + 256094948229120000 p_{0,17} - 8536498274304000 p_{4,15}, \\
& -217680705994752000 a_0 p_{0,18} - 320118685286400000 p_{1,17} \\
& - 38414242234368000 p_{3,16}, -2067966706950144000 p_{0,18}
\end{aligned}$$

$$-243290200817664000 p_{2,17}]]$$

```

> solve(%[-1], {p0, 12, seq(pk, m-k k=2..m)}) :
ss := subs(%[1..1], ss) union {b17=0, op(%) } :

```

>

**>**  $m := 20 :$

$$wY := LieDerivative(w, y) : Y := (i, j) \rightarrow subs(ss, subs(\{x=0, y=0\}, diff(wY, x\$i, y\$j))) :$$
$$Y(0, 0) := \text{subs}(\{x=0, y=0\}, wY) :$$
$$\text{simplify}([seq([seq(Y(k-i, i), i=0..k)], k=0..m)])$$
$$[0], [0, 0], [0, 0, 0], [0, 0, 0, 0], [0, 0, 0, 0, 0], [0, 0, 0, 0, 0, 0], [0, 0, 0, 0, 0, 0, 0], [0, \quad (30)$$

$[0, 0, 0, 0, 0, 0, 0, 0], [0, 0, 0, 0, 0, 0, 0, 0, 0, 0], [0, 0, 0, 0, 0, 0, 0, 0, 0, 0, 0], [0, 0, 0, 0, 0, 0, 0, 0, 0, 0, 0, 0],$   
 $[0, 0, 0, 0, 0, 0], [0, 0, 0, 0, 0, 0, 0, 0, 0, 0, 0, 0, 0, 0], [0, 0, 0, 0, 0, 0, 0, 0, 0, 0, 0, 0, 0, 0, 0, 0], [0, 0,$   
 $0, 0, 0, 0, 0, 0, 0, 0, 0, 0, 0, 0], [0, 0, 0, 0, 0, 0, 0, 0, 0, 0, 0, 0, 0, 0, 0, 0], [0, 0, 0, 0, 0, 0, 0, 0,$   
 $0, 0, 0, 0, 0, 0, 0, 0, 0, 0], [0, 0, 0, 0, 0, 0, 0, 0, 0, 0, 0, 0, 0, 0, 0, 0], [0, 0, 0, 0, 0, 0, 0, 0, 0, 0, 0,$   
 $0, 0, 0, 0, 0, 0, 0, 0, 0, 0, 0, 0, 0, 0, 0, 0], [0, 0, 0, 0, 0, 0, 0, 0, 0, 0, 0, 0, 0, 0, 0, 0], [0, 0,$   
 $0, 0, 0, 0, 0, 0, 0, 0, 0, 0, 0, 0, 0, 0, 0, 0], [0, 0, 0, 0, 0, 0, 0, 0, 0, 0, 0, 0, 0, 0, 0, 0], [0, 0,$

$$\begin{aligned}
& 0, 0, 0, 0, 0, 0, 0, 0, 0, 0, 0, 0, 0, 0, 0, 0, 0, 0], [460813984646400000 \, a_0^7 p_{1, 12}, \\
& -2808947092492800000 \, a_0^6 p_{1, 12}, -406293935523840000 \, a_0^6 p_{0, 13} \\
& + 1431962997171840000 \, a_0^5 a_1 p_{1, 12} - 4392286538963328000 \, a_0^5 p_{1, 12} \\
& - 4865804016353280000 \, p_{20, 0}, 152146138814208000 \, a_0^6 p_{1, 13} \\
& + 288343941709824000 \, a_0^5 a_1 p_{0, 13} - 910061038579230720 \, a_0^5 p_{0, 13} \\
& + 3565158529006448640 \, a_0^4 a_1 p_{1, 12} - 3807011602678464000 \, a_0^4 p_{1, 12} \\
& - 729870602452992000 \, p_{19, 1}, 39560346169344000 \, a_0^6 p_{0, 14} + 520914705125068800 \\
& a_0^5 p_{1, 13} + 971897420003328000 \, a_0^4 a_1 p_{0, 13} - 295956868696473600 \, a_0^4 a_2 p_{1, 12} \\
& - 552689086779648000 \, a_0^3 a_1^2 p_{1, 12} - 1069635368716701696 \, a_0^4 p_{0, 13} \\
& + 4066255536036175872 \, a_0^3 a_1 p_{1, 12} - 2247443049601032192 \, a_0^3 p_{1, 12} \\
& - 153656968937472000 \, p_{18, 2}, 176336397619200000 \, a_0^5 p_{0, 14} \\
& - 209819117491200000 \, a_0^4 a_1 p_{1, 13} - 101173312880640000 \, a_0^4 a_2 p_{0, 13} \\
& - 189699961651200000 \, a_0^3 a_1^2 p_{0, 13} + 866798336052864000 \, a_0^4 p_{1, 13} \\
& + 1436058179735961600 \, a_0^3 a_1 p_{0, 13} - 762925498721280000 \, a_0^3 a_2 p_{1, 12} \\
& - 1070929561436179200 \, a_0^2 a_1^2 p_{1, 12} - 818527487417303040 \, a_0^3 p_{0, 13} \\
& + 2696704507871412480 \, a_0^2 a_1 p_{1, 12} - 920993645553799680 \, a_0^2 p_{1, 12} \\
& - 42682491371520000 \, p_{17, 3}, -36643680944640000 \, a_0^5 p_{1, 14} - 87265469491200000 \\
& a_0^4 a_1 p_{0, 14} + 370169553761280000 \, a_0^4 p_{0, 14} - 636098325657984000 \, a_0^3 a_1 p_{1, 13} \\
& - 327871237349376000 \, a_0^3 a_2 p_{0, 13} + 76313417241600000 \, a_0^3 a_3 p_{1, 12} \\
& - 462076964616960000 \, a_0^2 a_1^2 p_{0, 13} + 204655251193344000 \, a_0^2 a_1 a_2 p_{1, 12}
\end{aligned}$$

$$\begin{aligned}
& + 63694492313760000 a_0 a_1^3 p_{1,12} + 895828792431974400 a_0^3 p_{1,13} \\
& + 1197492002055014400 a_0^2 a_1 p_{0,13} - 860070192593817600 a_0^2 a_2 p_{1,12} \\
& - 806555473101100800 a_0 a_1^2 p_{1,12} - 421824524815872000 a_0^2 p_{0,13} \\
& + 1039607788293388800 a_0 a_1 p_{1,12} - 242906888185344000 a_0 p_{1,12} \\
& - 15064408719360000 p_{16,4} - 18226074746880000 a_0^5 p_{0,15} - 162560129824512000 \\
& a_0^4 p_{1,14} - 326698598903040000 a_0^3 a_1 p_{0,14} + 64377680919552000 a_0^3 a_2 p_{1,13} \\
& + 39055874457600000 a_0^3 a_3 p_{0,13} + 90180196404480000 a_0^2 a_1^2 p_{1,13} \\
& + 105450861035520000 a_0^2 a_1 a_2 p_{0,13} + 32953394073600000 a_0 a_1^3 p_{0,13} \\
& + 472444742878617600 a_0^3 p_{0,14} - 840846011749632000 a_0^2 a_1 p_{1,13} \\
& - 455386388868956160 a_0^2 a_2 p_{0,13} + 195317373589632000 a_0^2 a_3 p_{1,12} \\
& - 428713622249472000 a_0 a_1^2 p_{0,13} + 350430077720862720 a_0 a_1 a_2 p_{1,12} \\
& + 54646651067904000 a_1^3 p_{1,12} + 604271894339635200 a_0^2 p_{1,13} \\
& + 568712026907136000 a_0 a_1 p_{0,13} - 500684241006673920 a_0 a_2 p_{1,12} \\
& - 235228817117952000 a_1^2 p_{1,12} - 137049632487936000 a_0 p_{0,13} \\
& + 185819506548480000 a_1 p_{1,12} - 31740910169472000 p_{1,12} \\
& - 6590678814720000 p_{15,5} - 98576287436390400 a_0^4 p_{0,15} + 65553546994790400 \\
& a_0^3 a_1 p_{1,14} + 39094930332057600 a_0^3 a_2 p_{0,14} + 54977245779456000 a_0^2 a_1^2 p_{0,14} \\
& - 334410220488314880 a_0^3 p_{1,14} - 525582030061670400 a_0^2 a_1 p_{0,14} \\
& + 193415857542512640 a_0^2 a_2 p_{1,13} + 121488369691852800 a_0^2 a_3 p_{0,13} \\
& + 180975943847946240 a_0 a_1^2 p_{1,13} + 219388107093442560 a_0 a_1 a_2 p_{0,13} \\
& - 41287939873689600 a_0 a_1 a_3 p_{1,12} - 19769196016926720 a_0 a_2^2 p_{1,12} \\
& + 34346851880140800 a_1^3 p_{0,13} - 18459759062384640 a_1^2 a_2 p_{1,12} \\
& + 387819050159923200 a_0^2 p_{0,14} - 572391082402191360 a_0 a_1 p_{1,13} \\
& - 322079753927393280 a_0 a_2 p_{0,13} + 193344524171366400 a_0 a_3 p_{1,12} \\
& - 151886900912947200 a_1^2 p_{0,13} + 174014711073423360 a_1 a_2 p_{1,12} \\
& + 251466472435691520 a_0 p_{1,13} + 123471659966054400 a_1 p_{0,13} \\
& - 126591263754117120 a_2 p_{1,12} - 21749240088576000 p_{0,13} \\
& - 3515028701184000 p_{14,6} + 20640638785536000 a_0^4 p_{1,15} + 46867049349120000 \\
& a_0^3 a_1 p_{0,15} - 244703554295316480 a_0^3 p_{0,15} + 230294720734525440 a_0^2 a_1 p_{1,14} \\
& + 141571009027768320 a_0^2 a_2 p_{0,14} - 24343780995072000 a_0^2 a_3 p_{1,13} \\
& + 132962760528998400 a_0 a_1^2 p_{0,14} - 43551591874560000 a_0 a_1 a_2 p_{1,13} \\
& - 30128817438720000 a_0 a_1 a_3 p_{0,13} - 14461832370585600 a_0 a_2^2 p_{0,13}
\end{aligned}$$

$$\begin{aligned}
& -6779436580224000 a_1^3 p_{1,13} - 13557967847424000 a_1^2 a_2 p_{0,13} \\
& -397835972952606720 a_0^2 p_{1,14} - 431131401288806400 a_0 a_1 p_{0,14} \\
& + 224261805056163840 a_0 a_2 p_{1,13} + 144784205269401600 a_0 a_3 p_{0,13} \\
& + 105110433814579200 a_1^2 p_{1,13} + 131119800827904000 a_1 a_2 p_{0,13} \\
& - 46565041365964800 a_1 a_3 p_{1,12} - 22324494325432320 a_2^2 p_{1,12} \\
& + 194452129557504000 a_0 p_{0,14} - 168943146557875200 a_1 p_{1,13} \\
& - 97997665812480000 a_2 p_{0,13} + 73858292479641600 a_3 p_{1,12} \\
& + 50344978505472000 p_{1,13} - 2259661307904000 p_{13,7}, 17261301657600000 \\
& a_0^4 p_{0,16} + 112728811345920000 a_0^3 p_{1,15} + 197390830500864000 a_0^2 a_1 p_{0,15} \\
& - 29801180344320000 a_0^2 a_2 p_{1,14} - 20713561989120000 a_0^2 a_3 p_{0,14} \\
& - 27839280801024000 a_0 a_1^2 p_{1,14} - 37284411580416000 a_0 a_1 a_2 p_{0,14} \\
& - 5825689309440000 a_1^3 p_{0,14} - 348967027983974400 a_0^2 p_{0,15} \\
& + 311995534562611200 a_0 a_1 p_{1,14} + 196597707315609600 a_0 a_2 p_{0,14} \\
& - 64175077177344000 a_0 a_3 p_{1,13} + 7966754611200000 a_0 a_5 p_{1,12} \\
& + 92477423630592000 a_1^2 p_{0,14} - 57577438033920000 a_1 a_2 p_{1,13} \\
& - 40666661038080000 a_1 a_3 p_{0,13} - 19542345596928000 a_2^2 p_{0,13} \\
& + 6292701499392000 a_2 a_3 p_{1,12} - 273503828189491200 a_0 p_{1,14} \\
& - 152362371313152000 a_1 p_{0,14} + 100268760453120000 a_2 p_{1,13} \\
& + 66182003306496000 a_3 p_{0,13} + 46605514475520000 p_{0,14} \\
& - 1738201006080000 p_{12,8}, 112711471488000000 a_0^3 p_{0,16} - 44270237975040000 \\
& a_0^2 a_1 p_{1,15} - 29742550548480000 a_0^2 a_2 p_{0,15} - 27883641139200000 a_0 a_1^2 p_{0,15} \\
& + 267323243894784000 a_0^2 p_{1,15} + 319434268640256000 a_0 a_1 p_{0,15} \\
& - 92098626291302400 a_0 a_2 p_{1,14} - 65200643988480000 a_0 a_3 p_{0,14} \\
& + 7966754611200000 a_0 a_5 p_{0,13} - 43089968452608000 a_1^2 p_{1,14} \\
& - 58840863105024000 a_1 a_2 p_{0,14} + 8740150594560000 a_1 a_3 p_{1,13} \\
& + 4186167422976000 a_2^2 p_{1,13} + 6373403688960000 a_2 a_3 p_{0,13} \\
& - 286531572096000000 a_0 p_{0,15} + 163118740232448000 a_1 p_{1,14} \\
& + 104912846438400000 a_2 p_{0,14} - 49015716406272000 a_3 p_{1,13} \\
& + 11799246412800000 a_5 p_{1,12} - 86999934954240000 p_{1,14} \\
& - 1593350922240000 p_{11,9}, -27338728919040000 a_0^3 p_{1,16} - 51783904972800000 \\
& a_0^2 a_1 p_{0,16} + 319194748680192000 a_0^2 p_{0,16} - 160474637030400000 a_0 a_1 p_{1,15} \\
& - 109715247503769600 a_0 a_2 p_{0,15} + 15205809991680000 a_0 a_3 p_{1,14}
\end{aligned}$$

$$\begin{aligned}
& - 51508689813504000 a_1^2 p_{0,15} + 13610113877606400 a_1 a_2 p_{1,14} \\
& + 10356780994560000 a_1 a_3 p_{0,14} + 4971254877388800 a_2^2 p_{0,14} \\
& + 327006996535296000 a_0 p_{1,15} + 199291987851264000 a_1 p_{0,15} \\
& - 82647733122662400 a_2 p_{1,14} - 59410261886976000 a_3 p_{0,14} \\
& + 14079428149248000 a_5 p_{0,13} - 2182407929856000 a_6 p_{1,12} \\
& - 108746200442880000 p_{0,15} - 1738201006080000 p_{10,10}, -37493639479296000 \\
& a_0^3 p_{0,17} - 174738024786124800 a_0^2 p_{1,16} - 224522458288128000 a_0 a_1 p_{0,16} \\
& + 27818941435084800 a_0 a_2 p_{1,15} + 21090172207104000 a_0 a_3 p_{0,15} \\
& + 12997760148172800 a_1^2 p_{1,15} + 18981154986393600 a_1 a_2 p_{0,15} \\
& + 466969769570304000 a_0 p_{0,16} - 169619338964275200 a_1 p_{1,15} \\
& - 117703246793932800 a_2 p_{0,15} + 31387921044480000 a_3 p_{1,14} \\
& - 3483644516352000 a_5 p_{1,13} - 3012881743872000 a_6 p_{0,13} \\
& + 174856537445990400 p_{1,15} - 2259661307904000 p_{9,11}, -287998018250342400 \\
& a_0^2 p_{0,17} + 62809169104281600 a_0 a_1 p_{1,16} + 45695373115392000 a_0 a_2 p_{0,16} \\
& + 21419706147840000 a_1^2 p_{0,16} - 437041512017510400 a_0 p_{1,16} \\
& - 285046858736640000 a_1 p_{0,16} + 68199925918924800 a_2 p_{1,15} \\
& + 52286051930112000 a_3 p_{0,15} - 5711921639424000 a_5 p_{0,14} \\
& + 299875886069760000 p_{0,16} - 3515028701184000 p_{8,12}, 90491066265600000 \\
& a_0^2 p_{1,17} + 123026004541440000 a_0 a_1 p_{0,17} - 871978191372288000 a_0 p_{0,17} \\
& + 184256549148672000 a_1 p_{1,16} + 135579678474240000 a_2 p_{0,16} \\
& - 15849013340160000 a_3 p_{1,15} - 431720846548992000 p_{1,16} \\
& - 6590678814720000 p_{7,13}, 213412456857600000 a_0^2 p_{0,18} \\
& + 642329649561600000 a_0 p_{1,17} + 441889322434560000 a_1 p_{0,17} \\
& - 46699667030016000 a_2 p_{1,16} - 37661021798400000 a_3 p_{0,16} \\
& - 1054508610355200000 p_{0,17} - 15064408719360000 p_{6,14}, \\
& 1886566118621184000 a_0 p_{0,18} - 177132339191808000 a_1 p_{1,17} \\
& - 136583972388864000 a_2 p_{0,17} + 1393583343280128000 p_{1,17} \\
& - 42682491371520000 p_{5,15}, -909137066213376000 a_0 p_{1,18} \\
& - 653042117984256000 a_1 p_{0,18} + 5224336943874048000 p_{0,18} \\
& - 153656968937472000 p_{4,16}, -4379223614717952000 a_0 p_{0,19} \\
& - 6447190321668096000 p_{1,18} - 729870602452992000 p_{3,17}, \\
& -43792236147179520000 p_{0,19} - 4865804016353280000 p_{2,18}]]
\end{aligned}$$

```

> solve(%[-1], {p1, 12, seq(p_{k,m-k}, k=2..m)}) :
ss := subs(%[1..1], ss) union{b18=0, op(%)} :

```

Thus for the vector fields on the plane with  $v(0) = 0$ ,  $d_0 v(0) = D_x \otimes dy$ , i.e.

$v(x, y) = y \cdot D_x + x \cdot (x \cdot a(x) + y \cdot b(x)) \cdot D_y$ , and also with  $a(0) \neq 0$ ,  $b(0) \neq 0$ , there is precisely 1 new invariant in orders 2,3,4,5,7,8,10,11,13,14,16,17,19,... . Consequently the Poincare series is equal to:

$$\begin{aligned}
 & \text{> } \text{simplify} \left( z^3 + \sum_{i=0}^{\infty} z^{3i+2} + \sum_{i=1}^{\infty} z^{3i+1} \right) \\
 & \qquad \qquad \qquad \frac{z^2 (z^4 - z^2 - z - 1)}{z^3 - 1} \qquad \qquad \qquad (31)
 \end{aligned}$$

$$\begin{aligned}
 & \text{> } \text{series} \left( \frac{z^2 (z^4 - z^2 - z - 1)}{z^3 - 1}, z=0, 20 \right) \\
 & \qquad \qquad \qquad z^2 + z^3 + z^4 + z^5 + z^7 + z^8 + z^{10} + z^{11} + z^{13} + z^{14} + z^{16} + z^{17} + z^{19} + O(z^{20}) \qquad (32)
 \end{aligned}$$
